# Supplementary material for: Learning Dynamics of Deep Linear Networks Beyond the Edge of Stability
Source: arXiv:2502.20531 source file (2025-02-27)
Supplement: Supplementary file 1 [file appendix.tex]

\appendix
\onecolumn
\par\noindent\rule{\textwidth}{1pt}
\begin{center}
{\Large \bf Appendix}
\end{center}
\vspace{-0.1in}
\par\noindent\rule{\textwidth}{1pt}
%\section{Appendix}

\section{Experimental Details}
\label{sec:exp_details}

\section{Additional Results}
\label{sec:additional_exp}

This section is organized as follows: Section~\ref{sec:init_outside_svs} presents an additional example of an initialization that empirically converges to the SVS set; Section~\ref{sec:more_balancing} presents more experimental results on the balancing result in Lemma~\ref{lemma:balancing}; Section~\ref{sec:more_oscillations} shows additional results on oscillations in deep linear networks and catapults in deep nonlinear networks; and finally Section~\ref{sec:lora_exp}  investigates the use of large learning rates in low-rank adaptation and how catapults may improve generalization in terms of Pearson correlation.

\subsection{Initialization Outside Singular Vector Invariant Set}
\label{sec:init_outside_svs}

In this section, we present an initialization example that is (initially) outside the singular vector stationary set. We consider the following initialization:
\begin{align}
    \mbf{W}_L(0) = \mbf{0}, \quad \quad\quad \mbf{W}_\ell(0) = \alpha \mbf{P}_\ell, \quad \forall \ell \in [L-1],
\end{align}
where $\mbf{P}_\ell \in \mbb{R}^{d\times d}$ is an orthogonal matrix. Note that here for $\ell>1$, the singular vectors do not align and lies outside the SVS set we defined in Proposition~\ref{prop:one_zero_svs_set}. 
We consider the deep matrix factorization problem with a target matrix $\mbf{M}_\star \in \mbb{R}^{d\times d}$, where $d=100$, $r=5$, and $\alpha = 0.01$. We empirically obtain that the decomposition after convergence admits the form:
    \begin{align}
        \mbf{W}_L(t) &= 
        \mbf{U}^\star
        \begin{bmatrix}
            \mbf{\Sigma}_L(t) & \mbf{0} \\
            \mbf{0} & \mbf{0}
        \end{bmatrix} \left[\left(\prod_{i=L-1}^1{\mbf{P}_{i}}\right)\mbf{V^\star}\right]^{\top}, \\
        \mbf{W}_{\ell}(t) &= \left[\left(\prod_{i=\ell}^1{\mbf{P}_{i}}\right)\mbf{V^\star}\right]
        \begin{bmatrix}
            \mbf{\Sigma}_{\ell}(t) & \mbf{0} \\
            \mbf{0} & \alpha\mbf{I}_{d-r}
        \end{bmatrix} \left[\left(\prod_{i=\ell-1}^1{\mbf{P}_{i}}\right)\mbf{V^\star}\right]^{\top},
        \quad \forall \ell \in [2, L-1], \\
        \mbf{W}_{1}(t) &= \mbf{P}_{1}\mbf{V}^{\star} \begin{bmatrix}
            \mbf{\Sigma}_{1}(t) & \mbf{0} \\
            \mbf{0} & \alpha\mbf{I}_{d-r}
        \end{bmatrix} \mbf{V}^{\star\top},
    \end{align} 
    where  
    $\mbf{W}_L(0) = \mbf{0}$ and $\mbf{W}_{\ell}(0) = \alpha \mbf{P}_{l}$, $\forall\ell \in [L-1]$.
    The decomposition after convergence lies in the SVS set as the singular vectors now align with each other. This demonstrates an example where even when the initialization is made outside the SVS set, GD aligns the singular vectors such that after certain iterations it lies in the SVS set.

\begin{figure}[h!]
    \centering
     \begin{subfigure}[b]{0.495\textwidth}
         \centering
        \includegraphics[width=\textwidth]{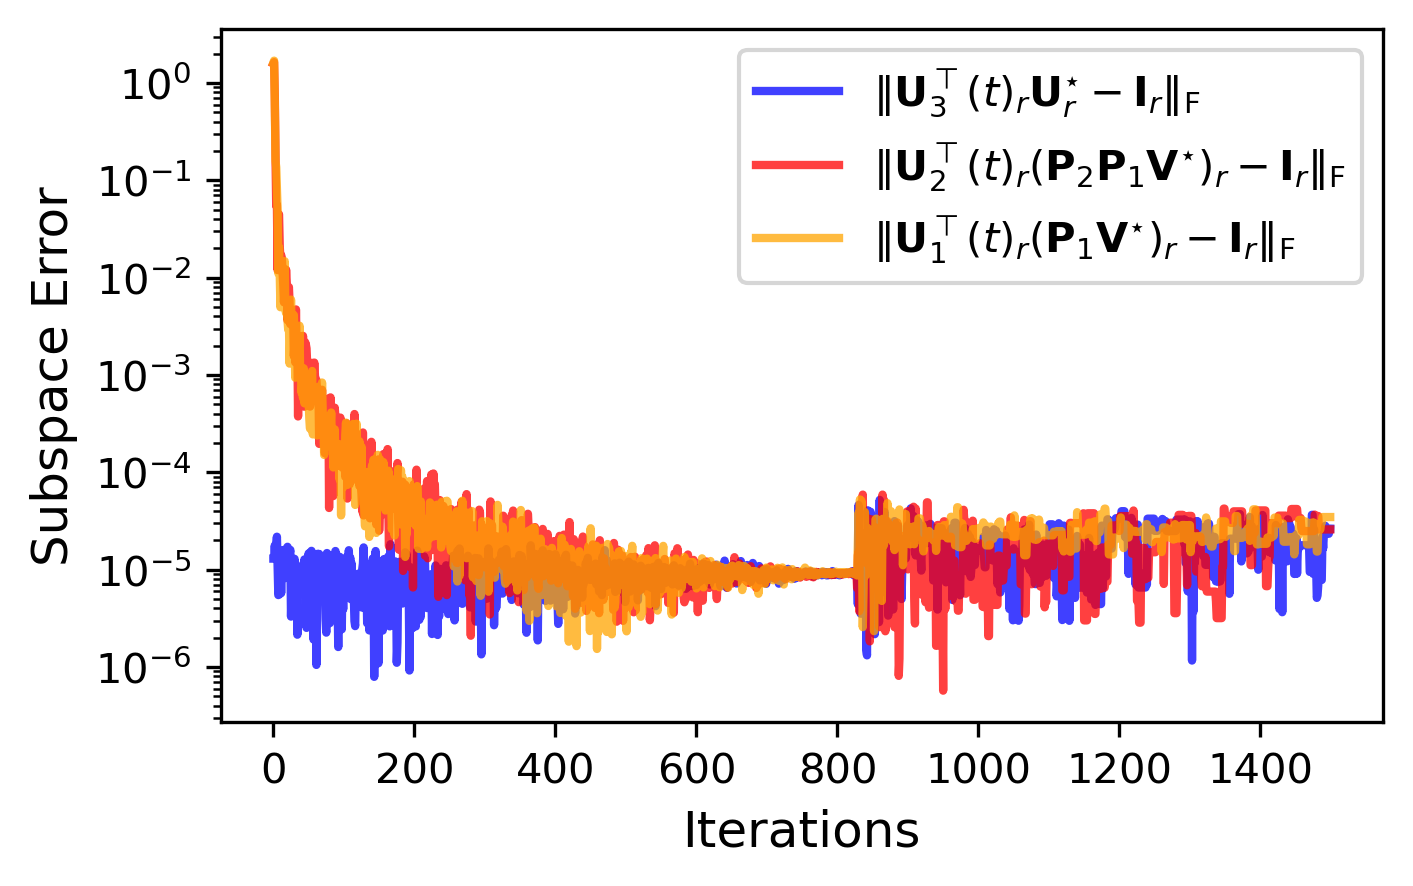}
         \caption*{Left Singular Vectors}
     \end{subfigure}
         \begin{subfigure}[b]{0.495\textwidth}
         \centering
        \includegraphics[width=\textwidth]{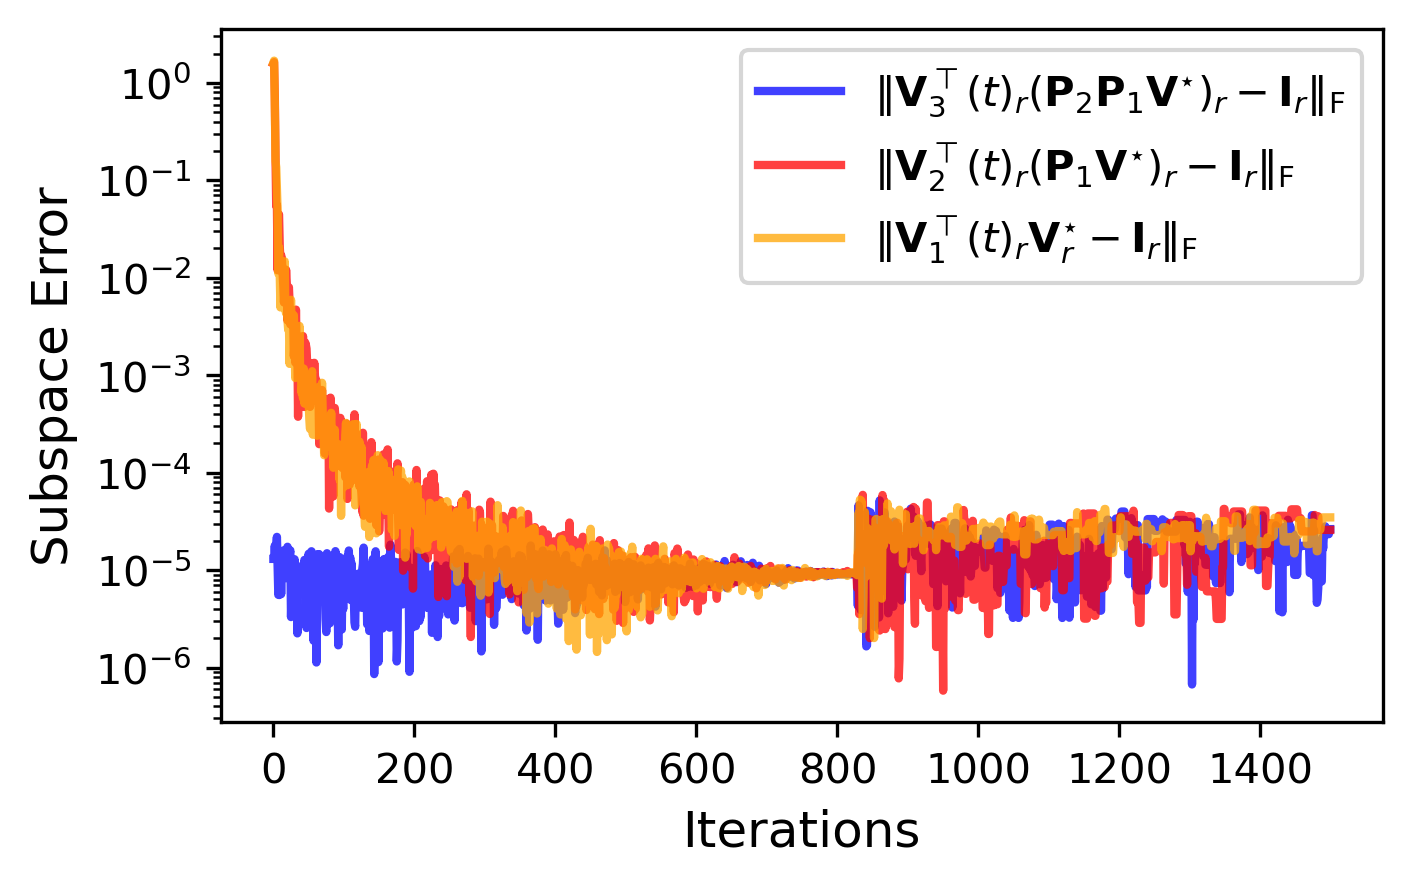}
         \caption*{Right Singular Vectors}
     \end{subfigure}
    \caption{Empirical verification of the decomposition for initialization with orthogonal matrices (lying outside SVS set) in that after some GD iterations, the singular vectors of the intermediate matrices align to lie within SVS set, displaying singular vector invariance.}
    \label{fig:verify_conj}
\end{figure}

\subsection{Balancing of Singular Values}
\label{sec:more_balancing}

In this section, we present additional experimental results on Lemma~\ref{lemma:balancing} and how close the iterates become for different initialization scales. To this end, we consider the same setup from the previous section, where we have a target matrix $\mbf{M}_\star \in \mbb{R}^{d\times d}$, where $d=100$, $r=5$, and varying initialization $\alpha$.  In Figure~\ref{fig:assumption}, we observe that for larger values of $\alpha$, the balancing quickly occurs, whereas for smaller values of $\alpha$, the balancing is almost immediate. This is to also highlight that our bound on $\alpha$ in Lemma~\ref{lemma:balancing} may be an artifact of our analysis, and can choose larger values of $\alpha$ in practice.

\begin{figure}[h!]
    \centering
     \begin{subfigure}[b]{0.315\textwidth}
         \centering
        \includegraphics[width=\textwidth]{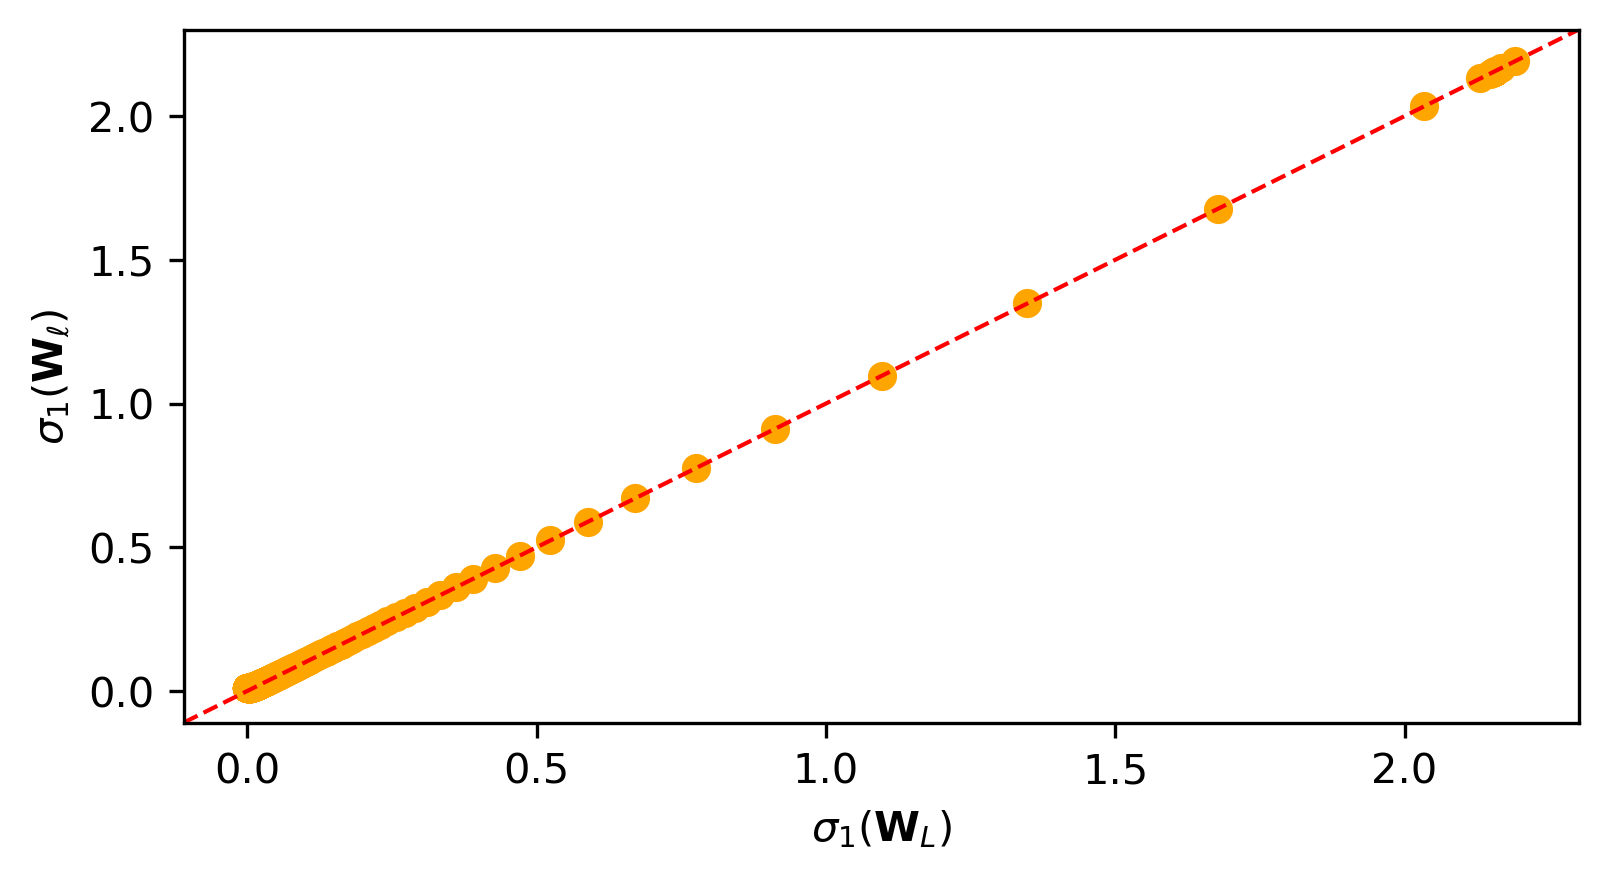}
         \caption*{$\alpha = 0.01$}
     \end{subfigure}
     \begin{subfigure}[b]{0.315\textwidth}
         \centering
        \includegraphics[width=\textwidth]{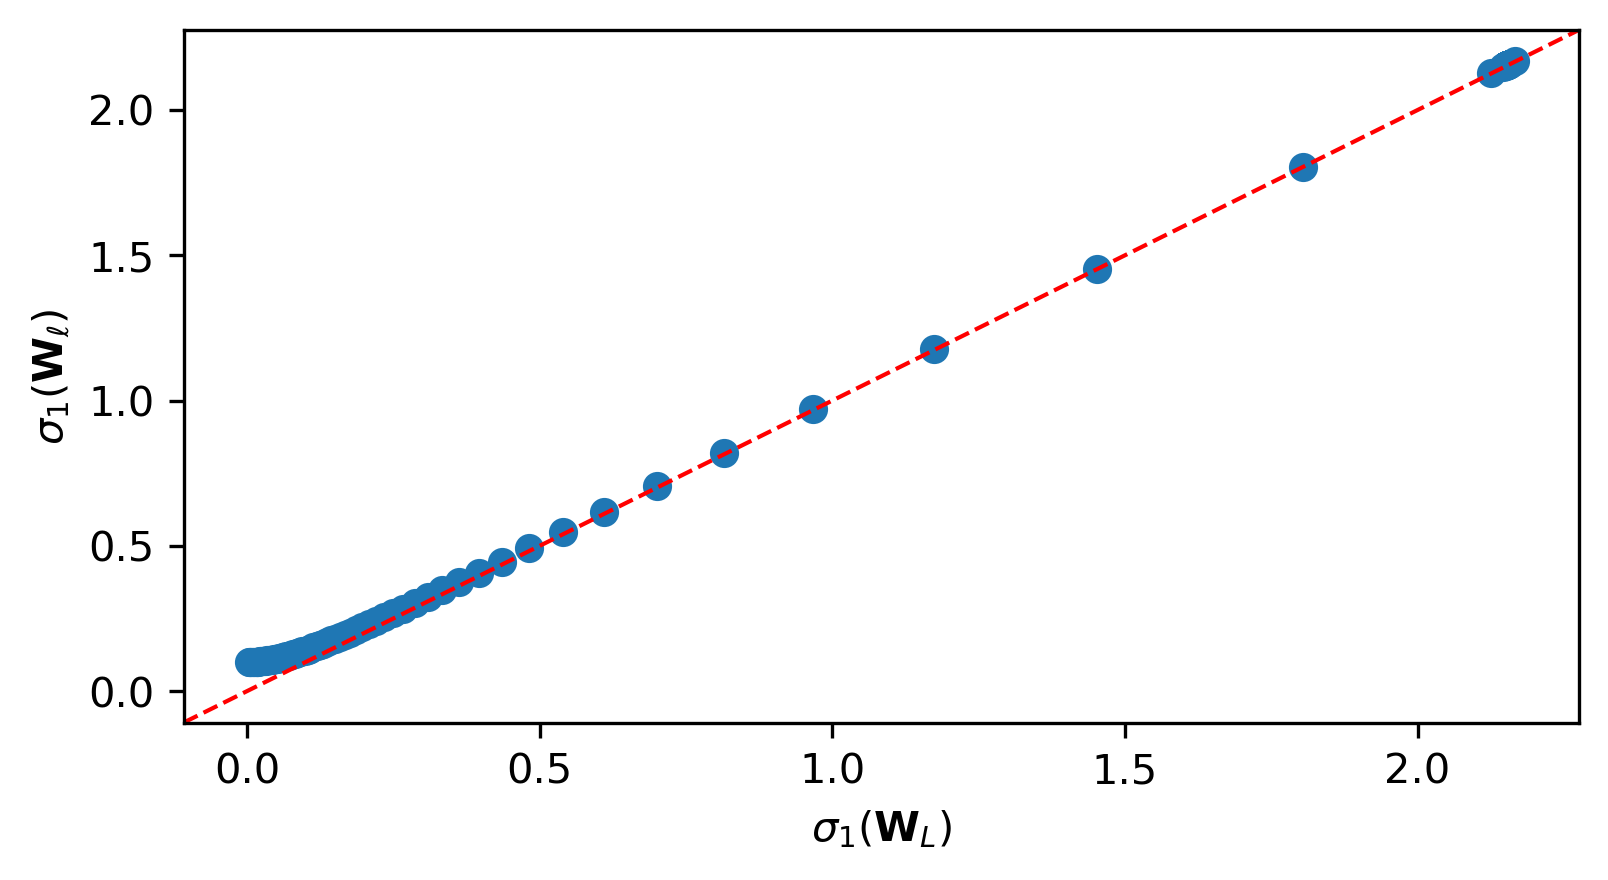}
         \caption*{$\alpha = 0.10$}
     \end{subfigure}
         \begin{subfigure}[b]{0.315\textwidth}
         \centering
        \includegraphics[width=\textwidth]{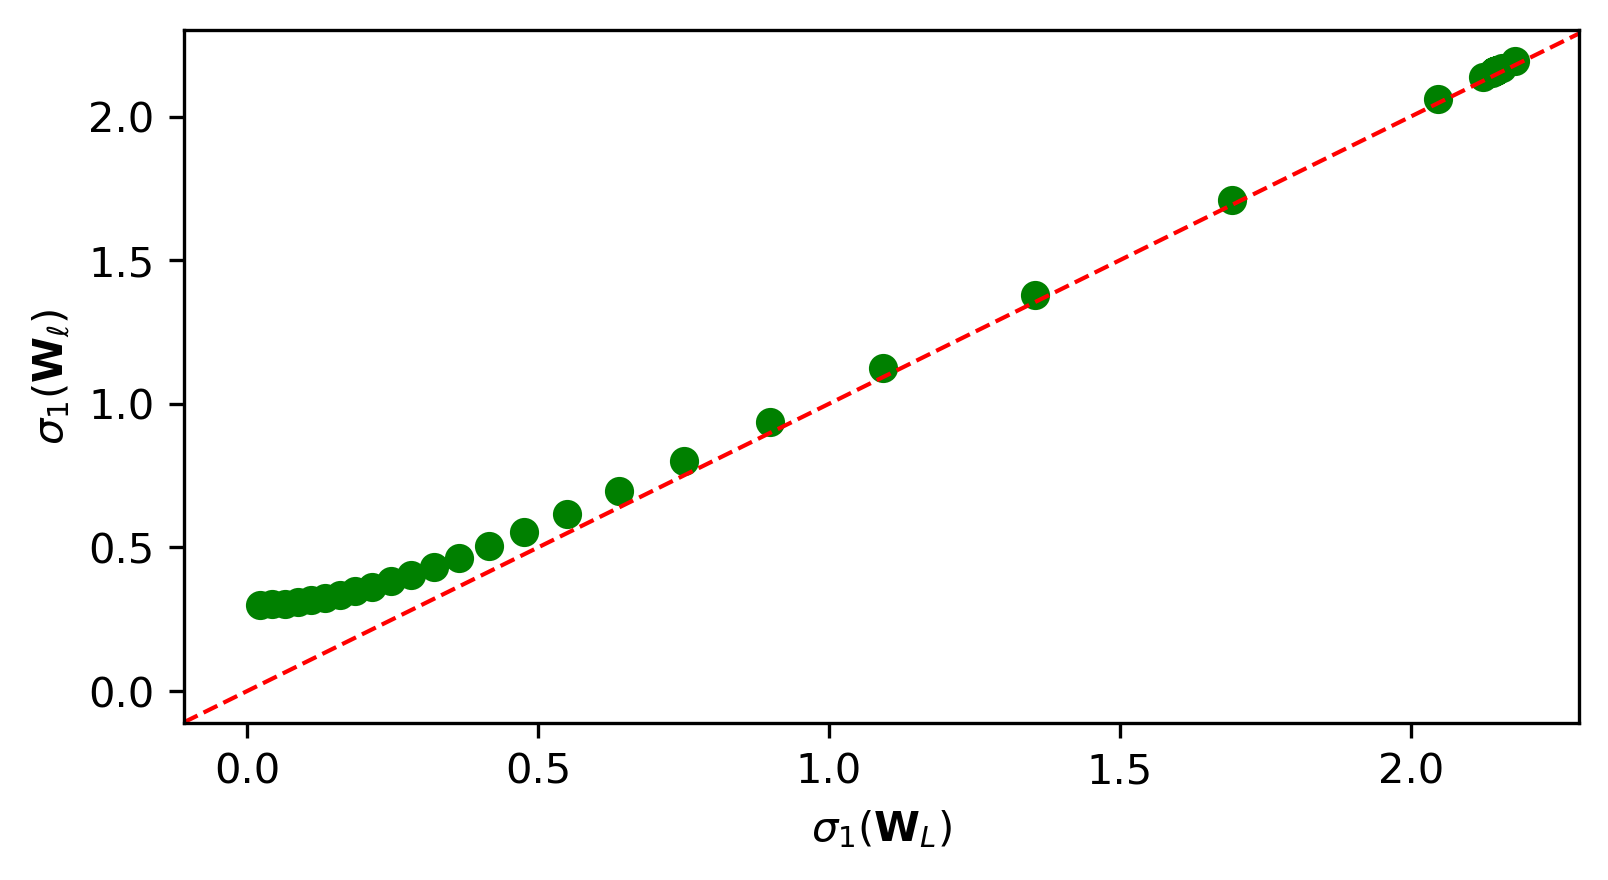}
         \caption*{$\alpha = 0.30$}
     \end{subfigure}
    \caption{Observing the balancedness between the singular value initialized to $0$ and a singular value initialized to $\alpha$. The scattered points are successive GD iterations (going left to right). The initial gap between the two values is larger for a larger $\alpha$, but quickly gets closer over more GD iterations.}
    \label{fig:assumption}
\end{figure}

\subsection{Additional Results on Periodic Oscillations}
\label{sec:more_oscillations}

%In this section, we present additional experiments on oscillation and catapults in both deep linear and nonlinear networks to supplement the results in the main paper. First, we consider a 3-layer MLP without bias terms for the weights, with each hidden layer consisting of 1000 units. The network is trained using MSE loss with a learning rate of $\eta = 4$, along with random weights scaled by $\alpha = 0.01$ and full-batch gradient descent on a 5K subset of the MNIST dataset, following~\cite{cohen2021gradient}. The motivation for omitting bias terms comes from the findings of~\cite{zhang2024when}, where they provably show that a ReLU network without bias terms behaves similarly to a linear network. With this in mind, we aimed to investigate how oscillations manifest in comparison to deep linear networks (DLNs). In Figure~\ref{fig:mlp_bias_free}, we plot the training loss, top-5 singular values, and sharpness throughout training. Interestingly, despite the non-convexity of the loss landscape, the oscillations appear to be almost periodic across all three plots. It would be of great interest to theoretically study the behavior of EOS for this network architecture and determine whether our analyses extend to this case as well.

In this section, we present additional results to to corroborate our theory in Theorem~\ref{thm:align_thm}. We consider modeling rank-3 target matrix with singular values $\sigma_{\star, i} = \{10, 9, 8\}$ with a 3-layer DLN with initialization scale $\alpha = 0.1$. By computing the sharpness under these settings, notice that $2 / \lambda_1 = L\sigma_{\star, 1}^{2 - \frac{2}{L}} \approx 0.01547$ and $2/\lambda_2 \approx 0.01657$. In Figure~\ref{fig:progressive_eta_dln}, we use learning rates near these values, and plot the oscillations in the singular values. Here, we can see that the oscillations follow exactly our theory.

\begin{figure}[ht]
    \centering
    \captionsetup{justification=centering}
    % Specify the filename for each figure
    \begin{subfigure}[b]{0.24\textwidth}
        \centering
        \includegraphics[width=\linewidth]{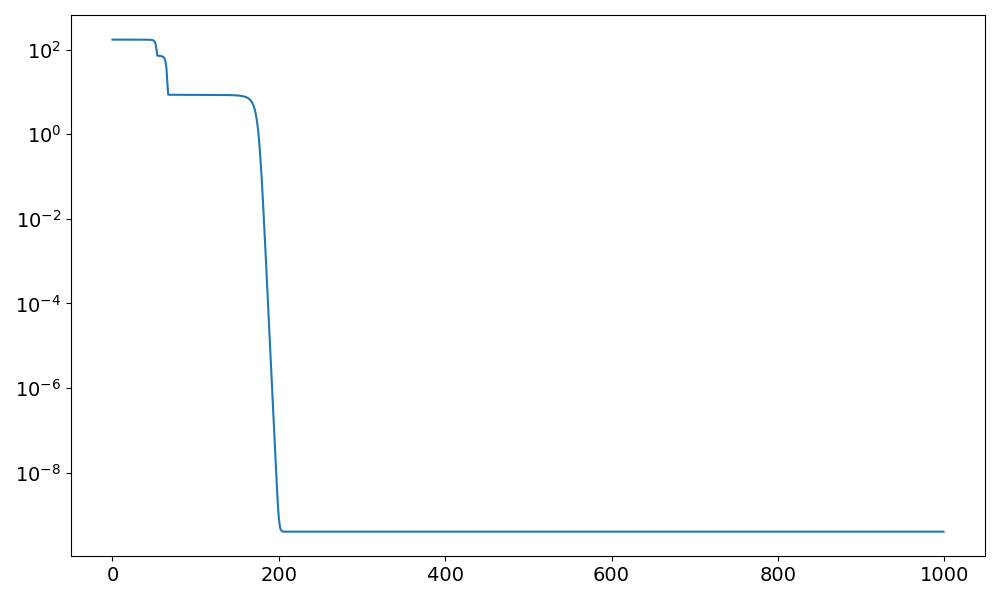}
        \caption*{\footnotesize Train Loss ($\eta = 0.015$) }
        \label{fig:1}
    \end{subfigure}\hfill
    \begin{subfigure}[b]{0.24\textwidth}
        \centering
        \includegraphics[width=\linewidth]{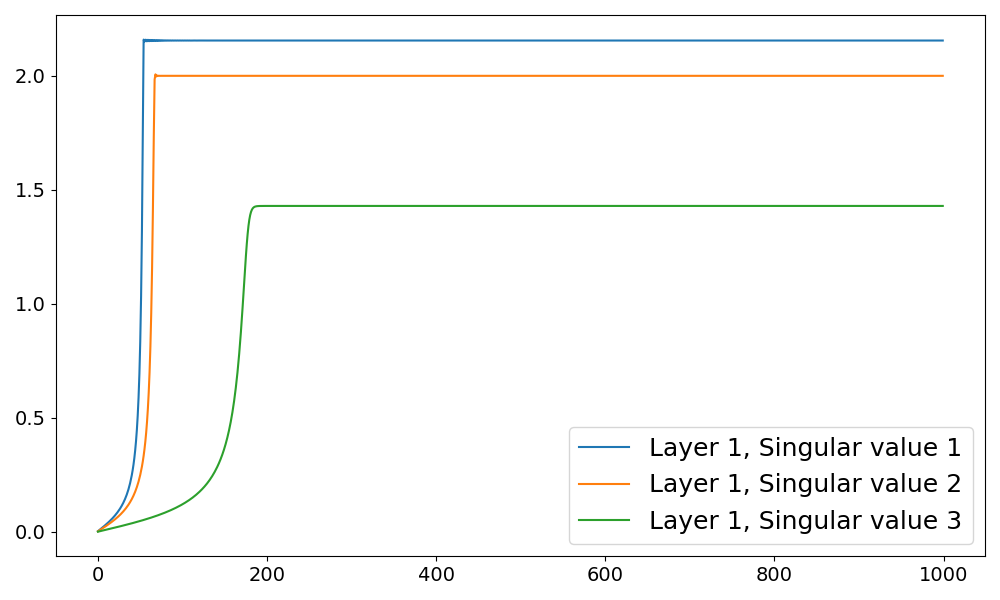}
        \caption*{\footnotesize Layer 1 $\sigma_i$ ($\eta = 0.015$)}
        \label{fig:2}
    \end{subfigure}\hfill
    \begin{subfigure}[b]{0.24\textwidth}
        \centering
        \includegraphics[width=\linewidth]{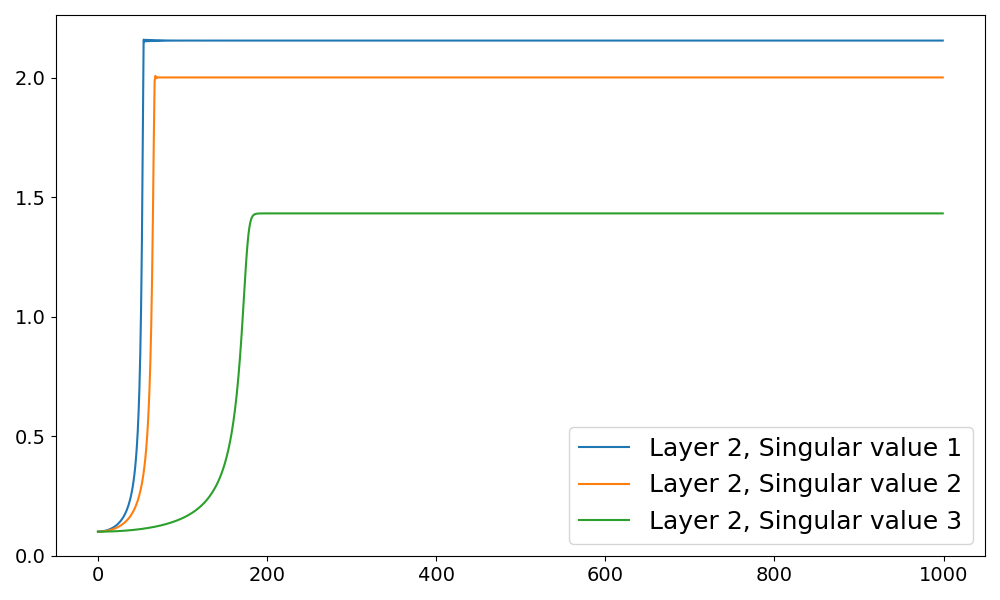}
        \caption*{\footnotesize Layer 2 $\sigma_i$ ($\eta = 0.015$)}
        \label{fig:3}
    \end{subfigure}\hfill
    \begin{subfigure}[b]{0.24\textwidth}
        \centering
        \includegraphics[width=\linewidth]{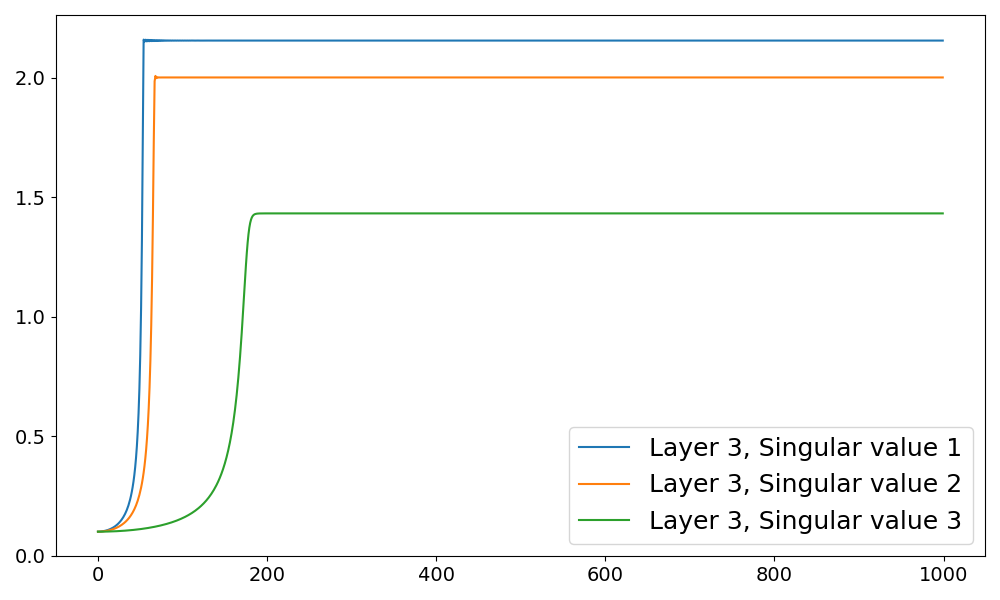}
        \caption*{\footnotesize Layer 3 $\sigma_i$ ($\eta = 0.015$)}
        \label{fig:4}
    \end{subfigure}
    \begin{subfigure}[b]{0.24\textwidth}
        \centering
        \includegraphics[width=\linewidth]{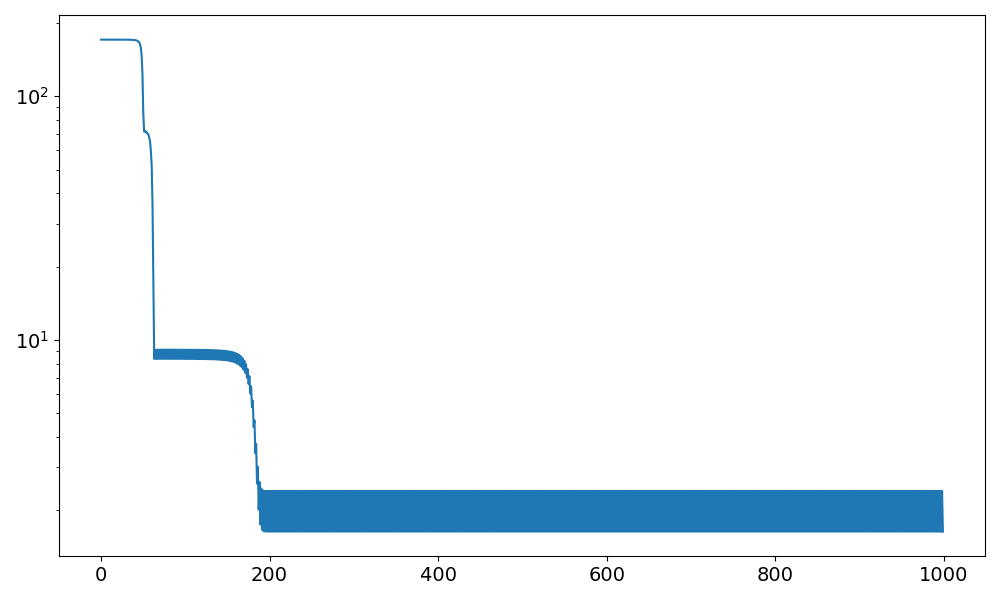}
        \caption*{\footnotesize Train Loss ($\eta = 0.016$) }
        \label{fig:1}
    \end{subfigure}\hfill
    \begin{subfigure}[b]{0.24\textwidth}
        \centering
        \includegraphics[width=\linewidth]{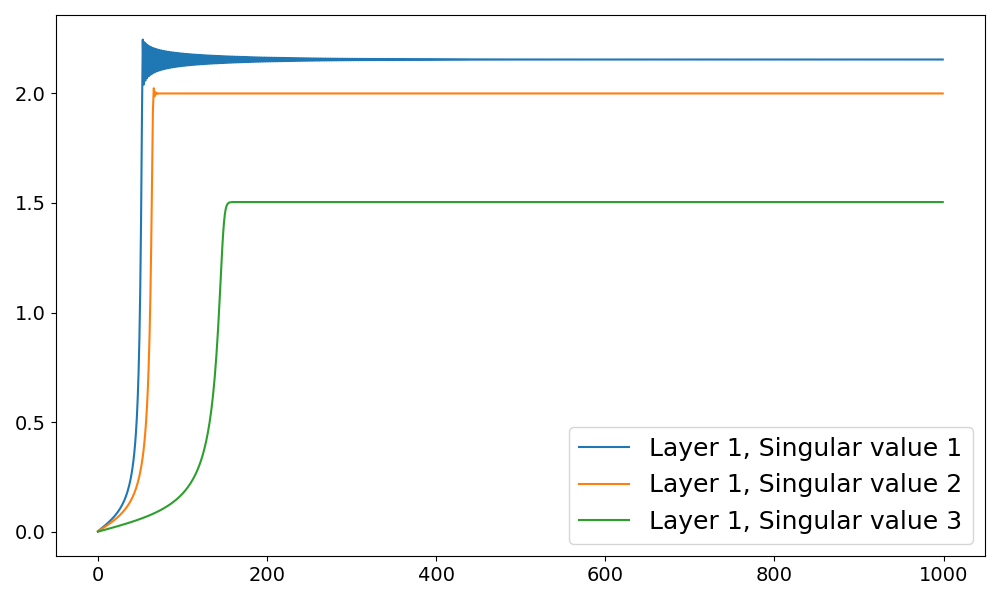}
        \caption*{\footnotesize Layer 1 $\sigma_i$ ($\eta = 0.0154$)}
        \label{fig:2}
    \end{subfigure}\hfill
    \begin{subfigure}[b]{0.24\textwidth}
        \centering
        \includegraphics[width=\linewidth]{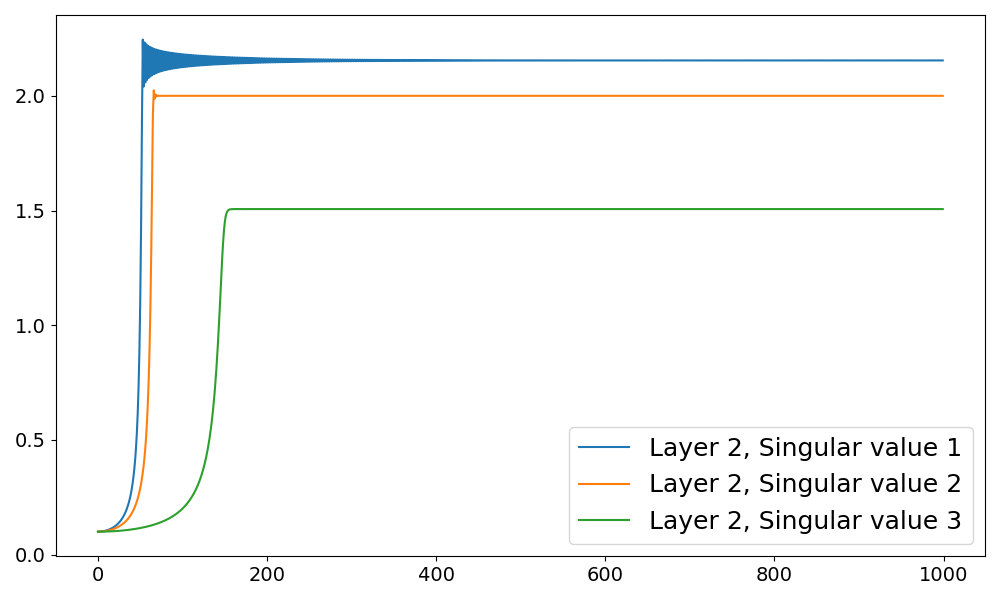}
        \caption*{\footnotesize Layer 2 $\sigma_i$ ($\eta = 0.0154$)}
        \label{fig:3}
    \end{subfigure}\hfill
    \begin{subfigure}[b]{0.24\textwidth}
        \centering
        \includegraphics[width=\linewidth]{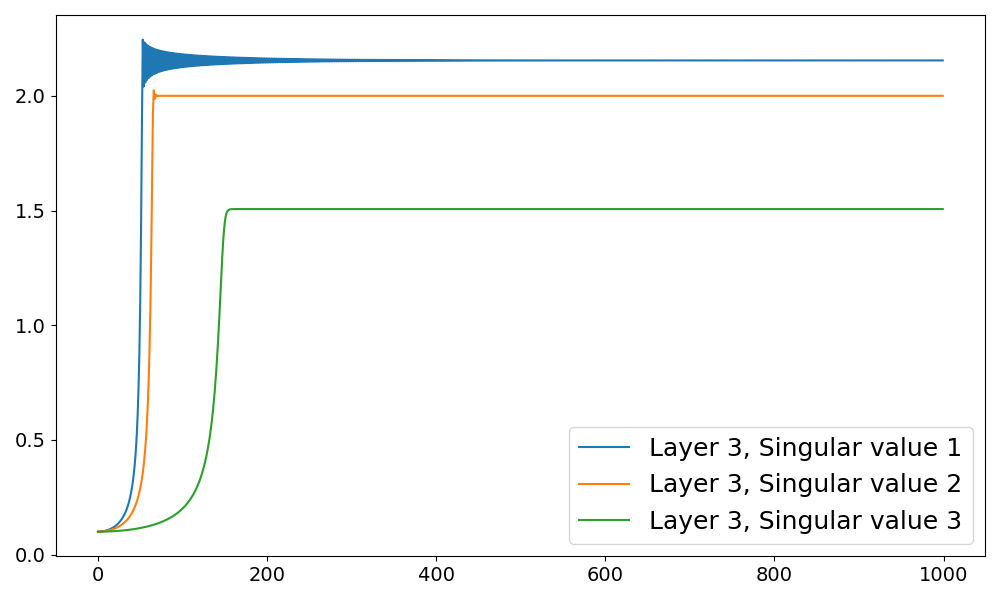}
        \caption*{\footnotesize Layer 3 $\sigma_i$ ($\eta = 0.0154$)}
        \label{fig:4}
    \end{subfigure}
        
    \begin{subfigure}[b]{0.24\textwidth}
        \centering
        \includegraphics[width=\linewidth]{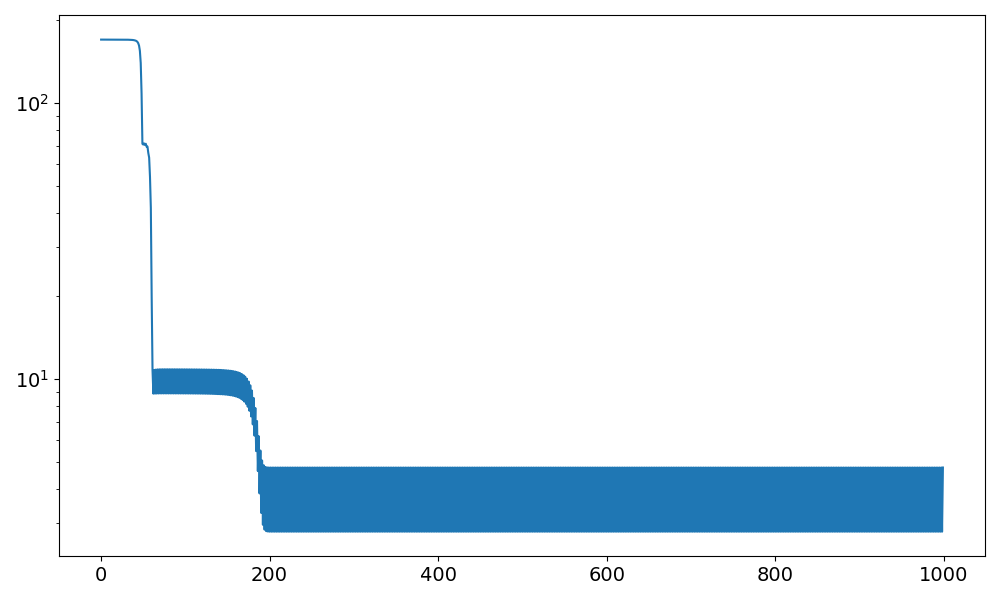}
        \caption*{\footnotesize Train Loss ($\eta = 0.0165$) }
        \label{fig:1}
    \end{subfigure}\hfill
    \begin{subfigure}[b]{0.24\textwidth}
        \centering
        \includegraphics[width=\linewidth]{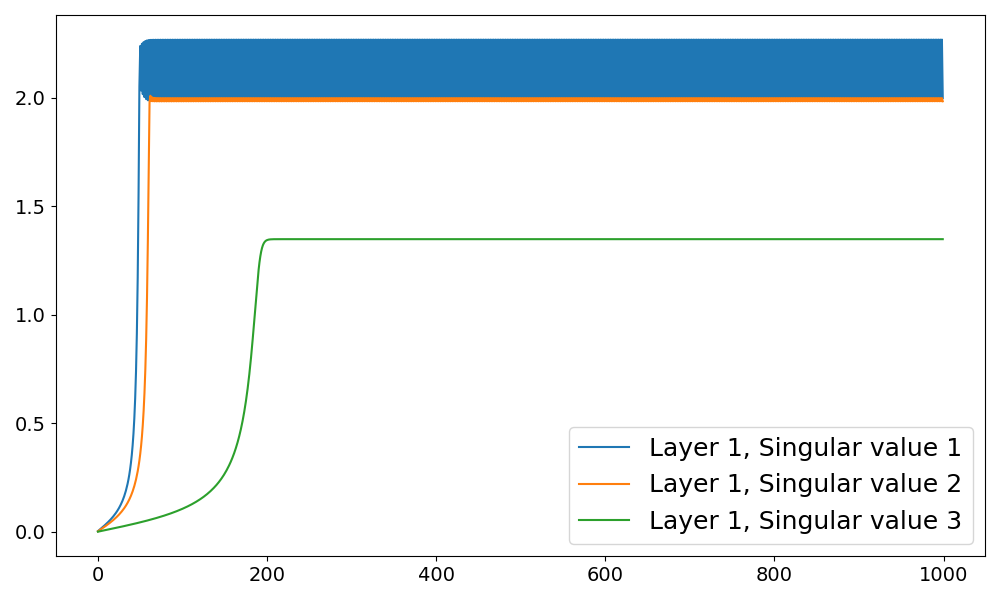}
        \caption*{\footnotesize Layer 1 $\sigma_i$ ($\eta = 0.0165$)}
        \label{fig:2}
    \end{subfigure}\hfill
    \begin{subfigure}[b]{0.24\textwidth}
        \centering
        \includegraphics[width=\linewidth]{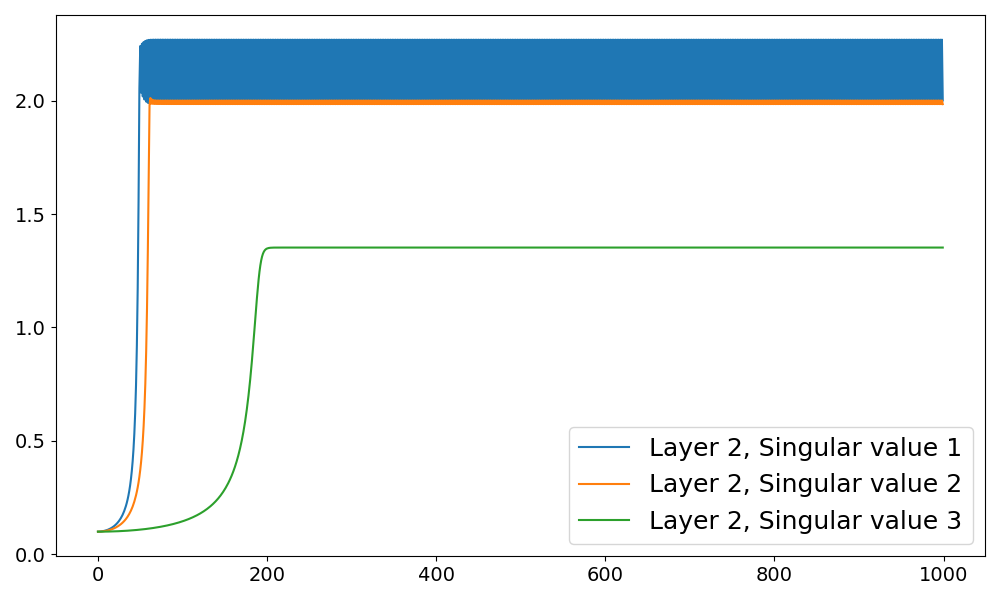}
        \caption*{\footnotesize Layer 2 $\sigma_i$ ($\eta = 0.0165$)}
        \label{fig:3}
    \end{subfigure}\hfill
    \begin{subfigure}[b]{0.24\textwidth}
        \centering
        \includegraphics[width=\linewidth]{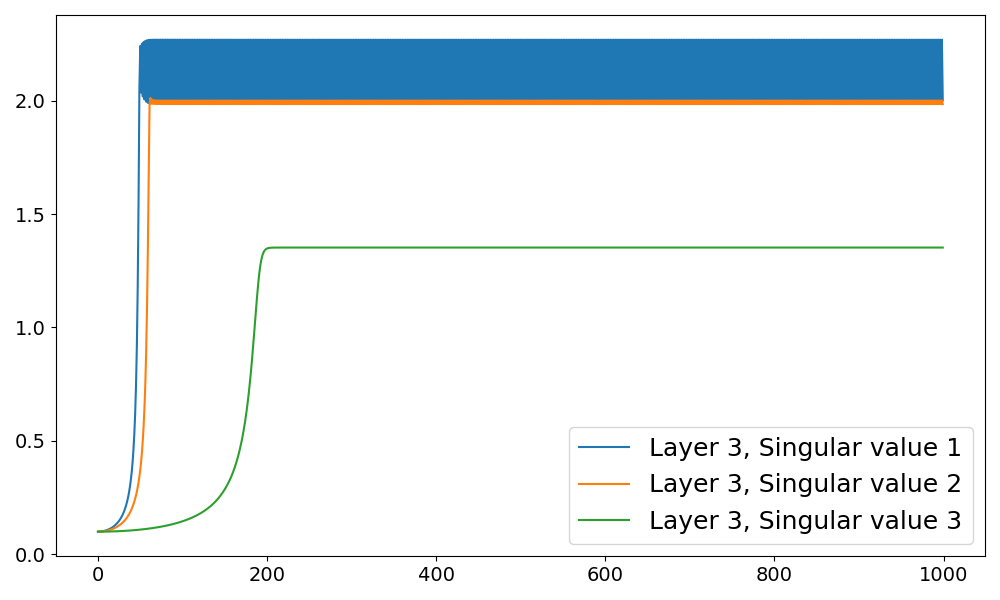}
        \caption*{\footnotesize Layer 3 $\sigma_i$ ($\eta = 0.0165$)}
        \label{fig:4}
    \end{subfigure}
    \begin{subfigure}[b]{0.24\textwidth}
        \centering
        \includegraphics[width=\linewidth]{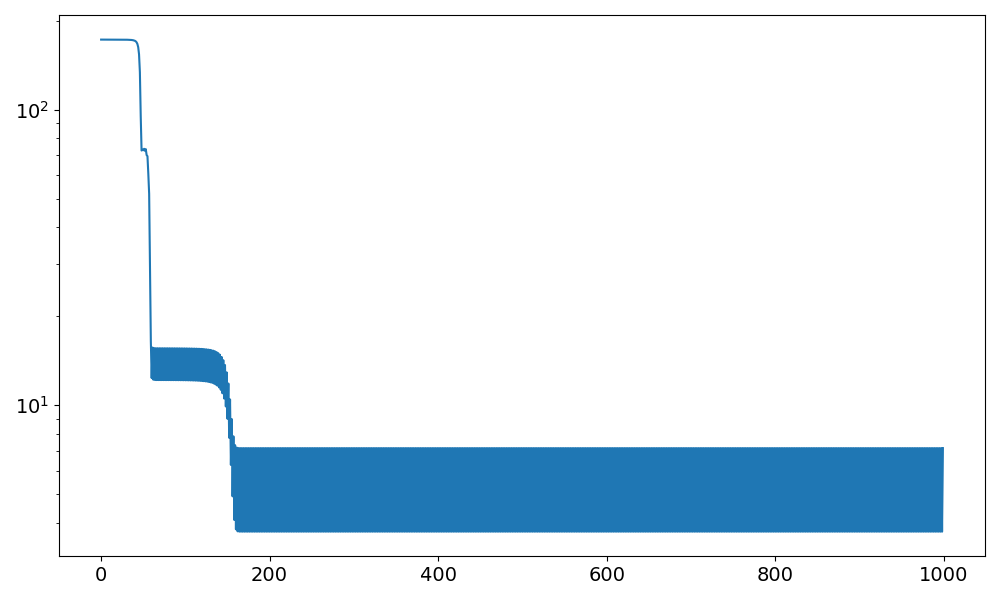}
        \caption*{\footnotesize Train Loss ($\eta = 0.017$) }
        \label{fig:1}
    \end{subfigure}\hfill
    \begin{subfigure}[b]{0.24\textwidth}
        \centering
        \includegraphics[width=\linewidth]{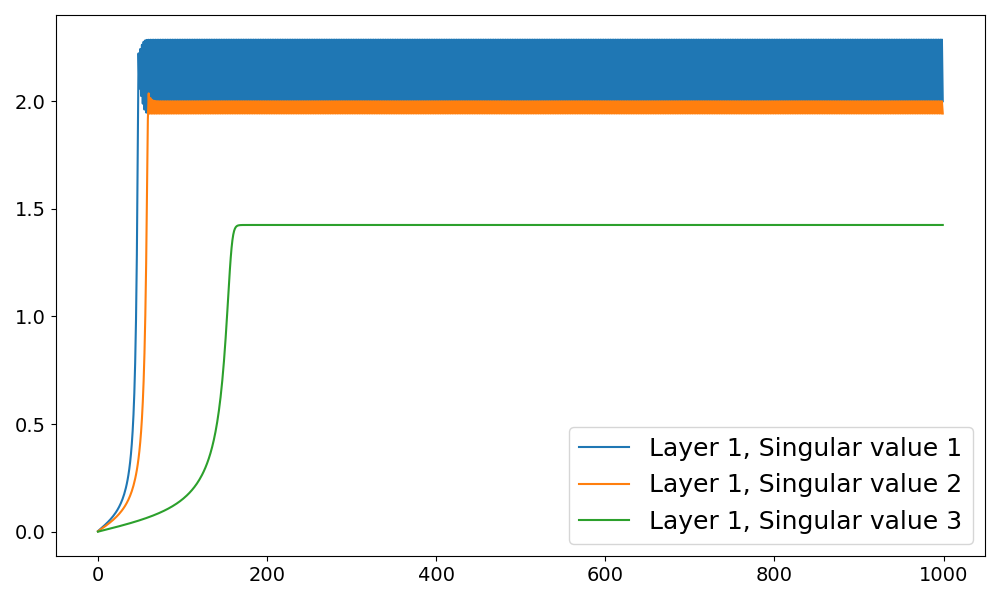}
        \caption*{\footnotesize Layer 1 $\sigma_i$ ($\eta = 0.017$)}
        \label{fig:2}
    \end{subfigure}\hfill
    \begin{subfigure}[b]{0.24\textwidth}
        \centering
        \includegraphics[width=\linewidth]{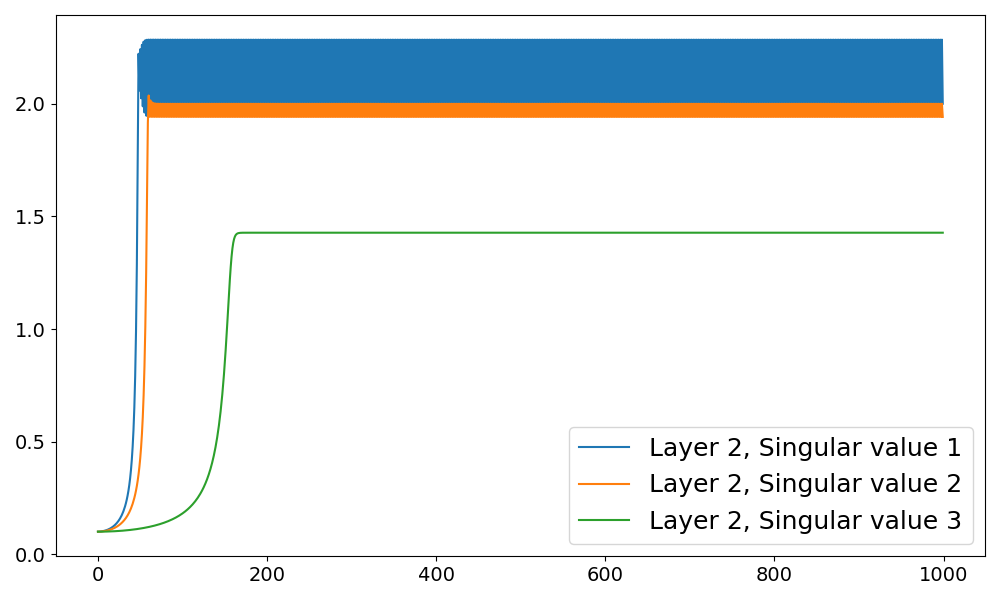}
        \caption*{\footnotesize Layer 2 $\sigma_i$ ($\eta = 0.017$)}
        \label{fig:3}
    \end{subfigure}\hfill
    \begin{subfigure}[b]{0.24\textwidth}
        \centering
        \includegraphics[width=\linewidth]{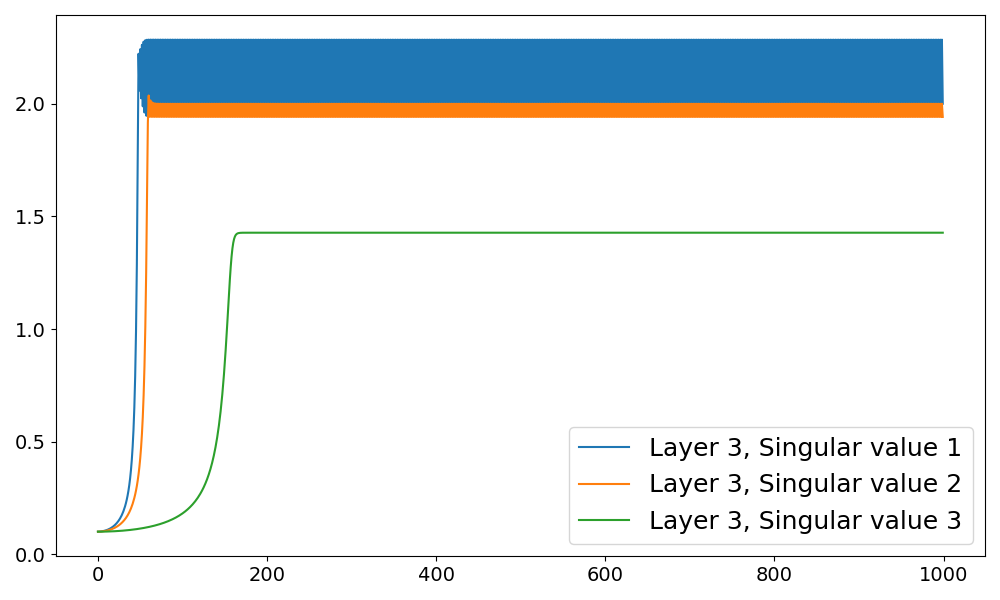}
        \caption*{\footnotesize Layer 3 $\sigma_i$ ($\eta = 0.017$)}
        \label{fig:4}
    \end{subfigure}

         % Adds space between the rows
    \begin{subfigure}[b]{0.24\textwidth}
        \centering
        \includegraphics[width=\linewidth]{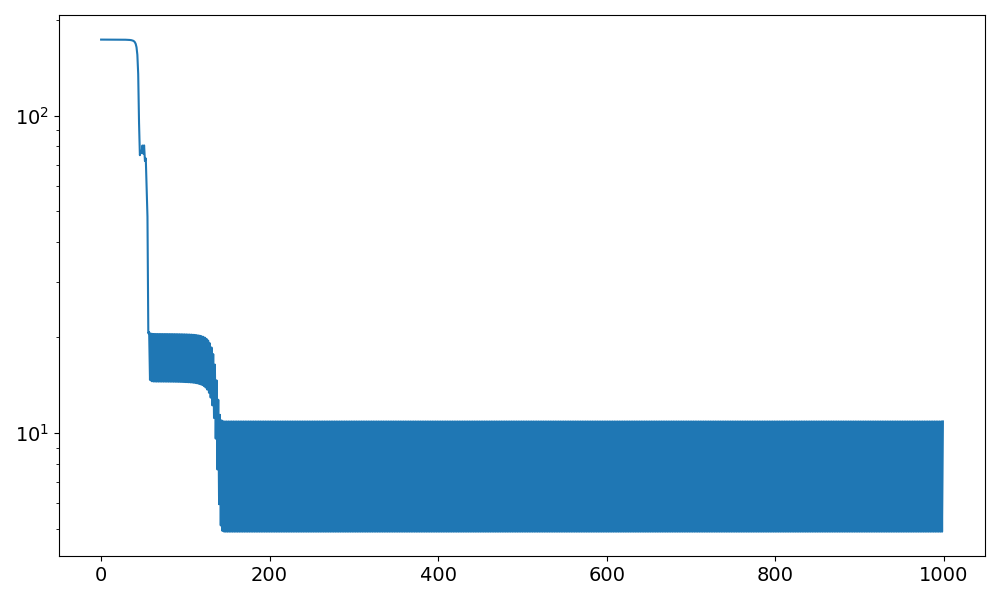}
        \caption*{\footnotesize Train Loss ($\eta = 0.0178$) }
        \label{fig:1}
    \end{subfigure}\hfill
    \begin{subfigure}[b]{0.24\textwidth}
        \centering
        \includegraphics[width=\linewidth]{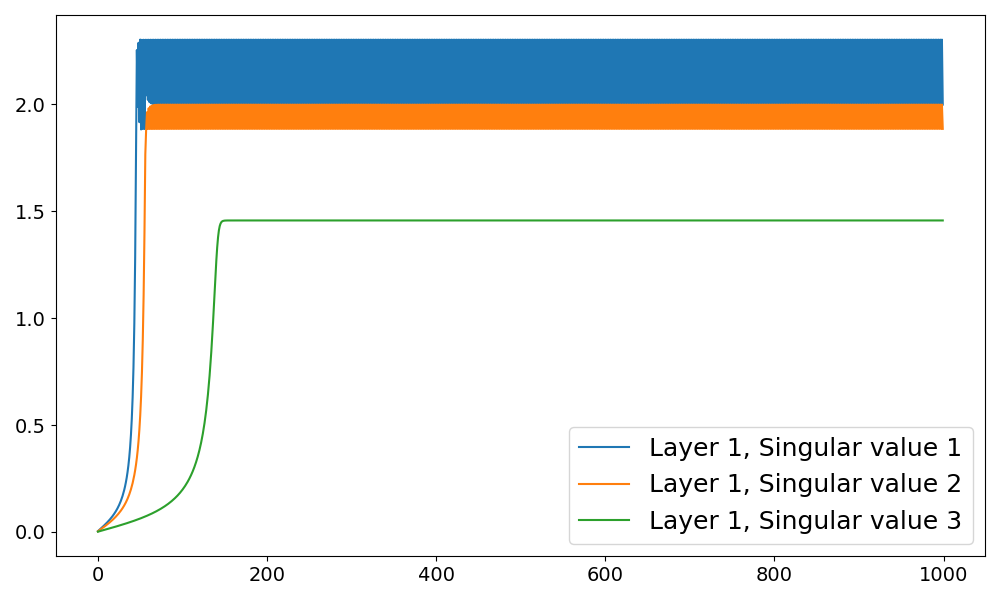}
        \caption*{\footnotesize Layer 1 $\sigma_i$ ($\eta = 0.0178$)}
        \label{fig:2}
    \end{subfigure}\hfill
    \begin{subfigure}[b]{0.24\textwidth}
        \centering
        \includegraphics[width=\linewidth]{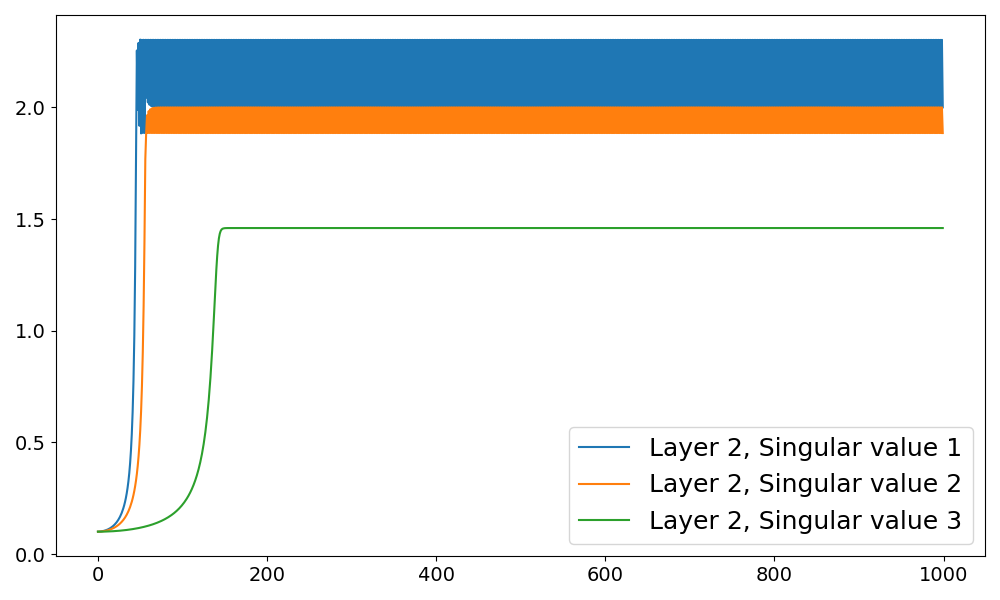}
        \caption*{\footnotesize Layer 2 $\sigma_i$ ($\eta = 0.0178$)}
        \label{fig:3}
    \end{subfigure}\hfill
    \begin{subfigure}[b]{0.24\textwidth}
        \centering
        \includegraphics[width=\linewidth]{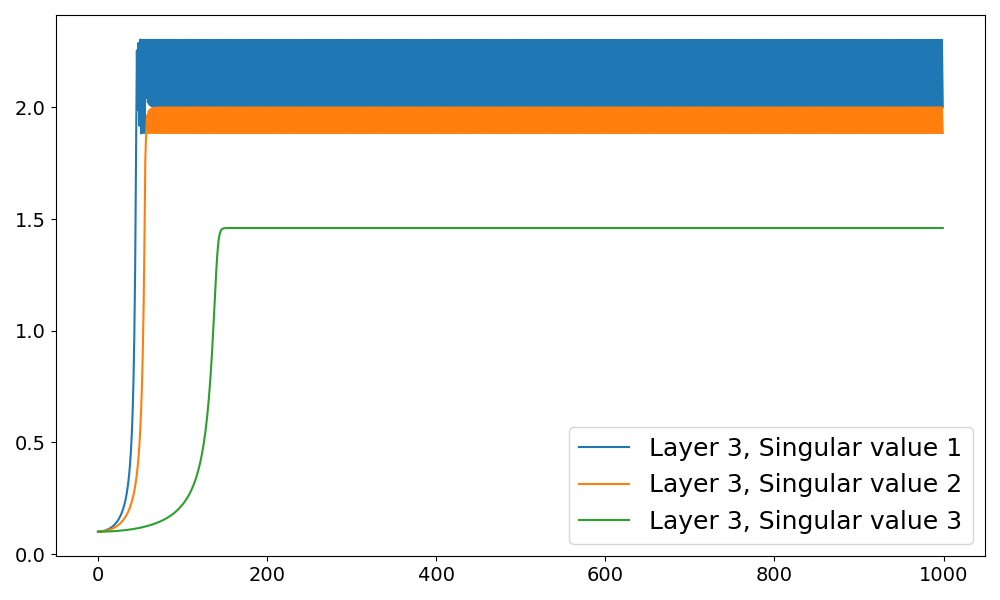}
        \caption*{\footnotesize Layer 3 $\sigma_i$ ($\eta = 0.0178$)}
        \label{fig:4}
    \end{subfigure}

    \begin{subfigure}[b]{0.24\textwidth}
        \centering
        \includegraphics[width=\linewidth]{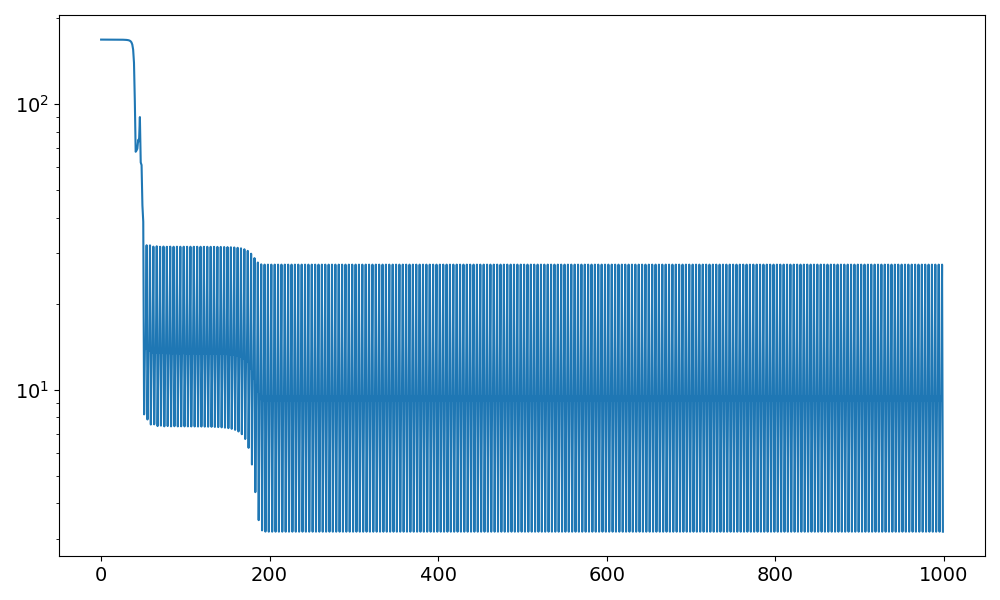}
        \caption*{\footnotesize Train Loss ($\eta = 0.02$) }
        \label{fig:1}
    \end{subfigure}\hfill
    \begin{subfigure}[b]{0.24\textwidth}
        \centering
        \includegraphics[width=\linewidth]{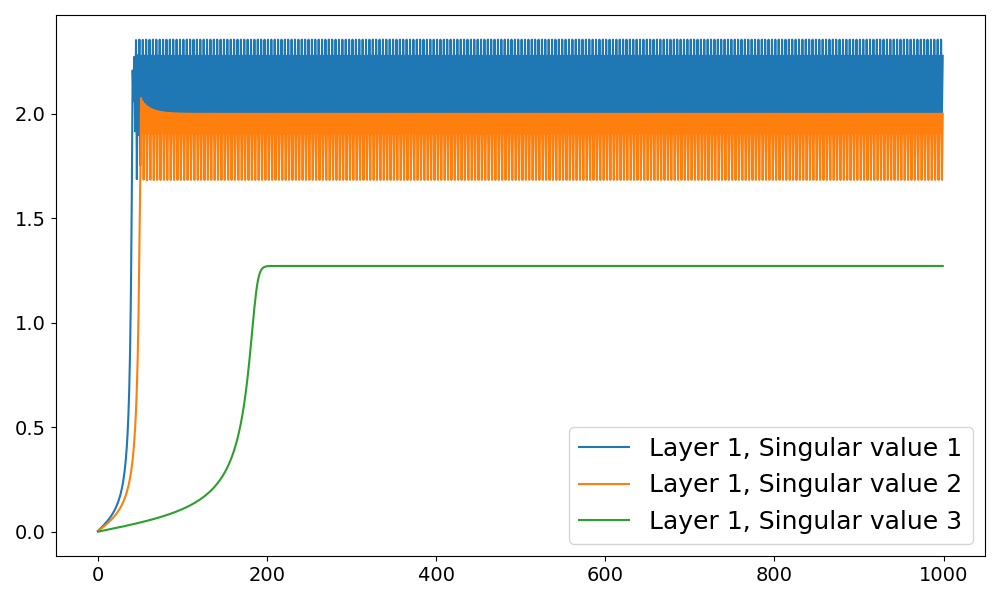}
        \caption*{\footnotesize Layer 1 $\sigma_i$ ($\eta = 0.02$)}
        \label{fig:2}
    \end{subfigure}\hfill
    \begin{subfigure}[b]{0.24\textwidth}
        \centering
        \includegraphics[width=\linewidth]{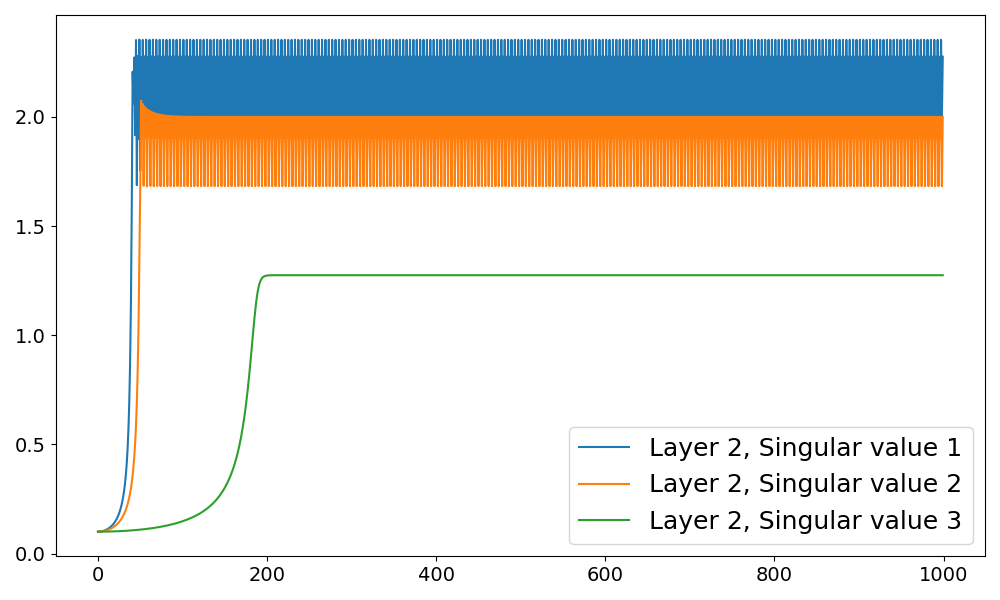}
        \caption*{\footnotesize Layer 2 $\sigma_i$ ($\eta = 0.02$)}
        \label{fig:3}
    \end{subfigure}\hfill
    \begin{subfigure}[b]{0.24\textwidth}
        \centering
        \includegraphics[width=\linewidth]{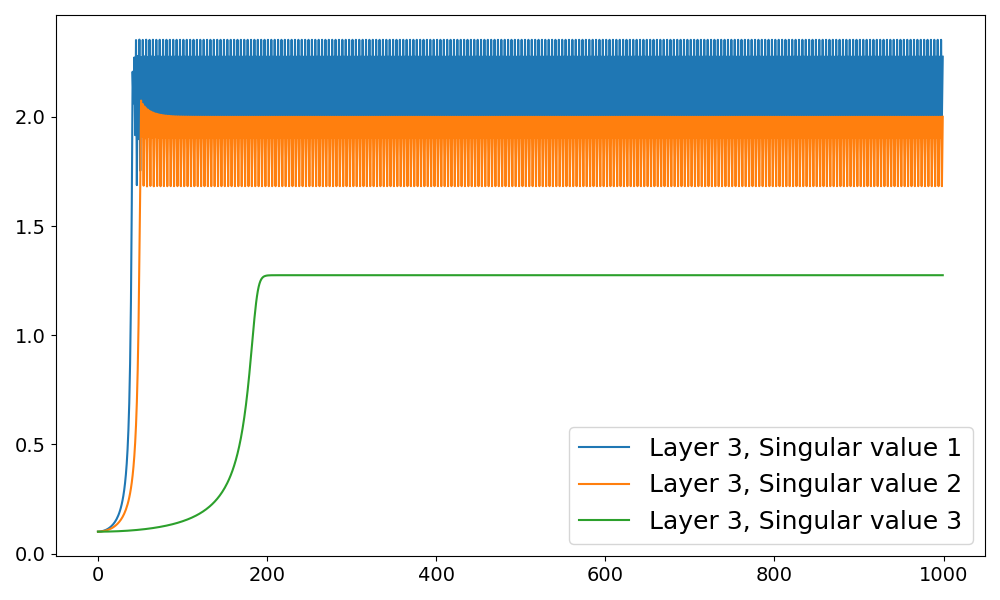}
        \caption*{\footnotesize Layer 3 $\sigma_i$ ($\eta = 0.02$)}
        \label{fig:4}
    \end{subfigure}

    \begin{subfigure}[b]{0.24\textwidth}
        \centering
        \includegraphics[width=\linewidth]{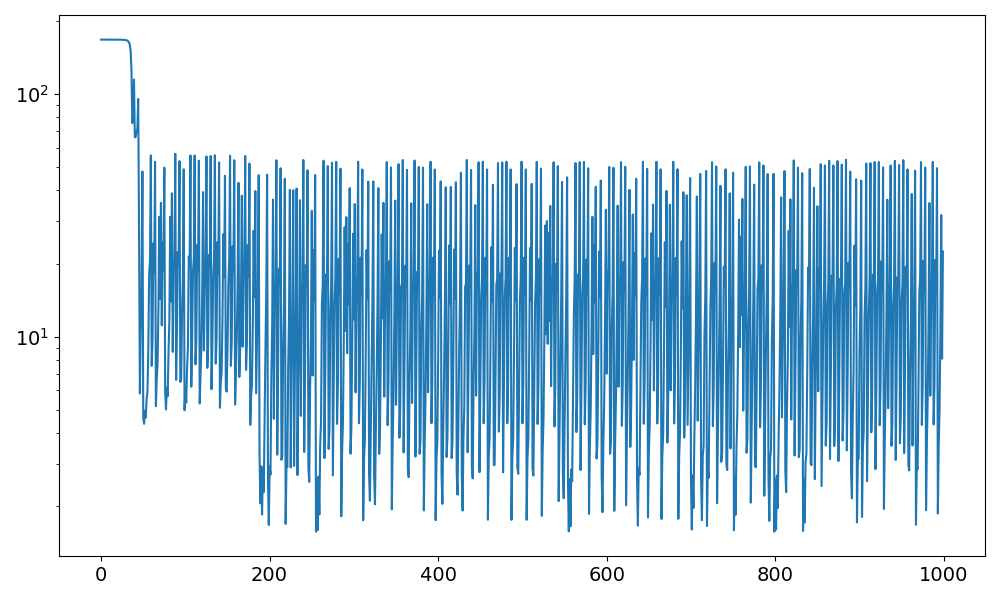}
        \caption*{\footnotesize Train Loss ($\eta = 0.022$) }
        \label{fig:1}
    \end{subfigure}\hfill
    \begin{subfigure}[b]{0.24\textwidth}
        \centering
        \includegraphics[width=\linewidth]{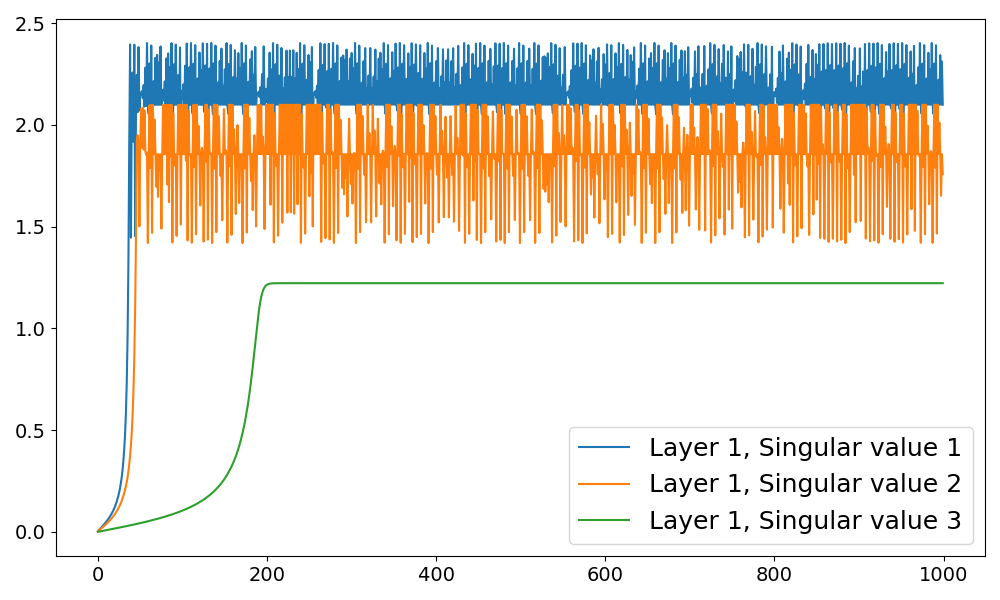}
        \caption*{\footnotesize Layer 1 $\sigma_i$ ($\eta = 0.022$)}
        \label{fig:2}
    \end{subfigure}\hfill
    \begin{subfigure}[b]{0.24\textwidth}
        \centering
        \includegraphics[width=\linewidth]{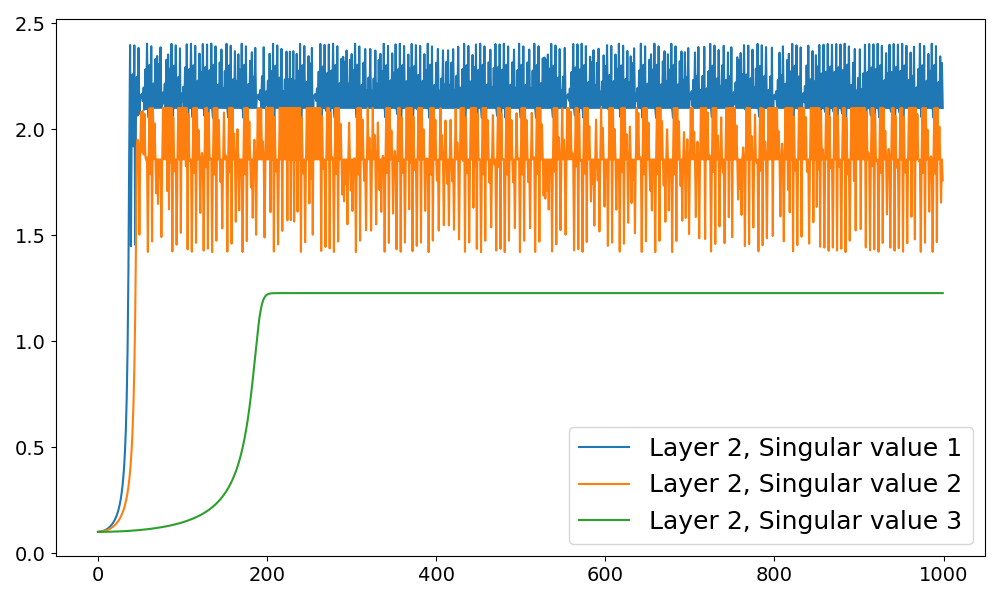}
        \caption*{\footnotesize Layer 2 $\sigma_i$ ($\eta = 0.022$)}
        \label{fig:3}
    \end{subfigure}\hfill
    \begin{subfigure}[b]{0.24\textwidth}
        \centering
        \includegraphics[width=\linewidth]{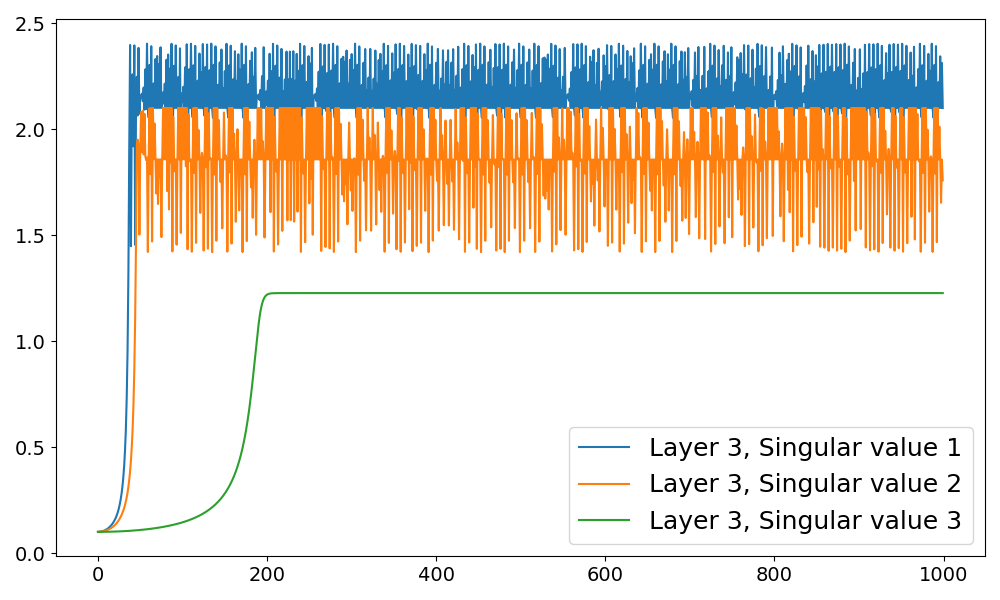}
        \caption*{\footnotesize Layer 3 $\sigma_i$ ($\eta = 0.022$)}
        \label{fig:4}
    \end{subfigure}
    \caption{Depiction of the edge of stability progressively where oscillation is occurring on each singular value depending on the learning rate $\eta$. When $\eta= 0.0154$, oscillation occur on the first singular value. When $\eta=0.0165$, oscillation occur on second singular value.}
    \label{fig:progressive_eta_dln}
\end{figure}

Next, we provide additional experiments demonstrating stronger oscillation in feature directions as measured by the singular values. To this end, we consider a 4-layer MLP with ReLU activations with hidden layer size in each unit of 200 for classification on a subsampled 20K set on MNIST and CIFAR-10. In Figure~\ref{fig:non-lin}, we show that the oscillations in the training loss are artifacts of jumps only in the top singular values, which is also what we observe in the DLN setting.

\begin{figure}[h!]
    \centering
    \begin{subfigure}[b]{0.485\textwidth}
        \centering
        \includegraphics[width=\textwidth]{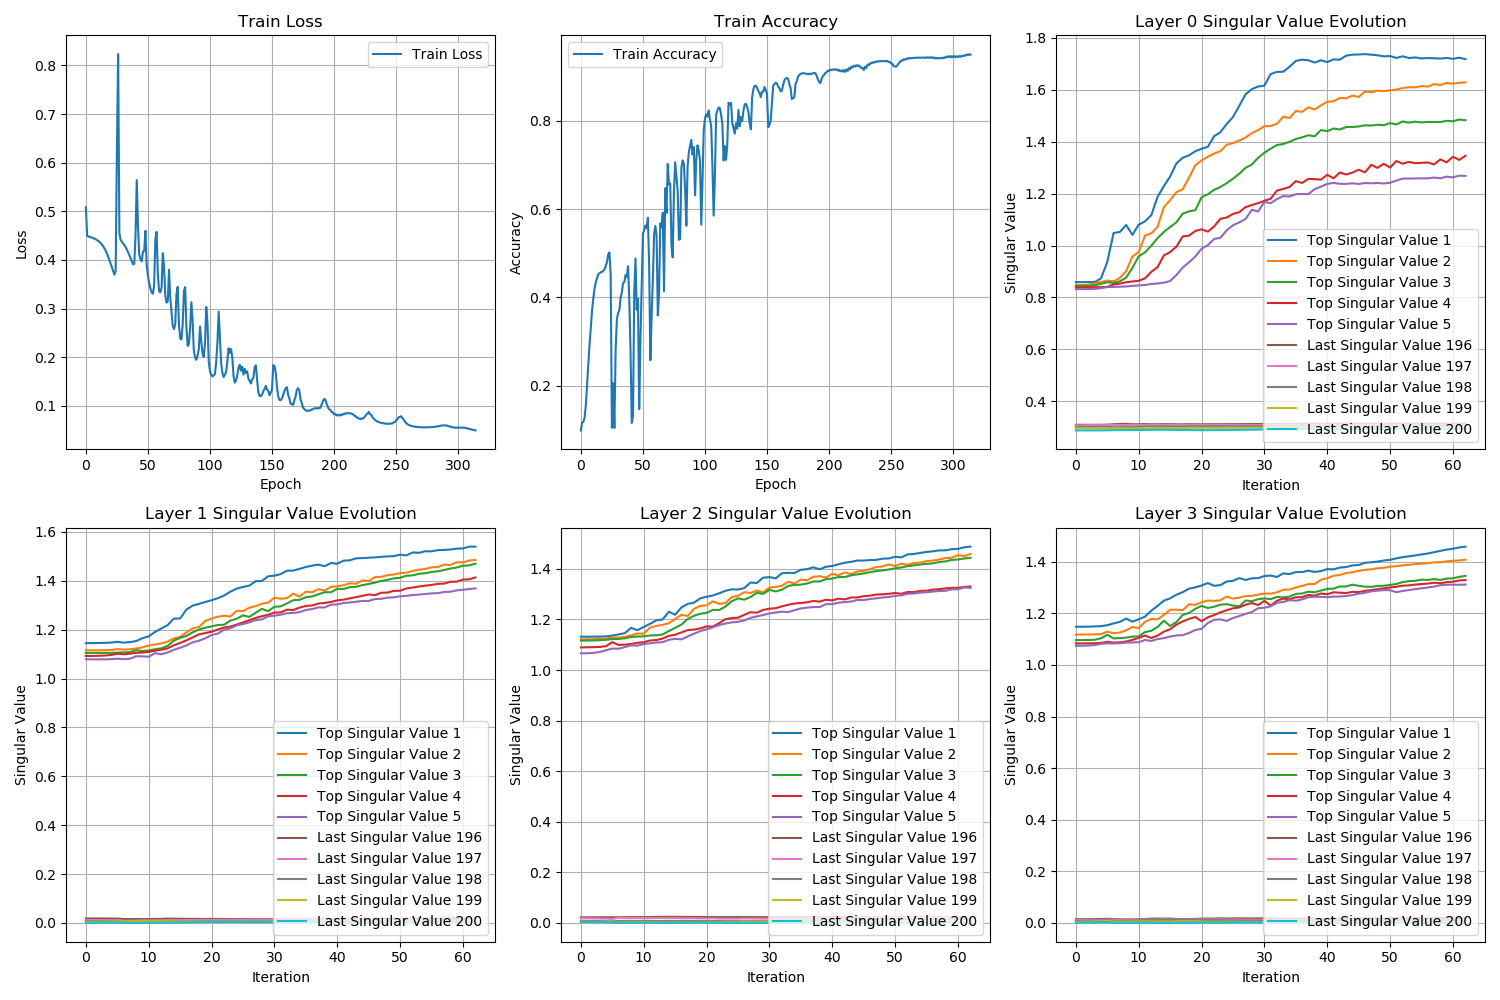}
        \caption*{MNIST Dataset with 4-Layer MLP}
        \label{fig:first_image}
    \end{subfigure}
    \hfill
    \begin{subfigure}[b]{0.485\textwidth}
        \centering
        \includegraphics[width=\textwidth]{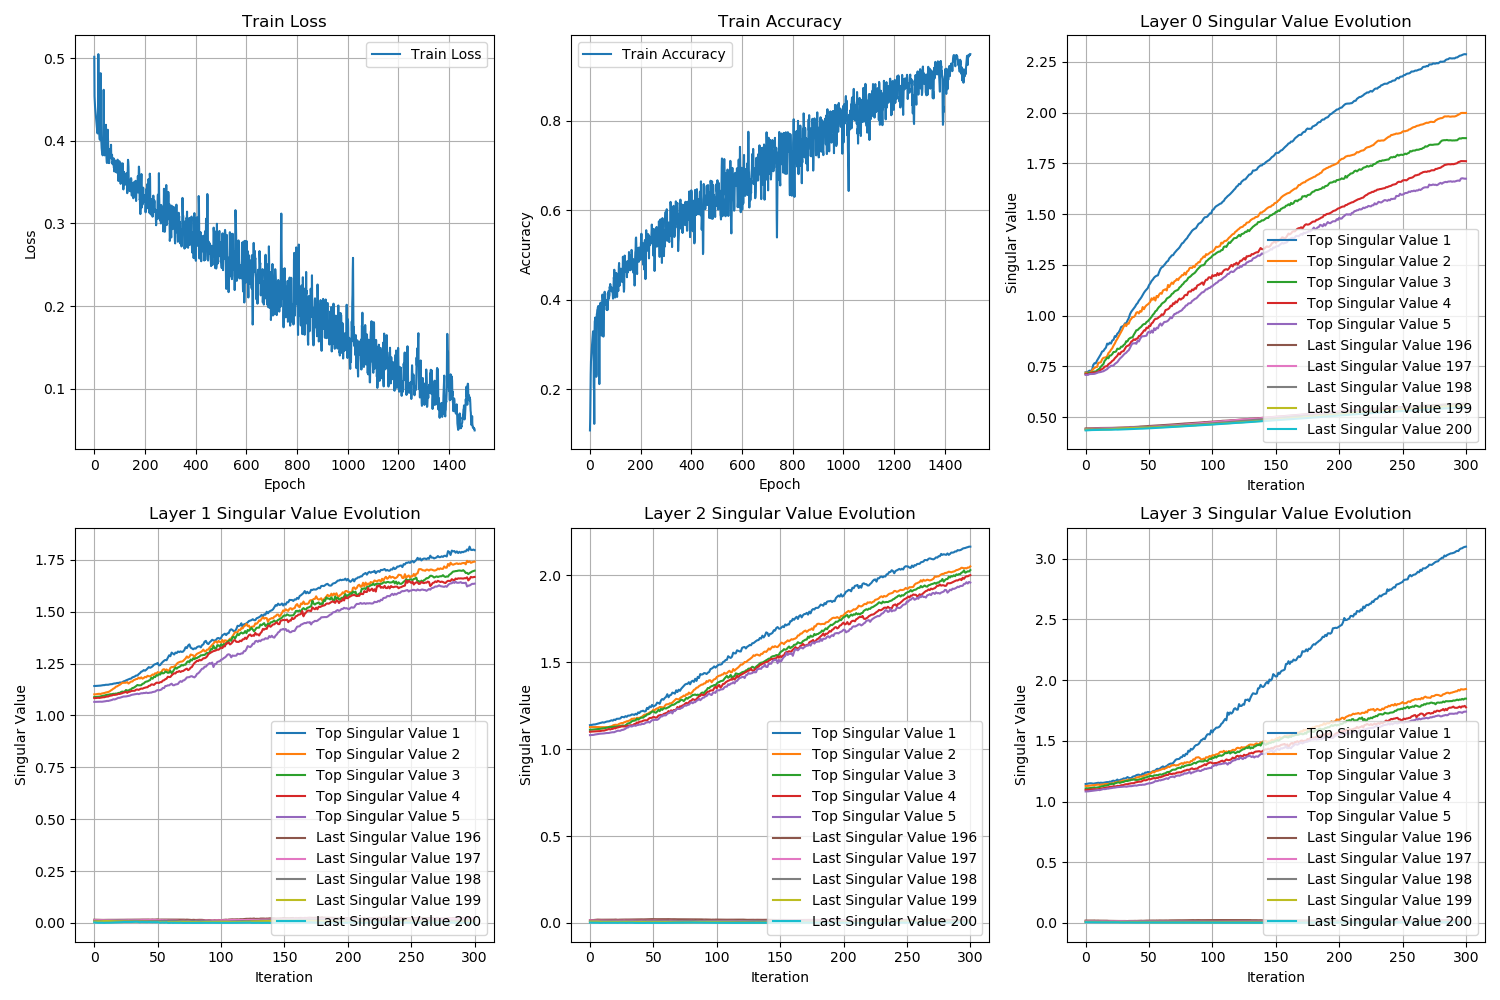}
        \caption*{CIFAR-10 Dataset with 4-Layer MLP}
        \label{fig:second_image}
    \end{subfigure}
    \caption{Prevalence of oscillatory behaviors in top subspaces in $4$-layer networks with ReLU activations on two different datasets.}
    \label{fig:non-lin}
\end{figure}

\subsection{Oscillations in Low-Rank Adaptors}
\label{sec:lora_exp}

Previously, we investigated the differences in oscillations (i.e., oscillations versus catapults) in deep linear and nonlinear networks, and how changes in the landscape present one behavior or the other. Low-rank adaptation (LoRA)~\citep{lora} has arguably become one of the most popular methods for fine-tuning deep neural networks. 
By viewing the adaptations as individual low-rank matrix factorization problems, then this formulation closely aligns with our theoretical setup with a depth of $2$. Hence, we investigate (i) how oscillations may appear in such a setup and (ii) what these oscillations may imply in terms of generalization.

Briefly, the main idea behind LoRA is that rather than training from scratch, we can update two low-rank factor matrices to ``append'' onto an existing weight matrix.
That is, give a pre-trained weight matrix $\mathbf{W}_0 \in \mathbb{R}^{d_1 \times d_2}$, LoRA involves updating two low-rank factors commonly referred to as ``adaptors'':
\begin{align*}
    \underbrace{\mathbf{W}_\star}_{\text{new weight}} = \underbrace{\mathbf{W}_0}_{\text{pre-trained weight}} + \underbrace{\mathbf{AB}^\top}_{\text{adaptors}}.
\end{align*}
For a sufficiently small rank $r$, upon training only $\mathbf{A} \in \mbb{R}^{d_1 \times r}$ and $\mathbf{B} \in \mbb{R}^{d_2 \times r}$, $\mathbf{W}_\star \in \mbb{R}^{d_1 \times d_2}$  is used for inference. 

\begin{wrapfigure}{r}{0.375\textwidth}
  \begin{center}
    \includegraphics[width=0.375\textwidth]{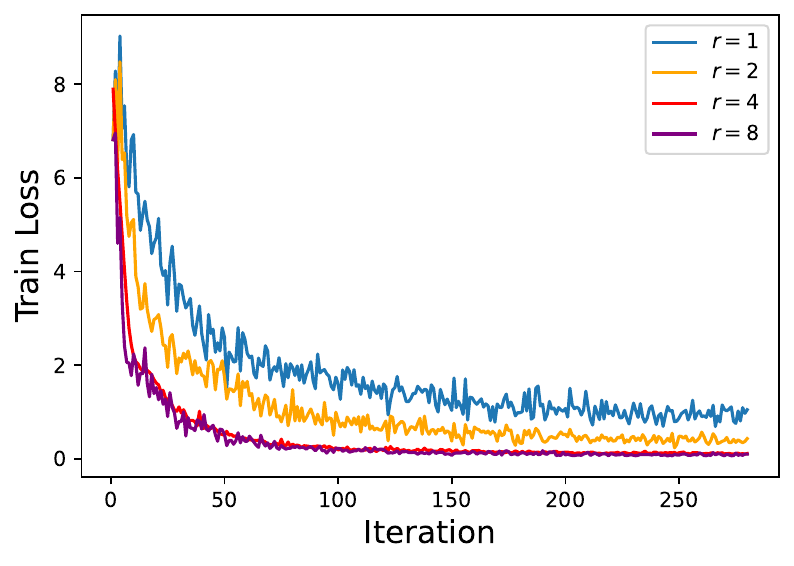}
  \end{center}
  \caption{Catapults in the training loss for different ranks for LoRA.}
\label{fig:rank_vs_correlation}
\end{wrapfigure}
For the experimental settings, we follow the setup used by~\cite{yaras2024compressible} and consider a pre-trained BERT~\citep{wang2018glue} base model and apply
adaptation on all attention and feedforward weights in the transformer, resulting in 72 adapted
layers in total. We choose an initialization scale of $\alpha = 10^{-3}$ for the adaptors and randomly sample $512$ examples from the STS-B~\citep{wang2018glue} dataset for fine-tuning.  We choose a batch size of 64  with a maximum sequence length of 128 tokens. 
First, we experiment how large the rank of the adaptors must be to drive the entire network to EOS. Using a learning rate of $\eta = 10^{-4}$, Figure~\ref{fig:rank_vs_correlation} shows oscillatory behavior across all ranks. However, this behavior may also be an artifact of the stochasticity induced by updating with only a batch of samples. Notably, for ranks $r = 4$ and $r = 8$, there are catapults (or jumps) that occur very early in the iterations, which do not occur for $r = 1$ or $r = 2$. Then, using a rank of $r=8$, we explore the implications of oscillations and catapults for generalization, aiming to determine whether these catapults correspond to improved generalization.

 In Figure~\ref{fig:lr_vs_correlation}, we present the training loss and Pearson correlation for different learning rates.
 When the learning rate is large enough to induce catapults (as seen for $\eta = 10^{-4}$), we observe that the training loss decreases rapidly, resulting in a very high Pearson correlation. In contrast, when the learning rate is small, convergence takes much longer, as the model seems to bounce around within the same local basin before reaching a low training loss. These results suggest that there may exist a combination of rank and learning rate that can converge to an optimal solution (as measured by Pearson correlation) more quickly and with better generalization by inducing catapults in the loss through EOS, as the learning rate of $10^{-4}$ appears to yield the highest Pearson correlation.
We leave for future work a careful study of this observation, aiming to accurately select the learning rate to maximize the efficiency of LoRA.
\begin{figure}[t!]
    \centering
     \begin{subfigure}[t!]{0.495\textwidth}
         \centering
        \includegraphics[width=0.75\textwidth]{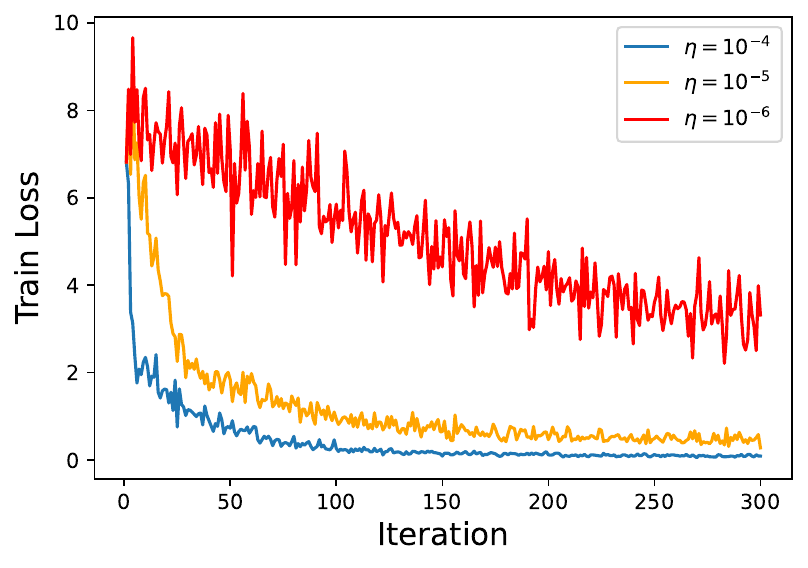}
     \end{subfigure}
     \begin{subfigure}[t!]{0.495\textwidth}
         \centering
         \includegraphics[width=0.75\textwidth]{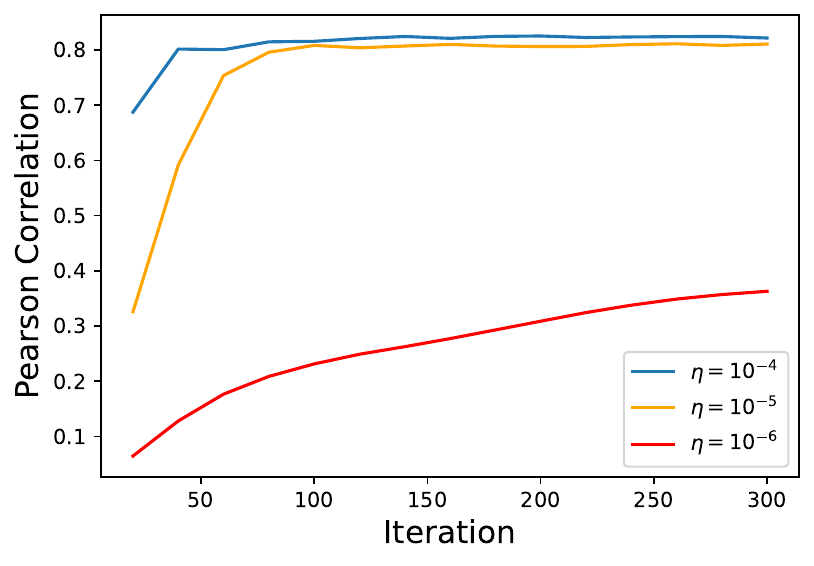}
     \end{subfigure}
    \caption{Illustration of different behaviors in the training loss for various learning rates with a fixed rank of $r=8$ for fine-tuning BERT using LoRA. When the learning rate is large enough to induce catapults in the loss (visible early in the stages for $\eta = 10^{-4}$), the adaptors converge to a point with high Pearson correlation much more rapidly.}
    
    \label{fig:lr_vs_correlation}
\end{figure}

\clearpage

\section{Deferred Proofs}
\label{sec:proofs}
\begin{manualpropositioninner}[Singular Vector Stationary Set]
Consider the deep matrix factorization loss in Equation~(\ref{eqn:deep_mf}). Let $\mbf{M}_\star = \mbf{U}_\star \mbf{\Sigma}_\star \mbf{V}_\star^\top$ and 
$\mbf{W}_\ell(t) = \mbf{U}_\ell(t) \mbf{\Sigma}_\ell(t) \mbf{V}_\ell^\top(t)$ denote the compact SVD for the target matrix and the $\ell$-th layer weight matrix at time $t$, respectively. For any time $t\geq 0$, if $\dot{\mbf{U}}_\ell(t) = \dot{\mbf{V}}_\ell(t) = 0$ for all $\ell \in [L]$, then the singular vector stationary points for each weight matrix are given by
\begin{align*}
\mathrm{SVS}(f(\mbf{\Theta})) = 
\begin{cases}
    (\mbf{U}_L, \mbf{V}_L) &= (\mbf{U}_\star, \mbf{Q}_L), \\
    (\mbf{U}_\ell, \mbf{V}_\ell) &= (\mbf{Q}_{\ell+1}, \mbf{Q}_\ell), \quad\forall \ell \in [2, L-1], \\
    (\mbf{U}_1, \mbf{V}_1) &= (\mbf{Q}_2, \mbf{V}_\star),
\end{cases}
\end{align*}
where \(\{\mbf{Q}_\ell\}_{\ell=2}^{L}\) can be any orthogonal matrices. \label{svs-set}
\end{manualpropositioninner}

\begin{proof}

Let us consider the dynamics of $\mbf{W}_\ell(t)$ in terms of its SVD with respect to time:
\begin{align}
\label{eqn:svd_rynamics}
    \dot{\mbf{W}}_\ell(t) &= \dot{\mbf{U}}_\ell(t) \mbf{\Sigma}_\ell(t) \mbf{V}_\ell^\top(t) + \mbf{U}_\ell(t) \dot{\mbf{\Sigma}}_\ell(t) \mbf{V}_\ell^\top(t) + \mbf{U}_\ell(t) \mbf{\Sigma}_\ell(t) \dot{\mbf{V}}_\ell^\top(t).
\end{align}
By left multiplying by \(\mbf{U}_\ell^\top(t)\) and right multiplying by \(\mbf{V}_\ell(t)\), we have
\begin{align}
    \mbf{U}_\ell^\top(t) \dot{\mbf{W}}_\ell(t) \mbf{V}_\ell(t) &= \mbf{U}_\ell^\top(t) \dot{\mbf{U}}_\ell(t) \mbf{\Sigma}_\ell(t) + \dot{\mbf{\Sigma}}_\ell(t) + \mbf{\Sigma}_\ell(t) \dot{\mbf{V}}_\ell^\top(t) \mbf{V}_\ell(t), 
\end{align}
where we used the fact that \(\mbf{U}_\ell(t)\) and \(\mbf{V}_\ell(t)\) have orthonormal columns. Now, note that we also have
\begin{align*}
    \mbf{U}_\ell^\top(t) \mbf{U}_\ell(t) = \mbf{I}_r \implies \dot{\mbf{U}}_\ell^\top(t) \mbf{U}_\ell(t) + \mbf{U}_\ell^\top(t) \dot{\mbf{U}}_\ell(t) = \mbf{0},
\end{align*}
which also holds for $\mbf{V}_\ell(t)$. This implies that $\dot{\mbf{U}}_\ell^\top(t) \mbf{U}_\ell(t)$ is a skew-symmetric matrix, and hence have zero diagonals. 
Since \(\mbf{\Sigma}_\ell(t)\) is diagonal, \(\mbf{U}_\ell^\top(t) \dot{\mbf{U}}_\ell(t) \mbf{\Sigma}_\ell(t)\) and \(\mbf{\Sigma}_\ell(t) \dot{\mbf{V}}_\ell^\top(t) \mbf{V}_\ell(t)\) have zero diagonals as well. On the other hand, since \(\dot{\mbf{\Sigma}}_\ell(t)\) is a diagonal matrix, we can write
\begin{align}
\label{eqn:diag_inv}
    \hat{\mbf{I}}_r \odot \left(\mbf{U}_\ell^\top(t) \dot{\mbf{W}}_\ell(t) \mbf{V}_\ell(t)\right) &= \mbf{U}_\ell^\top(t) \dot{\mbf{U}}_\ell(t) \mbf{\Sigma}_\ell(t) + \mbf{\Sigma}_\ell(t) \dot{\mbf{V}}_\ell^\top(t) \mbf{V}_\ell(t), 
\end{align}
where \(\odot\) stands for the Hadamard product and \(\hat{\mbf{I}}_r\) is a square matrix holding zeros on its diagonal and ones elsewhere. Taking transpose of Equation~(\ref{eqn:diag_inv}), while recalling that \(\mbf{U}_\ell^\top(t) \dot{\mbf{U}}_\ell(t)\) and \(\mbf{V}_\ell^\top(t) \dot{\mbf{V}}_\ell(t)\) are skew-symmetric, we have
\begin{align}
\label{eqn:diag_inv_transpose}
    \hat{\mbf{I}}_{r} \odot \left(\mbf{V}_\ell^\top(t) \dot{\mbf{W}}_\ell^\top(t) \mbf{U}_\ell(t)\right) &= -\mbf{\Sigma}_\ell(t) \mbf{U}_\ell^\top(t) \dot{\mbf{U}}_\ell(t) - \dot{\mbf{V}}_\ell^\top(t) \mbf{V}_\ell(t) \mbf{\Sigma}_\ell(t). 
\end{align}
Then, by right multiplying Equation~(\ref{eqn:diag_inv}) by \(\mbf{\Sigma}_\ell(t)\), left-multiply Equation~(\ref{eqn:diag_inv_transpose}) by \(\mbf{\Sigma}_\ell(t)\), and by adding the two terms, we get
\begin{align*}
    \hat{\mbf{I}}_{r} \odot \biggl(\mbf{U}_\ell^\top(t) \dot{\mbf{W}}_\ell(t) \mbf{V}_\ell(t) \mbf{\Sigma}_\ell(t) + \mbf{\Sigma}_\ell(t) \mbf{V}_\ell^\top(t) &\dot{\mbf{W}}_\ell^\top(t) \mbf{U}_\ell(t)\biggr) \\
    &= \mbf{U}_\ell^\top(t) \dot{\mbf{U}}_\ell(t) \mbf{\Sigma}_\ell^2(t) - \mbf{\Sigma}_\ell^2(t) \dot{\mbf{V}}_\ell^\top(t) \mbf{V}_\ell(t). 
\end{align*}
Since we assume that the singular values of $\mbf{M}_\star$ are distinct, the top-$r$ diagonal elements of \(\mbf{\Sigma}_{\ell}^2(t)\) are also distinct (i.e., $\Sigma^2_{r}(t) \neq \Sigma^2_{r'}(t) \text{ for } r \neq r'$). This implies that
\begin{align*}
    \mbf{U}_{\ell}^\top(t) \dot{\mbf{U}}_{\ell}(t) &= \mbf{H}(t) \odot \left[\mbf{U}_{\ell}^\top(t) \dot{\mbf{W}}_{\ell}(t) \mbf{V}_{\ell}(t) \mbf{\Sigma}_{\ell}(t) + \mbf{\Sigma}_{\ell}(t) \mbf{V}_{\ell}^\top(t) \dot{\mbf{W}}_{\ell}^\top(t) \mbf{U}_{\ell}(t)\right], 
\end{align*}

where the matrix \(\mbf{H}(t) \in \mathbb{R}^{d\times d}\) is defined by:
\begin{align}
    H_{r,r'}(t) := 
    \begin{cases}
    \left(\Sigma^2_{r'}(t) - \Sigma^2_r(t)\right)^{-1}, & r \neq r', \\
    0, & r = r'.
    \end{cases}
\end{align}

Then, multiplying from the left by \(\mbf{U}_{\ell}(t)\) yields
\begin{align}
    \mbf{P}_{\mbf{U}_{\ell}(t)} \dot{\mbf{W}}_{\ell}(t) &= \mbf{U}_{\ell}(t) \left(\mbf{H}(t) \odot \left[\mbf{U}_{\ell}^\top(t) \dot{\mbf{W}}_{\ell}(t) \mbf{V}_{\ell}(t) \mbf{\Sigma}_{\ell}(t) + \mbf{\Sigma}_{\ell}(t) \mbf{V}_{\ell}^\top(t) \dot{\mbf{W}}_{\ell}^\top(t) \mbf{U}_{\ell}(t)\right]\right), 
\end{align}
with \(\mbf{P}_{\mbf{U}_{\ell}(t)} := \mbf{U}_{\ell}(t) \mbf{U}_{\ell}^\top(t)\) being the projection onto the subspace spanned by the (orthonormal) columns of \(\mbf{U}_{\ell}(t)\). Denote by \(\mbf{P}_{\mbf{U}_{{\ell}\perp}(t)}\) the projection onto the orthogonal complement ( i.e., $\mbf{P}_{\mbf{U}_{\ell\perp}(t)} := \mbf{I}_r - \mbf{U}_{\ell}(t) \mbf{U}_{\ell}^\top(t)$). Apply \(\mbf{P}_{\mbf{U}_{\ell\perp}(t)}\) to both sides of Equation~(\ref{eqn:svd_rynamics}):
\begin{align}
    \mbf{P}_{\mbf{U}_{\ell\perp}(t)} \dot{\mbf{W}}_{\ell}(t) = \mbf{P}_{\mbf{U}_{\ell\perp}(t)} \dot{\mbf{U}}_{\ell}(t) \mbf{\Sigma}_\ell(t) \mbf{V}_{\ell}^\top(t) &+ \mbf{P}_{\mbf{U}_{\ell\perp}(t)} \mbf{U}_\ell(t) \dot{\mbf{\Sigma}}_{\ell}(t) \mbf{V}_{\ell}^\top(t)\\ &+ \mbf{P}_{\mbf{U}_{\ell\perp}(t)} \mbf{U}_\ell(t) \mbf{\Sigma}_\ell(t) \dot{\mbf{V}}_{\ell}^\top(t). 
\end{align}

Note that \(\mbf{P}_{\mbf{U}_{\ell\perp}(t)} \mbf{U}_\ell(t) = 0\), and multiply from the right by \(\mbf{V}_\ell(t) \mbf{\Sigma}_{\ell}^{-1}(t)\) (the latter is well-defined since we have the compact SVD and the top-$r$ elements are non-zero):
\begin{align}
    \mbf{P}_{\mbf{U}_{\ell\perp}(t)} \dot{\mbf{U}}_\ell(t) &= \mbf{P}_{\mbf{U}_{\ell\perp}(t)} \dot{\mbf{W}}_\ell(t) \mbf{V}_\ell(t) \mbf{\Sigma}_\ell^{-1}(t) = (\mbf{I}_r - \mbf{U}_\ell(t)\mbf{U}^\top(t)) \dot{\mbf{W}}(t) \mbf{V}_\ell(t) \mbf{\Sigma}_\ell^{-1}(t). 
\end{align}
Then by adding the two equations above, we obtain an expression for \(\dot{\mbf{U}}(t)\):
\begin{align}
    \dot{\mbf{U}}_\ell(t) &= \mbf{P}_{\mbf{U}_\ell(t)} \dot{\mbf{U}}_\ell(t) + \mbf{P}_{\mbf{U}_{\ell\perp}(t)} \dot{\mbf{U}}_\ell(t) \nonumber \\
    &= \mbf{U}_\ell(t)\left(\mbf{H}(t) \odot \left[\mbf{U}_\ell^\top(t) \dot{\mbf{W}}_\ell(t) \mbf{V}_\ell(t) \mbf{\Sigma}_\ell(t) + \mbf{\Sigma}_\ell(t) \mbf{V}_\ell^\top(t) \dot{\mbf{W}}_\ell^\top(t) \mbf{U}_\ell(t)\right]\right) \nonumber \\
    &\quad + (\mbf{I}_r - \mbf{U}_\ell(t) \mbf{U}_\ell^\top(t)) \dot{\mbf{W}}(t) \mbf{V}_\ell(t) \mbf{\Sigma}_\ell^{-1}(t). 
\end{align}
We can similarly derive the dynamics for $\dot{\mbf{V}}_\ell(t)$ and $\dot{\mbf{\Sigma}}_\ell(t)$:
\begin{align}
\dot{\mbf{V}}_\ell(t) = \mbf{V}_\ell(t)\left(\mbf{H}(t) \odot \left[\mbf{\Sigma}_\ell(t) \mbf{U}^\top_\ell(t) \dot{\mbf{W}_{\ell}}(t) \mbf{V}_\ell(t) + \mbf{V}^\top_\ell(t) \dot{\mbf{W}_{\ell}}^\top(t) \mbf{U}_\ell(t) \mbf{\Sigma}_\ell(t)\right]\right) \\
+ \left(\mbf{I}_{r} - \mbf{V}_\ell(t)\mbf{V}^\top_\ell(t)\right) \dot{\mbf{W}_{\ell}}^\top(t) \mbf{U}_\ell(t) \mbf{\Sigma}_\ell^{-1}(t), \label{vdiff}
\end{align}
\begin{align*}
   \dot{\mbf{\Sigma}}_\ell(t) = \mbf{I}_r \odot \left[ \mbf{U}^\top_\ell(t) \dot{\mbf{W}}_\ell(t) \mbf{V}_\ell(t) \right].
\end{align*}

Now, we will left multiply $\dot{\mbf{U}}_\ell(t)$ and $\dot{\mbf{V}}_\ell(t)$ with $\mbf{U}_\ell^\top(t)$ and $\mbf{V}_\ell^\top(t)$, respectively, to obtain
\begin{align*}
    \mbf{U}^\top_\ell(t) \dot{\mbf{U}}_\ell(t) &= -\mbf{H}(t) \odot \left[\mbf{U}^\top_\ell(t)\nabla_{\mbf{W}_{\ell}} f(\mbf{\Theta}) \mbf{V}_\ell(t) \mbf{\Sigma}_\ell(t) + \mbf{\Sigma}_\ell(t) \mbf{V}^\top_\ell(t) \nabla_{\mbf{W}_{\ell}} f(\mbf{\Theta}) \mbf{U}_\ell(t)\right], \\
    \mbf{V}^\top_\ell(t) \dot{\mbf{V}}_\ell(t) &= -\mbf{H}(t) \odot \left[\mbf{\Sigma}_\ell(t) \mbf{U}^\top_\ell(t) \nabla_{\mbf{W}_{\ell}} f(\mbf{\Theta}) \mbf{V}_\ell(t) + \mbf{V}^\top_\ell(t) \nabla_{\mbf{W}_{\ell}} f(\mbf{\Theta}) \mbf{U}_\ell(t) \mbf{\Sigma}_\ell(t)\right],
\end{align*}
where we replaced $\dot{\mbf{W}}_\ell(t) \coloneqq -\nabla_{\mbf{W}_{\ell}} f(\mbf{\Theta})$, as $\dot{\mbf{W}}_\ell(t)$ is the gradient of $f(\mbf{\Theta})$ with respect to $\mbf{W}_\ell$ by definition. By rearranging and multiplying by $\mbf{\Sigma}_\ell(t)$, we have
\begin{align}
\label{eqn:diagonal_grad}
      \mbf{U}^\top_\ell(t) \dot{\mbf{U}}_\ell(t) \mbf{\Sigma}_\ell(t) -   \mbf{\Sigma}_\ell(t) \mbf{V}^T (t) \dot{\mbf{V}}_\ell(t) = -  \hat{\mbf{I}}_{r} \odot [\mbf{U}^\top_\ell(t) \nabla_{\mbf{W}_{\ell}} f(\mbf{\Theta}) \mbf{V}_\ell(t)].
\end{align}
Hence, when $\dot{\mbf{U}}_\ell(t)=0$ and $\dot{\mbf{V}}_\ell(t)=0$, it must be that the left-hand side is zero and so $\mbf{U}^\top_\ell(t) \nabla_{\mbf{W}_{\ell}} f(\mbf{\Theta}) \mbf{V}_\ell(t)$ is a diagonal matrix. 

Now, notice that for the given loss function $f(\mbf{\Theta})$, we have
\begin{align*}
   -\dot{\mbf{W}}_\ell(t) = \nabla_{\mbf{W}_{\ell}} f(\mbf{\Theta}(t)) = \mbf{W}^{\top}_{L:\ell+1}(t) \cdot \left(\mbf{W}_{L:1}(t) - \mbf{M}_\star \right) \cdot \mbf{W}^{\top}_{\ell-1:1}(t). 
\end{align*}
Then, from Equation~(\ref{eqn:diagonal_grad}), when the singular vectors are stationary, we have
\begin{align*}
    \mbf{U}_\ell^\top(t)\mbf{W}^{\top}_{L:\ell+1}(t) \cdot \left(\mbf{W}_{L:1}(t) - \mbf{M}_\star \right) \cdot \mbf{W}^{\top}_{\ell-1:1}(t)\mbf{V}_\ell(t)
\end{align*}
must be a diagonal matrix for all $\ell \in [L]$. The only solution to the above should be (since the intermediate singular vectors need to cancel to satisfy the diagonal condition), is the set
\begin{align*}
\mathrm{SVS}(f(\mbf{\Theta})) = 
\begin{cases}
    (\mbf{U}_L, \mbf{V}_L) &= (\mbf{U}_\star, \mbf{Q}_L), \\
    (\mbf{U}_\ell, \mbf{V}_\ell) &= (\mbf{Q}_{\ell+1}, \mbf{Q}_\ell), \quad\forall \ell \in [2, L-1], \\
    (\mbf{U}_1, \mbf{V}_1) &= (\mbf{Q}_2, \mbf{V}_\star),
\end{cases}
\end{align*}
where \(\{\mbf{Q}_\ell\}_{\ell=2}^{L}\) are any set of orthogonal matrices. Then, notice that when the singular vectors are stationary, the dynamics become isolated on the singular values: \begin{align*}
   \dot{\mbf{\Sigma}}_\ell(t) = \mbf{I}_r \odot \left[ \mbf{U}^\top_\ell(t) \dot{\mbf{W}}_\ell(t) \mbf{V}_\ell(t) \right],
\end{align*} 
since $\left[ \mbf{U}^\top_\ell(t) \dot{\mbf{W}}_\ell(t) \mbf{V}_\ell(t) \right]$ is diagonal. This completes the proof.

\end{proof}

\begin{manualtheoreminner}[1-D Subspace Oscillation]
Let $\mbf{M}_\star = \mbf{U}_\star \mbf{\Sigma}_\star \mbf{V}_\star^\top$ denote the SVD of the target matrix and let $S\coloneqq L \sigma^{2-\frac{2}{L}}_{\star,1}$, 
$\alpha' \coloneqq \left( \log\left( \frac{2\sqrt{2}}{\eta S} \right) \cdot 2 \sigma_{\star, 1}^{\frac{4}{L}} \right)^{\frac{1}{4}}$, and $K' \coloneqq \mathrm{max} \left\{ \sum_{\ell=0}^{L-1} \left(\sigma_{\star, 1}^{1-\frac{1}{L} - \frac{1}{L}\ell} \cdot \sigma_{\star, 2}^{\frac{1}{L}\ell}\right)^2,\frac{S}{2\sqrt{2}}\right\}$.
If we run GD on the deep matrix factorization loss with initialization scale $\alpha < \alpha'$ and learning rate $\eta = \frac{2}{K}$, where $K' < K< S$, then under strict balancing, each weight matrix $\mbf{W}_{\ell}(t) \in \mbb{R}^{d\times d}$ oscillates around the minima in a $2$-period fixed orbit as follows:
\begin{align*}
    \mbf{W}_L(t) &= \underbrace{ \rho_i(t)\cdot \mbf{u}_{\star, 1}\mbf{v}_{\star, 1}^{\top} }_{\text{oscillation subspace}}+ \underbrace{\sum_{j=2}^r \sigma_{\star, i}\mbf{u}_{\star, j}\mbf{v}_{\star, j}^{\top}}_{\text{stationary subspace}}, \quad i = 1, 2, \\
    \mbf{W}_\ell(t) &=\underbrace{ \rho_i(t) \cdot\mbf{v}_{\star, 1}\mbf{v}_{\star, 1}^{\top}}_{\text{oscillation subspace}} + \underbrace{\sum_{j=2 }^r \sigma_{\star, i}\mbf{v}_{\star, j}\mbf{v}_{\star, j}^{\top}}_{\text{stationary subspace}}, \quad i = 1, 2, \quad \forall\ell \in [L-1], 
\end{align*}
where $\rho_i(t) \in \{\rho_1, \rho_2\}$
and $\rho_1 \in \left(0, \sigma_{\star, 1}^{1/L}\right)$ and $\rho_2 \in \left(\sigma_{\star, 1}^{1/L}, (2\sigma_{\star, 1})^{1/L}\right)$ are the two real roots of the polynomial $g(\rho)=0$, where
\begin{align*}
    g(\rho) = \rho^L\cdot\frac{1+\left(1 + \eta L(\sigma_{\star, 1} - \rho^L)\cdot \rho^{L-2} \right)^{2L-1}}{1+\left(1 + \eta L(\sigma_{\star, 1} - \rho^L)\cdot \rho^{L-2} \right)^{L-1}} - \sigma_{\star, 1}.
\end{align*}
\label{main:thm}
\end{manualtheoreminner}

\begin{proof}

For ease of exposition, let us denote the first singular value as $\sigma_{1} \coloneqq \sigma_{\ell, 1}$. Under balancing, consider the two-step GD update on the first singular value:
\begin{align*}
    \sigma_1(t+1) &= \sigma_1(t) + \eta L \cdot \left(\sigma_{\star, 1} - \sigma_1^L(t)\right)\cdot \sigma^{L-1}_{1}(t) \\
      \sigma_1(t) = \sigma_1(t+2) &= \sigma_1(t+1) + \eta L \cdot \left(\sigma_{\star, 1} - \sigma_1^L(t+1)\right)\cdot \sigma^{L-1}_{1}(t+1). \tag{By 2-period orbit}
\end{align*}
Define $z \coloneqq \left(1 + \eta L \cdot \left(\sigma_{\star, 1} - \sigma_1^L(t)\right)\cdot \sigma^{L-2}_{1}(t) \right)$ and by plugging in $\sigma_1(t+1)$ for $\sigma_1(t)$, we have
\begin{align*}
    \sigma_1(t) &= \sigma_1(t) z + \eta L \cdot \left(\sigma_{\star, 1} - \sigma_1^L(t)z^L \right) \cdot \sigma_1^{L-1}(t)z^{L-1} \\
    \implies 1 &= z + \eta L \cdot \left(\sigma_{\star, 1} - \sigma_1^L(t)z^L \right) \cdot \sigma_1^{L-2}(t)z^{L-1} \\
    \implies 1 &= \left(1 + \eta L \cdot \left(\sigma_{\star, 1} - \sigma_1^L(t)\right)\cdot \sigma^{L-2}_{1}(t) \right) + \eta L \cdot \left(\sigma_{\star, 1} - \sigma_1^L(t)z^L \right) \cdot \sigma_1^{L-2}(t)z^{L-1} \\
    \implies 0 &= \left(\sigma_{\star, 1} - \sigma_1^L(t)\right) + \left(\sigma_{\star, 1} - \sigma_1^L(t)z^L \right) \cdot z^{L-1}
\end{align*}
Simplifying this expression further, we have
\begin{align*}
    &0 = \sigma_{\star, 1} - \sigma_1^L(t) + \sigma_{\star, 1} z^{L-1} - \sigma_1^L(t) z^{2L-1} \\
    \implies &\sigma_1^L(t) + \sigma_1^L(t) z^{2L-1} =  \sigma_{\star, 1} + \sigma_{\star, 1} z^{L-1} \\
    \implies &\sigma_1^L(t)\cdot\left(1 + z^{2L - 1} \right) = \sigma_{\star, 1}\cdot\left(1 + z^{L - 1} \right) \\
    \implies &\sigma_1^L(t)\frac{\left(1 + z^{2L - 1} \right)}{\left(1 + z^{L - 1} \right)} = \sigma_{\star, 1},
\end{align*}
and by letting $\rho \coloneqq \sigma_1(t)$, we obtain the polynomial
\begin{align*}
    \sigma_{\star, 1} = \rho^L\frac{1+z^{2L-1}}{1+z^{L-1}}, \quad \text{where  } \, z \coloneqq \left(1 + \eta L(\sigma_{\star, 1} - \rho^L)\cdot \rho^{L-2} \right).
\end{align*}
Next, we show the existence of the roots within the ranges for $\rho_1$ and $\rho_2$. First, consider $\rho_1 \in \left(0, \sigma_{\star, 1}^{1/L} \right)$. We will show that for two values within this range, there is a sign change for all $L \geq 2$. More specifically, we show that there exists $\rho \in \left(0, \sigma_{\star, 1}^{1/L} \right)$ such that
\begin{align*}
     \rho^L\frac{1+z^{2L-1}}{1+z^{L-1}} - \sigma_{\star, 1} > 0 \quad \text{and} \quad \rho^L\frac{1+z^{2L-1}}{1+z^{L-1}} - \sigma_{\star, 1} < 0.
\end{align*}
For the positive case, consider $\rho = (\frac{1}{2}\sigma_{\star, 1})^{1/ L}$. We need to show that 
\begin{align*}
    \frac{1+z^{2L-1}}{1+z^{L-1}}  = \frac{1 + \left(1+\eta L\cdot\left(\frac{\sigma_{\star, 1}}{2}\right)\frac{\sigma_{\star, 1}^{1-\frac{2}{L}}}{2^{1 - \frac{2}{L}}}\right)^{2L-1}}{1 + \left(1+\eta L\cdot\left(\frac{\sigma_{\star, 1}}{2}\right)\frac{\sigma_{\star, 1}^{1-\frac{2}{L}}}{2^{1 - \frac{2}{L}}}\right)^{L-1}} > 2.
\end{align*}
To do this, we will plug in the smallest possible value of $\eta = \frac{2}{L\sigma_{\star, 1}^{2 - \frac{2}{L}}}$ to show that the fraction is still greater than $2$, which gives us
\begin{align}
\label{eqn:first_range_pos}
    \frac{1 + \left(1+\frac{1}{ 2^{1 - \frac{2}{L}}} \right)^{2L-1}}{1 + \left(1+\frac{1}{ 2^{1 - \frac{2}{L}}} \right)^{L-1}},
\end{align}
which is an increasing function of $L$ for all $L\geq 2$ and so Equation~(\ref{eqn:first_range_pos}) must be greater than $2$. For the negative case, we can simply consider $\rho = 0$.
Hence, since the polynomial is continuous, by the Intermediate Value Theorem (IVT), there must exist a root within the range $\rho \in \left(0, \sigma_{\star, 1}^{1/L} \right)$.

Next, consider the range $\rho_2 \in \left(\sigma_{\star, 1}^{1/L}, (2\sigma_{\star, 1})^{1/L}\right)$. Similarly, we will show sign changes for two values in $\rho_2$.
For the positive case, consider $\rho = \left(\frac{3}{2} \sigma_{\star, 1}\right)^{1/L}$. For $\eta$, we can plug in the smallest possible value within the range to show that this value of $\rho$ still provides a positive quantity. Specifically, we need to show that
\begin{align*}
    \frac{1+z^{2L-1}}{1+z^{L-1}} - \sigma_{\star, 1} > \frac{2}{3} \implies \frac{1+\left(1+\frac{2}{\sigma_{\star, 1}^{2- \frac{2}{L}}}\cdot(\sigma_{\star, 1} - \frac{3}{2}\sigma_{\star, 1})\cdot \left(\frac{3}{2}\sigma_{\star, 1}\right)^{1 - \frac{2}{L}} \right)^{2L-1}}{1+\left(1+\frac{2}{\sigma_{\star, 1}^{2- \frac{2}{L}}}\cdot(\sigma_{\star, 1} - \frac{3}{2}\sigma_{\star, 1})\cdot \left(\frac{3}{2}\sigma_{\star, 1}\right)^{1 - \frac{2}{L}} \right)^{L-1}} > \frac{2}{3}.
\end{align*}
We can simplify the fraction as follows:
\begin{align*}
    \frac{1+\left(1+\frac{2}{\sigma_{\star, 1}^{2- \frac{2}{L}}}\cdot(\sigma_{\star, 1} - \frac{3}{2}\sigma_{\star, 1})\cdot \left(\frac{3}{2}\sigma_{\star, 1}\right)^{1 - \frac{2}{L}} \right)^{2L-1}}{1+\left(1+\frac{2}{\sigma_{\star, 1}^{2- \frac{2}{L}}}\cdot(\sigma_{\star, 1} - \frac{3}{2}\sigma_{\star, 1})\cdot \left(\frac{3}{2}\sigma_{\star, 1}\right)^{1 - \frac{2}{L}} \right)^{L-1}} = 
    \frac{1+\left(1-(\frac{3}{2})^{1 - \frac{2}{L}} \right)^{2L-1}}{1+\left(1-(\frac{3}{2})^{1 - \frac{2}{L}} \right)^{L-1}}.
\end{align*}
Then, since we are subtracting by $(\frac{3}{2})^{1 - \frac{2}{L}}$, we can plug in its largest value for $L\geq 2$, which is $3/2$. This gives us 
\begin{align*}
    \frac{1+\left(-0.5\right)^{2L-1}}{1+\left(-0.5 \right)^{L-1}} > \frac{2}{3},
\end{align*}
as for odd values of $L$, the function increases to $1$ starting from $L=2$, and decreases to $1$ for even $L$. 
To check negativity, let us define
\begin{align*}
    h(\rho) \coloneqq \frac{f(\rho)}{g(\rho)} \coloneqq \frac{\rho^L \left(1 + z^{2L-1} \right)}{1 + z^{L-1}}.
\end{align*}
We will show that $h'\left(\sigma_{\star,1}^{1/L} \right) < 0$:
\begin{align*}
h'\left(\sigma_{\star,1}^{1/L} \right) &= \frac{f'\left(\sigma_{\star,1}^{1/L} \right)g\left(\sigma_{\star,1}^{1/L} \right) - f\left(\sigma_{\star,1}^{1/L} \right)g'\left(\sigma_{\star,1}^{1/L} \right)}{g^2\left(\sigma_{\star,1}^{1/L} \right)} \\
&= \frac{f'\left(\sigma_{\star,1}^{1/L} \right) - \sigma_{\star, 1}g'\left(\sigma_{\star,1}^{1/L} \right)}{2} \\
&= \frac{L\sigma_{\star, 1}^{1 - \frac{1}{L}} - \sigma_{\star, 1}(2L-1)\left(\eta L^2 \sigma_{\star,1}^{2 -\frac{3}{L}} \right) - \sigma_{\star, 1}(L-1)\left(\eta L^2 \sigma_{\star,1}^{2 -\frac{3}{L}} \right) }{2} \\
&= \frac{L\sigma_{\star, 1}^{1 - \frac{1}{L}} - (3L-2)\left(\eta L^2 \sigma_{\star,1}^{3 -\frac{3}{L}} \right) }{2} < 0,
\end{align*}
as otherwise we need $\eta \leq \frac{\sigma_{\star, 1}^{2/L - 2}}{3L^2 - 2L}$, which is out of the range of interest. Since $h'(\rho)< 0$, it follows that there exists a $\delta > 0$ such that $h(\rho) > h(x)$ for all $x$ such that $\rho < x < \rho+\delta$. Lastly, since $h(\rho) - \sigma_{\star, 1} = 0$ for $\rho = \sigma_{\star, 1}^{1/L}$, it follows that $h(\rho) - \sigma_{\star, 1}$ must be negative at $\rho + \delta$.
Similarly, by IVT, there must exist a root within the range 
$\rho_2 \in \left(\sigma_{\star, 1}^{1/L}, (2\sigma_{\star, 1})^{1/L}\right)$. 

Then, by Proposition~\ref{prop:one_zero_svs_set}, notice that we can write the dynamics of the weight matrices as
\begin{align*}
    \mbf{W}_L(t) &= \sigma_{\star, 1} \mbf{u}_{\star, 1}\mbf{v}_{\star, 1}^{\top} + \sum_{j=1}^r \sigma_{i, \star}\mbf{u}_{\star, j}\mbf{v}_{\star, j}^{\top},  \\
    \mbf{W}_\ell(t) &= \sigma_{\star, 1} \mbf{v}_{\star, 1}\mbf{v}_{\star, 1}^{\top} + \sum_{j=1}^r \sigma_{i, \star}\mbf{v}_{\star, j}\mbf{v}_{\star, j}^{\top}, \quad \forall\ell \in [L-1].
\end{align*}
By the oscillations, we can replace $\sigma_{\star, 1}$ with $\rho_i$ for $i=1, 2$.
This completes the proof.

\end{proof}

\begin{manuallemmainner}
[Hessian Eigenvalues at Convergence]
   Consider running GD on the deep matrix factorization loss $f(\mbf{\Theta})$ defined in Equation~(\ref{eqn:deep_mf}). Under strict balancing, for any stationary point $\mbf{\Theta}$ such that $\nabla_{\mbf{\Theta}} f(\mbf{\Theta}) = 0$, the set of all non-zero eigenvalues of the Hessian of the training loss are given by
    \begin{align*}
       \lambda_{\mbf{\Theta}} = \underbrace{\left\{L \sigma_{\star, i}^{2 - \frac{2}{L}}, \sigma_{\star, i}^{2 - \frac{2}{L}}\right\}_{i=1}^r, }_{\text{self-interaction}} \, \bigcup \, \underbrace{\left\{\sum_{\ell=0}^{L-1} \left(\sigma_{\star, i}^{1-\frac{1}{L} - \frac{1}{L}\ell} \cdot \sigma_{\star, j}^{\frac{1}{L}\ell}\right)^2\right\}_{i\neq j}^{r}}_{\text{interaction with other singular values}} \,\bigcup \, \underbrace{\left\{\sum_{\ell=0}^{L-1} \left(\sigma_{\star, k}^{1-\frac{1}{L} - \frac{1}{L}\ell} \cdot \alpha^{\ell}\right)^2\right\}_{k = 1}^{r}}_{\text{interaction with initialization}} 
    \end{align*}
    where $\sigma_{\star, i}$ is the $i$-th singular value of the target matrix $\mbf{M}_\star \in \mbb{R}^{d\times d}$,  $\alpha \in \mbb{R}$ is the initialization scale, $L$ is the depth of the network, and the last set of eigenvalues each have a multiplicity of $d-r$. \label{hess-eig}
\end{manuallemmainner}

\begin{proof}
     By Proposition~\ref{prop:one_zero_svs_set}, we can rewrite the loss in Equation~(\ref{eqn:deep_mf}) as
    \begin{align*}
        \frac{1}{2} \left\|\mbf{W}_{L:1} - \mbf{M}_\star\right\|^2_{\mathsf{F}} = \frac{1}{2} \|\mbf{\Sigma}_{L:1} - \mbf{\Sigma}_\star\|^2_{\mathsf{F}},
    \end{align*}
    where $\mbf{\sigma}_{L:1}$ are the singular values of $\mbf{M}_\star$.
    To calculate the Hessian matrix, we will consider taking the gradient with respect to the vectorized weight matrices. Consider the following vectorized loss:
    \begin{align*}
        f(\mbf{\Theta}) = \frac{1}{2} \|\mbf{\Sigma}_{L:1} - \mbf{\Sigma}_\star\|_\mathsf{F}^2 &= \frac{1}{2} \left\|\mathrm{vec}\left(\mbf{\Sigma}_{L:1} - \mbf{\Sigma}_\star\right)\right\|_2^2 \\&= \frac{1}{2} \| \underbrace{\left(\mbf{\Sigma}^\top_{\ell-1:1} \otimes \mbf{\Sigma}_{L:\ell+1} \right)}_{\eqqcolon \mbf{A}_{\ell}}\cdot\mathrm{vec}(\mbf{\Sigma}_{\ell}) - \mathrm{vec}(\mbf{\Sigma}_\star) \|_2^2. 
    \end{align*}
    Then, the gradient with respect to $\mathrm{vec}(\mbf{\sigma}_{\ell})$ is given by
    \begin{align*}
        \nabla_{\mathrm{vec}(\mbf{\Sigma}_{\ell})} f(\mbf{\Theta}) = \mbf{A}_{\ell}^\top \left( \mbf{A}_{\ell}\cdot \mathrm{vec}(\mbf{\Sigma}_{\ell}) - \mathrm{vec}(\mbf{\Sigma}_\star)\right).
    \end{align*}
    Now, we can consider each block of the overall Hessian matrix. Let $\mbf{H} \in \mbb{R}^{d^2L \times d^2 L}$ denote the overall Hessian matrix, with block entries
    \begin{align*}
        \mbf{H} =
        \begin{bmatrix}
            \mbf{H}_{1, 1} & \mbf{H}_{1, 2} & \ldots & \mbf{H}_{1, L} \\
            \mbf{H}_{2, 1} & \mbf{H}_{2, 2} & \ldots & \mbf{H}_{2, L} \\
            \vdots & \vdots & \ddots & \vdots \\
             \mbf{H}_{L, 1} & \mbf{H}_{L, 2} & \ldots & \mbf{H}_{L, L}
        \end{bmatrix},
        \quad\, \text{where } \quad [\mbf{H}]_{m, \ell} \eqqcolon \mbf{H}_{m, \ell} \in \mbb{R}^{d^2 \times d^2}.
    \end{align*}
    Then, for $m=\ell$, we have
    \begin{align*}
        \mbf{H}_{\ell, \ell} = \nabla^2_{\mathrm{vec}(\mbf{W}_{\ell})} f(\mbf{\Theta}) &= \mbf{A}_{\ell}^{\top}\mbf{A}_{\ell}. 
    \end{align*}
For $m\neq l$, we have
\begin{align*}
   & \mbf{H}_{m, \ell} = \nabla_{\mathrm{vec}(\mbf{\Sigma}_{m})}  \nabla_{\mathrm{vec}(\mbf{\Sigma}_{\ell})} f(\mbf{\Theta}) =  \nabla_{\mathrm{vec}(\mbf{\Sigma}_{m})} \left[\mbf{A}_{\ell}^\top (\mbf{A}_{\ell} \mathrm{vec}(\mbf{W}_{\ell}) - \mathrm{vec}(\mbf{M}^{\star})) \right] \\
   & = \nabla_{\mathrm{vec}(\mbf{\Sigma}_{m})} \mbf{A}_{\ell}^\top \cdot \underbrace{(\mbf{A}_\ell \mathrm{vec}(\mbf{W}_{\ell}) - \mathrm{vec}(\mbf{M}^{\star}))}_{=0 \text{ 
 at convergence}} + \mbf{A}_{\ell}^{\top} \cdot  \nabla_{\mathrm{vec}(\mbf{\Sigma}_{m})} (\mbf{A}_{\ell} \mathrm{vec}(\mbf{W}_{\ell}) - \mathrm{vec}(\mbf{M}^{\star})) \\
   & = \mbf{A}_{\ell}^\top \mbf{A}_{m},
\end{align*}
where we have used the product rule along with the fact that $\mbf{A}_{\ell} \mathrm{vec}(\mbf{W}_{\ell}) = \mbf{A}_m \mathrm{vec}(\mbf{W}_{m})$.

Overall, the Hessian at convergence for GD is given by
\begin{align*}
    \mbf{H} =
    \begin{bmatrix}
        \mbf{A}_{1}^\top \mbf{A}_{1} & \mbf{A}_{1}^\top \mbf{A}_{2} & \ldots & \mbf{A}_{1}^\top \mbf{A}_{L} \\
        \mbf{A}_{2}^\top \mbf{A}_{1} & \mbf{A}_{2}^\top \mbf{A}_{2} & \ldots & \mbf{A}_{2}^\top \mbf{A}_{L} \\
        \vdots & \vdots & \ddots & \vdots \\
        \mbf{A}_{L}^\top \mbf{A}_{1} & \mbf{A}_{L}^\top \mbf{A}_{2} & \ldots & \mbf{A}_{L}^\top \mbf{A}_{L}
    \end{bmatrix}
\end{align*}
Now, we can derive an explicit expression for each $\mbf{A}_{m, \ell}$ by considering the implicit balancing effect of GD in Lemma~\ref{lemma:balancing}. Under balancing and Proposition~\ref{prop:one_zero_svs_set}, we have that at convergence,
    \begin{align*}
        \mbf{\Sigma}_{L:1} = \mbf{\Sigma}_\star \implies \mbf{\Sigma}_{\ell} = \begin{bmatrix}
            \mbf{\Sigma}^{1/L}_{\star, r} & \mbf{0} \\
            \mbf{0} & \alpha \cdot \mbf{I}_{d-r}
        \end{bmatrix}, \quad \forall \ell \in [L-1], \quad \text{and} \,\,\, \mbf{\Sigma}_L = \mbf{\Sigma}^{1/L}_{\star}.
    \end{align*}
    Thus, we have
    \begin{align*}
        \mbf{H}_{m, \ell} = \begin{cases}
            \mbf{\Sigma}_{\ell}^{2(\ell -1)} \otimes \mbf{\Sigma}_{\star}^{\frac{2(L-\ell)}{L}} \quad& \text{for } \,m=\ell, \\
            \mbf{\Sigma}_\ell^{m+\ell - 2} \otimes \mbf{\Sigma}_{\star}^{2L -m-\ell} \quad& \text{for }\, m\neq\ell. \\
        \end{cases}
    \end{align*}
        Now, we are left with computing the eigenvalues of $\mbf{H} \in \mbb{R}^{d^2 L \times d^2 L}$. To do this, let us block diagonalize $\mbf{H}$ into $\mbf{H} = \mbf{PCP}^\top$, where $\mbf{P}$ is a permutation matrix and 
    \begin{align*}
        \mbf{C} = 
        \begin{bmatrix}
            \mbf{C}_{1} & & \\
            & \ddots & \\
            &&\mbf{C}_{d^2}
        \end{bmatrix} \in \mbb{R}^{d^2 L \times d^2 L},
    \end{align*}
    where each $(i,j)$-th entry of $\mbf{C}_k \in \mbb{R}^{L \times L}$ is the $k$-th diagonal element of $\mbf{H}_{i, j}$. Since $\mbf{C}$ and $\mbf{H}$ are similar matrices, they have the same eigenvalues.
    Then, since $\mbf{C}$ is a block diagonal matrix, its eigenvalues (and hence the eigenvalues of $\mbf{H}$) are the union of each of the eigenvalues of its blocks. 

    By observing the structure of $\mbf{H}_{m, \ell}$, notice that each $\mbf{C}_k$ is a rank-$1$ matrix. Hence, when considering the top-$r$ diagonal elements of $\mbf{H}_{m, \ell}$ corresponding to each Kronecker product to construct $\mbf{C}_k$, each $\mbf{C}_k$ can be written as an outer product $\mbf{uu}^{\top}$, where $\mbf{u} \in \mbb{R}^L$ is
    \begin{align}
        \mbf{u}^{\top} = \begin{bmatrix}
            \sigma_{\star, i}^{1 - \frac{1}{L}} \sigma_{\star, j}^{0} & \sigma_{\star, i}^{1 - \frac{2}{L}} \sigma_{\star, j}^{\frac{1}{L}} & \sigma_{\star, i}^{1 - \frac{3}{L}} \sigma_{\star, j}^{\frac{2}{L}} & \ldots & \sigma_{\star, i}^{0} \sigma_{\star, j}^{1 - \frac{1}{L}} 
        \end{bmatrix}^{\top}.
    \end{align}
    Then, the non-zero eigenvalue of this rank-$1$ matrix is simply $\|\mbf{u}\|_2^2$, which simplifies to 
    \begin{align*}
        \|\mbf{u}\|_2^2 = \sum_{\ell=0}^{L-1} \left(\sigma_{\star, i}^{1-\frac{1}{L} - \frac{1}{L}\ell} \cdot \sigma_{\star, j}^{\frac{1}{L}\ell}\right)^2.
    \end{align*}
    Next, we can consider the remaining $d-r$ components of each Kronecker product of $\mbf{H}_{m, \ell}$. Notice that for $m = \ell = L$, we have
    \begin{align*}
        \mbf{H}_{L, L} = \begin{bmatrix}
            \sigma_{\star, 1}^{\frac{2(L-1)}{L}} \cdot \mbf{I}_d & & & \\
            & \ddots & & \\
            & & \sigma_{\star, r}^{\frac{2(L-1)}{L}} \cdot \mbf{I}_d  & \\
            & & & \alpha^{2(L-1)}\mbf{I}_{d-r} \otimes \mbf{I}_d
        \end{bmatrix}. 
    \end{align*}
    This amounts to a matrix $\mbf{C}_k$ with a single element  $\sigma_{\star, i}^{\frac{2(L-1)}{L}}$ and $0$ elsewhere. This gives an eigenvalue $\sigma_{\star, i}^{\frac{2(L-1)}{L}}$  for all $i \in [r]$, with multiplicity $d-r$. 

    Lastly, we can consider the diagonal components of $\mbf{H}_{m, \ell}$ that is a function of the initialization scale $\alpha$. For this case, each $\mbf{C}_k$ can be written as an outer product $\mbf{vv}^{\top}$, where 
    \begin{align}
        \mbf{v}^{\top} = \begin{bmatrix}
            \sigma_{\star, i}^{1 - \frac{1}{L}} \alpha^{0} & \sigma_{\star, i}^{1 - \frac{2}{L}} \alpha& \sigma_{\star, i}^{1 - \frac{3}{L}} \alpha^{2} & \ldots & \sigma_{\star, i}^{0} \alpha^{L-1}
        \end{bmatrix}^{\top}.
    \end{align}
    Similarly, the non-zero eigenvalue is simply $\|\mbf{v}\|_2^2$, which corresponds to
    \begin{align*}
        \|\mbf{v}\|_2^2 = \sum_{\ell=0}^{L-1} \left(\sigma_{\star, k}^{1-\frac{1}{L} - \frac{1}{L}\ell} \cdot \alpha^{\ell}\right)^2.
    \end{align*}
    This completes the proof.
\end{proof}

\begin{manuallemmainner}[Balancing]
    Suppose we run GD on the deep matrix factorization loss in Equation~(\ref{eqn:deep_mf}) with learning rate $\eta < \frac{2\sqrt{2}}{L \sigma^{2-\frac{2}{L}}_{\star,1}}$, where $\sigma_{\star, 1}$ is the first singular value of $\mbf{M}_\star \in \mbb{R}^{d\times d}$. Let $\sigma_{i,\ell}$ denote the $i$-th singular value of the $\ell$-th layer matrix.  If the initialization scale $\alpha$ satisfies
    $0< \alpha < \left( \log\left( \frac{2\sqrt{2}}{\eta L \sigma_{\star, 1}^{2 - \frac{2}{L}}} \right) \cdot 2 \sigma_{\star, 1}^{\frac{4}{L}} \right)^{\frac{1}{4}}$,  we have $| \sigma^2_{i,L}(t+1) - \sigma^2_{i,\ell}(t+1)| < | \sigma^2_{i,L}(t) - \sigma^2_{i,\ell}(t)|$.  \label{lemm:balancing}
\end{manuallemmainner}

\begin{proof}
    From Proposition~\ref{prop:svs_set}, we can re-write the loss in terms of the singular values:
\begin{align}
    \frac{1}{2} \left\|\mbf{W}_{L:1}(t) - \mbf{M}^\star\right\|^2_{\mathsf{F}} = \frac{1}{2} \sum_{k=1}^r \left(\sigma_k(\mbf{\Sigma}_{L:1}(t)) - \sigma_{\star, k}\right)^2 = \sum_{k=1}^r \frac{1}{2} \left(\prod_{\ell=1}^L \sigma_{\ell, k} - \sigma_{\star, k} \right)^2.
\end{align}
We aim to prove that balancing occurs on each singular value scalar index $k$, and so we focus on the scalar loss 
\begin{align*}
    \frac{1}{2} \left(\prod_{\ell=1}^L \sigma_{\ell, k} - \sigma_{\star, k}  \right)^2 \eqqcolon \frac{1}{2} \left(\prod_{\ell=1}^L \sigma_{\ell} - \sigma_{\star}  \right)^2  ,
\end{align*}
and omit the dependency on $k$ for ease of exposition. Then, let us define the balancing dynamics between $\sigma_i$ and $\sigma_j$ as $b_{i,j}^{(t+1)} \coloneqq \left(\sigma_i^{(t+1)}\right)^2 - \left(\sigma_j^{(t+1)}\right)^2$ and $\pi^{(t)} \coloneqq \prod_{\ell=1}^L \sigma_{\ell}(t)$ for the product of singular values at iteration $t$.
We can simplify the balancing dynamics as follows:
% \begin{align*}
%     \pi^{(t+1)} = \prod_{i=1}^{L} \sigma_{i}^{(t+1)} 
%     &= \prod_{i=1}^{D} \left(\sigma_i^{(t)} - \eta \left(\pi^{(t)} - 1 \right)\frac{\pi^{(t)}}{\sigma_i^{(t)}} \right) \\
%     &= \pi^{(t)} \prod_{i=1}^{L} \left(1 - \eta \left(\pi^{(t)} - 1 \right) \frac{\pi^{(t)}}{\left(\sigma_i^{(t)}\right)^2}\right) \\
%     &= \pi^{(t)} + \sum_{m=1}^{L} \eta^m (1 - \pi^{(t)})^m \pi^{(t)} \sigma_m(\sigma^{(t)}).
% \end{align*}

% Defining  to be the balance,
% The dynamic of the balances then becomes:
\begin{align*}
    b_{i,j}^{(t+1)} &= \left(\sigma_i^{(t+1)}\right)^2 - \left(\sigma_j^{(t+1)}\right)^2 \\
    &= \left(\sigma_i^{(t)} - \eta\left(\pi^{(t)} - \sigma_{\star}\right)\frac{\pi^{(t)}}{\sigma_i^{(t)}}\right)^2 - \left(\sigma_j^{(t)} - \eta\left(\pi^{(t)} - \sigma_{\star}\right)\frac{\pi^{(t)}}{\sigma_j^{(t)}}\right)^2 \\
    &= \left(\sigma_i^{(t)}\right)^2 - \left(\sigma_j^{(t)}\right)^2 + \eta^2 \left(\pi^{(t)} - \sigma_{\star}\right)^2 \left(\frac{\left(\pi^{(t)}\right)^2}{\left(\sigma_i^{(t)}\right)^2} - \frac{\left(\pi^{(t)}\right)^2}{\left(\sigma_j^{(t)}\right)^2}\right) \\
    &= \left(\left(\sigma_i^{(t)}\right)^2 - \left(\sigma_j^{(t)}\right)^2 \right) \left( 1 - \eta^2 (\pi^{(t)} - \sigma_{\star})^2 \frac{\left(\pi^{(t)}\right)^2}{\left(\sigma_i^{(t)}\right)^2 \left(\sigma_j^{(t)}\right)^2} \right) \\
    &= b_{i,j}^{(t)} \left( 1 - \eta^2 (\pi^{(t)} - \sigma_{\star})^2 \frac{\left(\pi^{(t)}\right)^2}{\left(\sigma_i^{(t)}\right)^2 \left(\sigma_j^{(t)}\right)^2} \right).
\end{align*}
Then, in order to show that $ \left|b_{i,j}^{(t+1)}\right| < \left|b_{i,j}^{(t)}\right|$, we need to prove that
\begin{align*}
    \underbrace{\left | 1 - \eta^2 (\pi^{(t)} -\sigma_{\star} )^2 \frac{\left(\pi^{(t)}\right)^2}{\left(\sigma_i^{(t)}\right)^2 \left(\sigma_j^{(t)}\right)^2} \right|}_{\eqqcolon c(t)} < 1,
\end{align*}
 for all iterations $t$. Following \cite{kreisler2023gradient}, it is straightforward to show that analyzing $c(t)$ is equivalent to analyzing the gradient flow solution. To this end, we introduce  a definition called gradient flow solution sharpness (GFS sharpness) before we proceed.

\begin{definition}[GFS Sharpness]
    The GFS sharpness denoted by $\psi(x)$ is the sharpness achieved by the global minima which lies in the same GF trajectory of $x$ (i.e., $\|\nabla^2 L(z)\|$ such that $L(z)=0$ and $z = GF(x)$, where $GF(\cdot)$ denotes the gradient flow solution).
\end{definition}

\noindent Then, we complete the following two steps:
\begin{enumerate}[label=(\roman*)]
    \item We show that for all scalars $\sigma$ in the trajectory, if $\psi(\sigma)< \frac{2\sqrt{2}}{\eta}$ and $\sigma > 0$, then it holds that $\sum_{i=1}^{\min\{2,L-1\}} \frac{\eta^2 (\pi(\sigma) - \sigma_{\star} )^2 \pi^2(\sigma)}{\sigma_{L-i}^2 \sigma_{L}^2} \leq 2$, where $\pi(\sigma)$ denotes the product given the trajectory of all $\sigma_i$. This case is analyzed when  \(\pi(\sigma) \in [0,\sigma_{\star} ]\) and when $\pi(\sigma) > \sigma_{\star}$. 
    \item If $\sum_{i=1}^{\min\{2,L-1\}} \frac{\eta^2 (\pi(\sigma) - \sigma_{\star} )^2 \pi^2(\sigma)}{\sigma_{L-i}^2 \sigma_{L}^2} \leq 2$, then iterates become more balanced, i.e,  $|b_{i,j}^{(t+1)}| < |b_{i,j}^{(t)}|$. 
\end{enumerate}

\noindent We prove (i) in Lemma \ref{GFS-1} and (ii) in Lemma \ref{GFS-2}. Both of the proofs are originally from \cite{kreisler2023gradient}, which we adapted using our notation for ease of the reader. Then, in Lemma~\ref{GFS-3}, we show that for each $\sigma_\star$, as long as the initialization scale satisfies
\begin{align*}
    \alpha < \left( \log\left( \frac{2\sqrt{2}}{\eta L \sigma_{\star}^{2 - \frac{2}{L}}} \right) \cdot 2 \sigma_{\star}^{\frac{4}{L}} \right)^{\frac{1}{4}},
\end{align*}
then it holds that the GFS sharpness satisfies $\psi(\sigma) \leq \frac{2{\sqrt{2}}}{\eta}$, which is the necessary condition for balancing. Then, to satisfy this condition for all singular values $\sigma_{\star, i}$ for all $i \in [r]$, we need
\begin{align}
\label{eqn:balance_condition}
    \alpha < \left( \log\left( \frac{2\sqrt{2}}{\eta L \sigma_{\star, 1}^{2 - \frac{2}{L}}} \right) \cdot 2 \sigma_{\star, 1}^{\frac{4}{L}} \right)^{\frac{1}{4}} \implies \eta < \frac{2\sqrt{2}}{L \sigma_{\star, 1}^{2 - \frac{2}{L}}},
\end{align}
 for the validity of the initialization scale. Thus, as long as the conditions in Equation~(\ref{eqn:balance_condition}) hold, we will have balancing. This completes the proof. 
\end{proof}

\begin{manuallemmainner}
\label{GFS-1}
    If the GFS sharpness $\psi(\sigma) \leq \frac{2\sqrt{2}}{\eta}$ and $\sigma > 0$, then  $\sum_{i=1}^{\min\{2,L-1\}} \frac{\eta^2 (\pi(\sigma)-\sigma_{\star})^2 \pi^2(\sigma)}{\sigma_{[L-i]}^2 \sigma_{[D]}^2} \leq 2$.
\end{manuallemmainner}

\begin{proof}

We will consider two cases: (i) $\pi(\sigma) \in [0, \sigma_\star]$ and (ii) $\pi(\sigma) > \sigma_\star$.\\

\noindent \textbf{Case 1:} Let \(\sigma \in \mathbb{R}^D\) and consider the case where \(\pi(\sigma) \in [0,\sigma_{\star} ]\). Then, we have
\[
\sum_{i=1}^{\min\{2,L-1\}} \frac{\eta^2 (\pi(\sigma) - \sigma_{\star} )^2 \pi^2(\sigma)}{\sigma_{L-i}^2 \sigma_{L}^2 } 
\leq \frac{\eta^2 \pi^2(\sigma)}{\sigma_{L-i}^2 \sigma_{L}^2}.
\]
Our goal is to show that if \(\psi(\sigma) \leq \frac{2\sqrt{2}}{\eta}\) then 
\[
\sum_{i=1}^{\min\{2,L-1\}} \frac{\eta^2 (\pi(\sigma) - 1)^2 \pi^2(\sigma)}{\sigma_{L-i}^2 \sigma_{L}^2}  \leq \frac{\eta^2 \pi^2(\sigma)}{\sigma_{L-i}^2 \sigma_{L}^2}\leq 2.
\]

Since the GFS sharpness is constant for all the weights on the gradient flow (GF) trajectory by definition, we can focus on the singular values (or weights) at the global minima.
Consider $z = \mathrm{GF}(\sigma)$, the GF solution of $\sigma$. In Lemma \ref{gf-unbalanced}, we proved that GF preserves unbalancedness, such that $\sigma^2_{l} - \sigma^2_{m} = z^2_{l} - z^2_{m}$ for all layers. Hence, it is sufficient to show that $\sum_{i=1}^{\min\{2,L-1\}} \frac{\eta^2 \pi(z)^2}{z_{L-i}^2 z_{L}^2} \leq 2$ in order to ensure $\sum_{i=1}^{\min\{2,L-1\}} \frac{\eta^2 \pi^2(\sigma)}{\sigma_{L-i}^2 \sigma_{L}^2} \leq 2$. Note that $\pi(z)=\sigma_{\star}$, since it lies on the global minima. Then,
\begin{align}
    \sum_{i=1}^{\min\{2,L-1\}} \frac{\eta^2 \pi^2(z)}{z^{2}_{L-i} z^2_{L}} 
= \sum_{i=1}^{\min\{2,L-1\}} \frac{\eta^2 \sigma^2_{\star}}{z^{2}_{L-i} z^2_{L}}.
\end{align}
From Lemma~\ref{1d-sharp}, we know that the sharpness at the global minima is given as
\begin{align}
\label{eqn:helper1}
\psi(\sigma)=\left\| \nabla^2 L(z) \right\| = \sum_{i=1}^{L} \frac{ \sigma^2_{\star}}{z_i^2}.
\end{align}
This immediately implies that \(\frac{\sigma^2_{\star}}{z^2_{L}} \leq \psi(\sigma)\) and equivalently, \(\exists \alpha \in [0,1]\) such that $\frac{\sigma^2_{\star}}{z^2_{L}} = \alpha \psi(\sigma)$.
Therefore, we have
\begin{align}
\label{eqn:helper2}
    \sum_{i=1}^{\min\{2,L-1\}} \frac{\sigma^2_{\star}}{z^2_{L-i}} \leq (1 - \alpha) \psi(\sigma).
\end{align}
Substituting Equations~(\ref{eqn:helper1}) and~(\ref{eqn:helper2}) into the expression we aim to bound, we obtain

\[
\sum_{i=1}^{\min\{2,L-1\}} \frac{\eta^2 (\pi(\sigma) - \sigma^2_{\star})^2 \pi^2(\sigma)}{\sigma_{L-i}^2 \sigma_{L}^2}
= \sum_{i=1}^{\min\{2,L-1\}} \frac{\eta^2 \sigma^2_{\star}}{z^{2}_{L-i} z^2_{L}} 
\leq \eta^2 \alpha (1 - \alpha) \psi^2(\sigma) \leq \frac{\eta^2}{4} \psi^2(\sigma) \leq 2,
\]
where we used the fact that the maximum of $\alpha(1-\alpha) $ is $\frac{1}{4}$ when \(\alpha = \frac{1}{2}\) and \(\psi(\sigma) \leq \frac{2\sqrt{2}}{\eta}\).
Thus, if \(\psi(\sigma) \leq \frac{2\sqrt{2}}{\eta}\), then for every weight $\sigma$ lying on its GF trajectory, we have
\begin{align*}
    \sum_{i=1}^{\min\{2,L-1\}} \frac{\eta^2 (\pi(\sigma) - \sigma_{\star})^2 \pi^2(\sigma)}{\sigma_{L-i}^2 \sigma_{L}^2} \leq 2.
\end{align*}

\noindent \textbf{Case 2:} Consider the case in which $\pi(\sigma) > \sigma_{\star}$. We already have that $\sigma>0$ throughout the trajectory (refer to Lemma 3.11 in \cite{kreisler2023gradient}) and so  $\pi(\sigma)>0$. Since, $\sigma>0$ throughout, we have
\begin{align*}
    \sigma_{i}-\eta (\pi(\sigma_{i}) - \sigma_{\star})\pi(\sigma_{i}) \frac{1}{\sigma_{i}} >0.
\end{align*}
Notice that this is just the next GD update from $\sigma_{i}$. 
From this, we get 
\begin{align*}
  1>  \frac{\eta (\pi(\sigma_{i}) - \sigma_{\star})\pi(\sigma_{i})}{\sigma^2_{i}}>0,
\end{align*}
which implies $\sum_{i=1}^{\min\{2,L-1\}} \frac{\eta^2 (\pi(\sigma) - \sigma_{\star})^2 \pi^2(\sigma)}{\sigma_{L-i}^2 \sigma_{L}^2} \leq 2$. This completes the proof.
\end{proof}

\begin{manuallemmainner}
\label{GFS-2}
    If $\sum_{i=1}^{\min\{2,L-1\}} \frac{\eta^2 (\pi(\sigma) - \sigma_{\star})^2 \pi^2(\sigma)}{\sigma_{L-i}^2 \sigma_{L}^2} \leq 2$, then $ \left|b_{i,j}^{(t+1)}\right| \leq \left|b_{i,j}^{(t)}\right|$ for $i,j \in [L]$.
\end{manuallemmainner}

\begin{proof}

Recall that the condition for balancing was given by
\begin{align}
\label{balance}
 b_{i,j}^{(t+1)}  = b_{i,j}^{(t)} \left( 1 - \eta^2 (\pi^{(t)} - \sigma_{\star})^2 \frac{\pi^{(t)2}}{\left(\sigma_i^{(t)}\right)^2 \left(\sigma_j^{(t)}\right)^2} \right).
\end{align}
WLOG, suppose that the $\sigma$ are sorted such that $\sigma_1 \geq \sigma_2 \geq \ldots \geq \sigma_L$. We know that  $$\sum_{i=1}^{\min\{2,L-1\}} \frac{\eta^2 (\pi(\sigma) - \sigma_{\star})^2 \pi^2(\sigma)}{\sigma_{L-i}^2 \sigma_{L}^2} \leq 2,$$ 
which implies 
\begin{align}
        \frac{\eta^2 (\pi(\sigma) - \sigma_{\star})^2 \pi^2(\sigma)}{\sigma_{L-1}^2 \sigma_{L}^2} < 2 \quad \text{and} \quad 
        \frac{\eta^2 (\pi(\sigma) - \sigma_{\star})^2 \pi^2(\sigma)}{\sigma_{i}^2 \sigma_{j}^2} < 1,
\end{align}
for all $i \in [L]$, $j \in [L-2] $ and $ i < j$. Notice that the latter inequality comes from the fact that 
\begin{align*}
    \frac{\eta^2 (\pi(\sigma) - \sigma_{\star})^2 \pi^2(\sigma)}{\sigma_{L-2}^2 \sigma_{L}^2} + \frac{\eta^2 (\pi(\sigma) - \sigma_{\star})^2 \pi^2(\sigma)}{\sigma_{L-2}^2 \sigma_{L}^2} &< \frac{\eta^2 (\pi(\sigma) - \sigma_{\star})^2 \pi^2(\sigma)}{\sigma_{L-1}^2 \sigma_{L}^2} + \frac{\eta^2 (\pi(\sigma) - \sigma_{\star})^2 \pi^2(\sigma)}{\sigma_{L-2}^2 \sigma_{L}^2} \\
    &< 2,
\end{align*}
which implies that
\begin{align*}
    2\frac{\eta^2 (\pi(\sigma) - \sigma_{\star})^2 \pi^2(\sigma)}{\sigma_{L-2}^2 \sigma_{L}^2} < 2 \implies \frac{\eta^2 (\pi(\sigma) - \sigma_{\star})^2 \pi^2(\sigma)}{\sigma_{L-2}^2 \sigma_{L}^2} < 1,
\end{align*}
and since $\sigma$ are sorted, it holds for all other $\sigma$.
Therefore from Equation~(\ref{balance}), we have for all $i \in [L-2]$,
\begin{align}
    b^{(t+1)}_{i,i+1} <  b^{(t)}_{i,i+1} \quad \text{and}\quad b^{(t+1)}_{L-2,L} <  b^{(t)}_{L-2,L}
    \quad \text{and} \quad -b^{(t)}_{L-1,L}  <b^{(t+1)}_{L-1,L} <  b^{(t)}_{L-1,L} .
\end{align}
%Now, we prove balancing considering two cases where $b^{(t+1)}_{L-1,L} \geq 0 $ and $b^{(t+1)}_{L-1,L} \leq 0 $. 
%First, consider the case $b^{(t+1)}_{L-1,L} \geq 0 $ then using the fact for all $i \in [L-2]$,
%$b^{(t+1)}_{i,i+1} <  b^{(t)}_{i,i+1}$, $b^{(t+1)}_{i,i+1} <  b^{(t)}_{i,i+1}$.
Then, notice that since we initialized all of the singular values $\sigma_\ell$ for $\ell \in [L-1]$ to be the same, they follow the same dynamics. Since we already showed that $|b^{(t+1)}_{L-1,L}| <  |b^{(t)}_{L-1,L}|$, it must follow that
\begin{align*}
    \left|b_{i,j}^{(t+1)}\right| \leq \left|b_{i,j}^{(t)}\right| \quad \text{for } \, i,j \in [L].
\end{align*}
This completes the proof.

%Hence we prove balancing for all $i,j \in [L]$, we have $ b_{i,j}^{(t+1)} \leq b_{i,j}^{(t)}$. 

%Now considering the case $b^{(t+1)}_{L-1,L} \leq 0 $, we will only obtain till $i \in [L-3]$, that $b^{(t+1)}_{i,i+1} <  b^{(t)}_{i,i+1}$ and $b^{(t+1)}_{L-2,L} <  b^{(t)}_{L-2,L} $
%Now considering the case $b^{(t+1)}_{L-1,L} \leq 0 $, we will only obtain till $i \in [L-3]$, that $b^{(t+1)}_{i,i+1} <  b^{(t)}_{i,i+1}$ and $b^{(t+1)}_{L-1,L} <  b^{(t)}_{L-1,L} $. This completes the proof. 
\end{proof}

\begin{manuallemmainner}
\label{GFS-3}
    Consider running GD with learning rate $\eta$ in Equation~(\ref{eqn:gd}) on the scalar loss 
    \begin{align*} 
        \mathcal{L}(\{\sigma_i\}_{i=1}^d)
 = \frac{1}{2} \left( \prod_{i=1}^L \sigma_{i} - \sigma_{\star} \right)^2,
    \end{align*} 
    with initialization
    $\sigma_{L}(0) = 0$ and $\sigma_{\ell}(0) = \alpha$ for all $\ell \in [L-1]$.
    If $\alpha < \left( \ln\left( \frac{2\sqrt{2}}{\eta L \sigma_{\star}^{2 - \frac{2}{L}}} \right) \cdot 2 \sigma_{\star}^{\frac{4}{L}} \right)^{\frac{1}{4}}$, then
    the GFS sharpness $\psi(\sigma) \leq \frac{2\sqrt{2}}{\eta}$.
\end{manuallemmainner}

\begin{proof}
    %We prove that the initialization set $\sigma_{L}(0) = 0$ and $\sigma_{\ell}(0) = \alpha$ for all $\ell \in [L-1]$ has a GFS sharpness $\psi(\sigma) \leq \frac{2\sqrt{2}}{\eta}$ if $\alpha \leq \log(\frac{2\sqrt{2}}{\eta}) $. This means that starting from this initialization the solution that GF finds will have sharpness less than $\frac{2\sqrt{2}}{\eta}$. For this initialization set, gradient descent with step-size $\eta$ will always balance in the next iterate. 

    %Note that at initialization $(L-1)$ iterates are equal. So, throughout the GD trajectory they are always equal, i.e, $\sigma_{L-1}(t) = \sigma_{L-2}(t)= \ldots= \sigma_{1}(t) \eqqcolon y$ for all t. Further by lemma \ref{balance}, $\sigma^{2}_{L}(t)-\sigma^{2}_{l}(t)=-\alpha^2$ for all $t$. 
    Since the singular values $\sigma_\ell$ for all $\ell \in [L-1]$ are initialized to $\alpha$, note that they all follow the same dynamics. Then, let us define 
    \begin{align*}
        y \coloneqq \sigma_1 = \ldots = \sigma_{L-1} \quad \text{and} \quad x \coloneqq \sigma_L.
    \end{align*}
    The gradient flow (GF) solution is the intersection between
    \begin{align*}
       xy^{L-1}=\sigma_{\star} \quad \text{and} \quad x^{2} - y^{2}= -\alpha^2,
    \end{align*}
    where the first condition comes from convergence and the second comes from the conservation flow law of GF which we prove in Lemma \ref{gf-unbalanced}.  
    Then, if we can find a solution at the intersection such that
    \begin{align*}
        (\hat{x}(\alpha),\hat{y}(\alpha)) = \begin{cases}
            xy^{L-1}=\sigma_{\star} \\
            x^{2} - y^{2}= -\alpha^2,
        \end{cases} 
    \end{align*}
    solely in terms of $\alpha$, then we can plug in $(\hat{x}(\alpha),\hat{y}(\alpha))$ into the GFS\footnote{Note that throughout the proof $(\hat{x}(\alpha),\hat{y}(\alpha))$ denotes the gradient flow solution as function of $\alpha$. It does
not refer to the GF trajectory.} from Lemma \ref{1d-sharp}
    \begin{align*}
        \psi(\hat{x}(\alpha),\hat{y}(\alpha)) 
 = \psi(\sigma) = \sum_{i=1}^{L} \frac{\sigma^2_{\star}}{\sigma^2_{i}} = \sigma^2_{\star}\left(\frac{1}{\hat{x}(\alpha)^2} + \frac{L-1}{\hat{y}(\alpha)^2}\right) \leq \frac{2\sqrt{2}}{\eta}
    \end{align*}
and solve to find an upper bound on $\alpha$. However, the intersection $(\hat{x}(\alpha),\hat{y}(\alpha))$ is a $2L$-th order polynomial in $\hat{y}(\alpha)$ which does not have a straightforward closed-form solution solely in terms of $\alpha$. Hence, we aim to find the upper bound on $\alpha$ by using a calculus of variations. By plugging in $x$, the solution $\hat{y}(\alpha)$ satisfies
\begin{align*}
    y^{2L} - \alpha^2 y^{2L-2} =  \sigma^2_{\star}.
\end{align*}
Then, by differentiating the relation with respect to $\alpha$, we obtain the following variational relation:
\begin{align}
   & 2L y^{2L-1}dy - \alpha^2 2 (L-1) y^{2L-3}dy - 2\alpha y^{2L-2} d\alpha = 0 \notag  \\ 
   & \implies y^{2L-3} (y^2 L - \alpha^2 (L-1)) dy = \alpha y^{2(L-1)} d\alpha \notag \\ \
   & \implies dy = \frac{y \alpha}{ (y^2 L -\alpha^2 (L-1))} d\alpha,
\end{align}
where we used the fact that $y^{2L-2} > 0 $ from Lemma~\ref{GFS-1} in the last line. Then, in order to have $\frac{dy}{d \alpha}>0$, we need $y > \sqrt{\frac{L-1}{L}} \alpha$, which is always true since $y > \alpha$ from initialization. Then, since $\alpha \to 0$, 
$\lim_{\alpha \rightarrow 0} \hat{y}(\alpha) = \sigma^{\frac{1}{L}}_{\star}$ and $\lim_{\alpha \rightarrow 0} \hat{x}(\alpha) = \sigma^{\frac{1}{L}}_{\star}$, as it corresponds to exact balancing. Hence, $\frac{dy}{d \alpha}>0$ implies as $\alpha$ increases from $0$, $\hat{y}(\alpha)$ would increase from $\sigma^{\frac{1}{L}}_{\star}$ and $\hat{y}(\alpha)$ is an increasing function of $\alpha$.
%Note that $\lim_{\alpha \rightarrow 0} \hat{y}(\alpha) = \sigma^{\frac{1}{L}}_{\star}$ and $\lim_{\alpha \rightarrow 0} \hat{x}(\alpha) = \sigma^{\frac{1}{L}}_{\star}$ , since $\alpha \rightarrow 0$ correspond to exact balancing. 
%So, $\frac{dy}{d \alpha}>0$ implies $y > \sqrt{\frac{L-1}{L}} \alpha$, which is always true since $y> \alpha$ as it is the intialization. So, $\frac{dy}{d \alpha}>0$, implies as $\alpha$ increases from $0$, $\hat{y}(\alpha)$ would increase from $\sigma^{\frac{1}{L}}_{\star}$. 
%So, $\hat{y}(\alpha)$ is an increasing function of $\alpha$. 
Similarly, the intersection at the global minima would satisfy the following relation for $ \hat{x}(\alpha)$:
\begin{align}
    & x^{(2+ \frac{2}{L-1})} + x^{\frac{2}{(L-1)}} \alpha^2 = \sigma^{\frac{2}{L-1}}_{\star} \notag \\ 
    & \implies \left(2+\frac{2}{L-1} \right) x^{1+ \frac{2}{L-1}}dx + \left(\frac{2}{L-1}\right)\alpha^2 x^{\frac{2}{L-1}-1} dx  + x^{\frac{2}{L-1}}(2\alpha d\alpha) = 0 \notag \\
    & \implies dx = \frac{-\alpha}{\left(\frac{L}{L-1}x + \frac{\alpha^2}{L-1}\frac{1}{x}\right)} d\alpha.
\end{align}

Note that since $x>0$, we will always have $\frac{dx}{d\alpha}<0$. Then, since $\lim_{\alpha \rightarrow 0} \hat{x}(\alpha) = \sigma^{\frac{1}{L}}_{\star}$,  $\frac{dx}{d\alpha}<0$ implies that as $\alpha$ increases, $\hat{x}(\alpha)$ would decrease from $\sigma^{\frac{1}{L}}_{\star}$.
Now, with the variational relations  $\frac{d\hat{x}}{d\alpha}$ and  $\frac{d \hat{y}}{d\alpha}$ in place, we aim to find $\frac{d \psi}{d \alpha}$:
\begin{align*}
   &  \Psi(\alpha) \coloneqq  \psi(\hat{x}(\alpha),\hat{y}(\alpha)) =  \sigma_{\star}^2 \left(\frac{1}{\hat{x}(\alpha)^2} + \frac{L-1}{\hat{y}(\alpha)^2} \right)  \\ 
   & \implies d \Psi = \sigma^2_{\star} \left(-\frac{2 }{\hat{x}^3} d\hat{x} - \frac{2 (L-1) }{\hat{y}^3}d\hat{y} \right)  \\ 
   & \implies d \Psi = \frac{1}{\hat{x}^3} \left[\frac{2 \alpha \sigma^2_{\star}}{\left(\frac{L}{L-1}\right)\hat{x} +\left(\frac{\alpha^2}{L-1}\right)\frac{1}{\hat{x}} } \right] d\alpha 
   - \left[\frac{(L-1)}{\hat{y}^3} \frac{2 \alpha \hat{y} \sigma^2_{\star}}{(\hat{y}^2L - \alpha^2 (L-1))} \right] d \alpha \\
   & \implies d \Psi = \left [\frac{1}{\hat{x}^4 + \frac{\alpha^2}{L}\hat{x}^2 } - \frac{1}{(\hat{y}^4 - \alpha^2 \hat{y}^2\frac{(L-1)}{L})} \right] 2 \frac{(L-1)\sigma^2_{\star}}{L} \alpha d \alpha \\
   & \implies d \Psi  = G(\alpha) d\alpha,
\end{align*}
where we defined $G(\alpha) \coloneqq \left [\frac{1}{\hat{x}^4 + \frac{\alpha^2}{L}\hat{x}^2 } - \frac{1}{(\hat{y}^4 - \alpha^2 \hat{y}^2\frac{(L-1)}{L})} \right] 2 \frac{(L-1)\sigma^2_{\star}}{L} \alpha$ and used the notation $\hat{x} = \hat{x}(\alpha)$ and $\hat{y} = \hat{y}(\alpha)$ for simplicity. \\

\noindent Next, we will show the three following steps:
\begin{enumerate}[label=(\roman*)]
    \item Prove that $G(\alpha) > 0$ for all $\alpha > 0$ to show that the sharpness $\Psi(\alpha)$ is an increasing function of $\alpha$.
    \item Solve the differential $d\Psi$ to find the relationship between $d\Psi$ and $\Psi(\alpha)$.
    \item Find an upper bound on a part of $\frac{d\Psi}{\Psi(\alpha)}$ found in Step 2.
\end{enumerate}
These series of steps comes from the fact that the intersection does not have a closed-form solution. The goal is to find a function in which we can upper bound $\frac{d\Psi}{\Psi(\alpha)}$ with a function with a closed-form solution to find a bound on $\alpha$ such that the sharpness $\psi(\alpha) \leq \frac{2\sqrt{2}}{\eta}$. \\

% \ag{There are a few steps to go from here. }

% \begin{enumerate}
%     \item Show that  $ G(\hat{x}(\alpha),\hat{y}(\alpha),\alpha)$ is always positive, meaning sharpness increases as $\alpha$ increases. This is true since we already proved balanced iterates have the least sharpness. 
%     \item Find an upper bound on $ G(\hat{x}(\alpha),\hat{y}(\alpha),\alpha)$ (say $H(\alpha)$), so that the PDE $d \Psi  = H(\alpha) d\alpha$ has a known closed form solution (since we know initial condition). 
%     \item By continuity, the solution of PDE $d \Psi  = H(\alpha) d\alpha$ will always be above the curve $d \Psi  = G(\hat{x}(\alpha),\hat{y}(\alpha),\alpha) d\alpha$. 
%     \item Since both are increasing function and $d \Psi  = H(\alpha) d\alpha$ is an upper bound on $d \Psi  = G(\hat{x}(\alpha),\hat{y}(\alpha),\alpha) d\alpha$, the initialization condition found by solving $d \Psi  = H(\alpha) d\alpha$ would be also true for the original PDE. 
% \end{enumerate}

\noindent \textbf{Step 1}: \underline{Prove $ G(\alpha)>0 $ to show sharpness $ \Psi(\alpha)$ is an increasing function of $\alpha$}. \\

\noindent There have been several lines of work such as those by \cite{kreisler2023gradient} and \cite{marion2024deep} which showed that GD would decrease the sharpness of the solution. The more balanced the solution (which corresponds to smaller $\alpha$), the smaller the sharpness. We prove this again here:
\begin{align*}
    G(\alpha) > 0 
    & \implies \hat{y}^4 - \alpha^2 \hat{y}^2\frac{(L-1)}{L} > \hat{x}^4 + \frac{\alpha^2}{L}\hat{x}^2 \\
    & \implies (\hat{y}^4  - \hat{x}^4) > \alpha^2 \left(\frac{1}{L}\hat{x}^2 + \hat{y}^2\frac{(L-1)}{L}\right) \\
    &  \implies \underbrace{(\hat{y}^2  - \hat{x}^2)}_{=\alpha^2}(\hat{y}^2  + \hat{x}^2) > \alpha^2 \left(\frac{1}{L}\hat{x}^2 + \hat{y}^2\frac{(L-1)}{L}\right) \\
    & \implies  \hat{x}^2 (1- \frac{1}{L}) + \hat{y}^2\frac{1}{L} >0,
\end{align*}
where the last inequality always holds since we have $L>2$. This proves that $\Psi$ is an increasing function of $\alpha$ since for  $d \Psi  = G(\alpha) d\alpha$, as it always holds that $ G(\alpha) >0$ for any $L>2$ and $\alpha > 0$. \\

\begin{figure}
    \centering
    \includegraphics[width=0.5\linewidth]{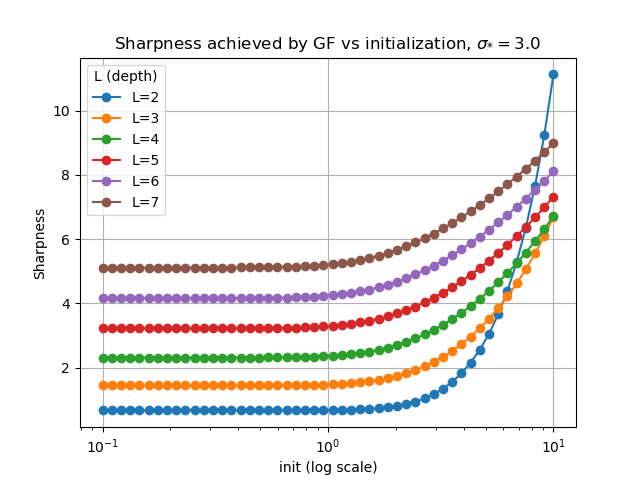}
    \caption{Sharpness $\Psi(\alpha)$ as a function of initialization $\alpha$. The theoretical approximation bound $ \Psi = \Psi_{0} \exp\left( \frac{ \left(\frac{1}{L} - \frac{1}{L^2}\right)}{2\sigma_{\star}^{\frac{4}{L}}} \alpha^4 \right)$ serves as proxy upper bound to this increasing function.  }
    \label{fig:sharp-init}
\end{figure}

\noindent \textbf{Step 2}: \underline{Solve the differential to establish the relation between $\Psi(\alpha)$ and $\alpha$}. \\

\noindent Rewriting the expression for sharpness and establishing an equation we have
\begin{align}
    \Psi(\alpha) = \sigma_{\star}^2 \left(\frac{1}{\hat{x}(\alpha)^2} + \frac{L-1}{\hat{y}(\alpha)^2} \right) 
    & \implies  \Psi(\alpha) = \sigma_{\star}^2 \left(\frac{\hat{y}^2 + (L-1)\hat{x}^2}{\hat{x}^2\hat{y}^2} \right)\\ 
    & \implies \frac{\hat{y}^2}{L} + \left(1-\frac{1}{L} \right) \hat{x}^2 = \frac{\Psi(\alpha) \hat{x}^2 \hat{y}^2}{L \sigma_{\star}^2}. \label{mid-eq}
\end{align}
Now, we revisit the original differential between $\Psi(\alpha)$ and $\alpha$:
\begin{align}
   &  d \Psi  = \left [\frac{1}{(\hat{x}^4 + \frac{\alpha^2}{L}\hat{x}^2 )} - \frac{1}{(\hat{y}^4 - \alpha^2 \hat{y}^2\frac{(L-1)}{L})} \right] 2 \frac{(L-1)\sigma^2_{\star}}{L} \alpha d\alpha \notag \\
   & \implies d \Psi = \frac{\hat{y}^4 - \hat{x}^4 -\alpha^2 (\frac{\hat{x}^2}{L} + (1-\frac{1}{L}\hat{y}^2 )) }{(\hat{x}^4 + \frac{\alpha^2}{L}\hat{x}^2 )(\hat{y}^4 - \alpha^2 \hat{y}^2\frac{(L-1)}{L}) } 2 \left(1-\frac{1}{L} \right) \sigma^2_{\star} \alpha d \alpha \notag \\
   &  \implies   d \Psi =   \frac{\alpha^2  \left( \frac{\hat{y}^2}{L} + (1-\frac{1}{L})\hat{x}^2\right) }{(\hat{x}^4 + \frac{\alpha^2}{L}\hat{x}^2 )(\hat{y}^4 - \alpha^2 \hat{y}^2\frac{(L-1)}{L}) } 2 \left(1-\frac{1}{L}\right) \sigma^2_{\star} \alpha d \alpha    \label{mid-eq2}   
\end{align}
Using the expression for $  \frac{\hat{y}^2}{L} + (1-\frac{1}{L})\hat{x}^2$ derived in Equation~(\ref{mid-eq}) and plugging it into Equation~(\ref{mid-eq2}), we obtain
\begin{align}
    &    d \Psi = \frac{\alpha^2 \left( \frac{\Psi(\alpha) \hat{x}^2 \hat{y}^2}{L \sigma_{\star}^2} \right)}{(\hat{x}^4 + \frac{\alpha^2}{L}\hat{x}^2)(\hat{y}^4 - \alpha^2 \hat{y}^2 \frac{(L-1)}{L})} 2 \left(1-\frac{1}{L}\right) \sigma_{\star}^2 \alpha \, d \alpha \notag \\
    & \implies \frac{d \Psi }{\Psi(\alpha)} =   \frac{2}{(\hat{x}^2 + \frac{\alpha^2}{L})(\hat{y}^2 - \alpha^2\frac{(L-1)}{L})}    \left(\frac{1}{L} - \frac{1}{L^2} \right)\alpha^{3} d \alpha \notag  \\ 
    & \implies \frac{d \Psi }{\Psi(\alpha)} =   \frac{2}{(\hat{x}^2 + \frac{\alpha^2}{L} )^2 }    \left(\frac{1}{L} - \frac{1}{L^2} \right)\alpha^{3} d \alpha  \\
    & \implies \frac{d \Psi }{\Psi(\alpha)} = P(\alpha) \alpha^3 d\alpha,
\end{align}
where we have defined $P(\alpha) \coloneqq \frac{2}{(\hat{x}^2 + \frac{\alpha^2}{L} )^2 }    \left(\frac{1}{L} - \frac{1}{L^2} \right)$.

\noindent Solving the differential $ \frac{d \Psi }{\Psi(\alpha)} = P(\alpha) \alpha^{3}d\alpha$ in exact closed-form is difficult since $\hat{x}$ is also an function of $\alpha$. However, in Step 1, we proved that $\Psi(\alpha)$ is an increasing function of $\alpha$, and so instead of solving exactly, we can find a differential equation $ \frac{d \Psi }{\Psi(\alpha)} = F(\alpha) \alpha^{3} d\alpha$ with $F(\alpha)> P(\alpha) $ such that $F(\alpha)$ is more increasing, and use it to solve the PDE instead.
Though, note that the initialization limit on $\alpha$ that would be found after solving the surrogate PDE $ \frac{d \Psi }{\Psi(\alpha)} = F(\alpha)\alpha^{3} d\alpha$ would be smaller than the $\alpha$ if it was found using the original PDE $ \frac{d \Psi }{\Psi(\alpha)} = P(\alpha)\alpha^{3} d\alpha$. \\

\begin{figure}
    \centering
    \includegraphics[width=0.5\linewidth]{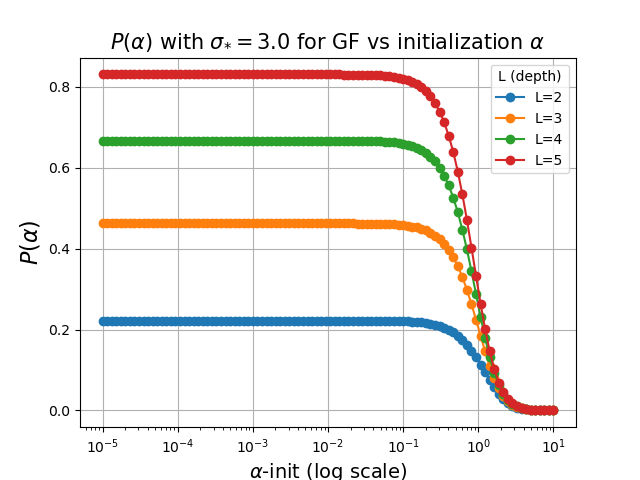}
    \caption{$P(\alpha)$ is a decreasing function of $\alpha$ for Gradient Flow. So $F(\alpha)= \lim_{\alpha \rightarrow 0} P(\alpha)$ is used for the bound in the integral. }
    \label{fig:P-var}
\end{figure}

\noindent \textbf{Step 3}: \underline{Finding an upper bound function and solving for initialization}. \\
\smk{TODO: proofread here onwards}
\noindent Note that the original coefficient in $ \frac{d \Psi }{\Psi(\alpha)} = P(\alpha)\alpha^{3} d\alpha$ is of the form
\begin{align*}
    P(\alpha)  = \frac{2}{(\hat{x}^2 + \frac{\alpha^2}{L})^2 }    \left(\frac{1}{L} - \frac{1}{L^2}\right)
\end{align*}
Let's consider the two corner cases for $\alpha$. We showed before that $\lim_{\alpha \rightarrow 0} \hat{x}(\alpha) = \sigma^{\frac{1}{L}}_{\star}$, so \[
\lim_{\alpha \rightarrow 0} P(\alpha) = \frac{2 \left(\frac{1}{L} - \frac{1}{L^2}\right)}{\sigma_{\star}^{\frac{4}{L}} }
\]
As $\alpha \rightarrow \infty $, we have $\lim_{\alpha \rightarrow \infty} P(\alpha) \rightarrow 0 $ since $\lim_{\alpha \rightarrow \infty} \hat{x} = 0$. Since, we have $P(\alpha)$ to be decreasing in $\alpha$ (Figure~\ref{fig:P-var}), we will use the largest value of $P(\alpha)$ as $F(\alpha)$ in upper bounding this increasing function. We have $\lim_{\alpha \rightarrow 0} P(\alpha) = \frac{2 \left(\frac{1}{L} - \frac{1}{L^2}\right)}{\sigma_{\star}^{\frac{4}{L}} }$, the integral of this upper bound gives us:
\begin{align*}
    & \int \frac{d \Psi}{\Psi} = \frac{2 \left(\frac{1}{L} - \frac{1}{L^2}\right)}{\sigma_{\star}^{\frac{4}{L}}} \int \alpha^3 \, d\alpha \\
    & \mathrm{ln}(\frac{\Psi}{\Psi_{0}}) = \frac{ \left(\frac{1}{L} - \frac{1}{L^2}\right)}{2\sigma_{\star}^{\frac{4}{L}}} (\alpha^4)
\end{align*}
where $\Psi_{0}= \lim_{\alpha \rightarrow 0}\Psi = L\sigma^{2-\frac{2}{L}}_{\star} $. So, we will have:

\begin{align*}
    \Psi = \Psi_{0} \exp\left( \frac{ \left(\frac{1}{L} - \frac{1}{L^2}\right)}{2\sigma_{\star}^{\frac{4}{L}}} \alpha^4 \right)
\end{align*}

We verify this upper bound empirically from Figure \ref{fig:sharp-init}, where we see a near exponential growth in sharpness as function of $\alpha$. The growth rate is smaller as depth $L$ increases, which is evident from this expression. 

So, in order to ensure that sharpness $\Psi< \frac{2\sqrt{2}}{\eta}$ to ensure balancing, we will require 

\begin{align*}
    \alpha < \left( \ln\left( \frac{\frac{2\sqrt{2}}{\eta}}{L \sigma_{\star}^{2 - \frac{2}{L}}} \right) \cdot \frac{2 \sigma_{\star}^{\frac{4}{L}}}{\left( \frac{1}{L} - \frac{1}{L^2} \right)} \right)^{\frac{1}{4}} < \left( \ln\left( \frac{2\sqrt{2}}{\eta L \sigma_{\star}^{2 - \frac{2}{L}}} \right) \cdot 2 \sigma_{\star}^{\frac{4}{L}} \right)^{\frac{1}{4}}.
\end{align*}

\end{proof}

\begin{manuallemmainner}
\label{gf-unbalanced}
    Consider the minimizing the loss         \begin{align*} 
        \mathcal{L}\left(\{\sigma_\ell\}_{\ell=1}^L\right)
 = \frac{1}{2} \left( \prod_{\ell=1}^L \sigma_{\ell} - \sigma_{\star} \right)^2,
    \end{align*}  
    using gradient flow. Then, the balancedness between two singular values defined by $\sigma^2_{ \ell} (t) - \sigma^2_{m} (t)$ for all $m, \ell \in [L]$ is constant for all $t$.
\end{manuallemmainner}

\begin{proof}
Notice that the result holds specifically for gradient flow and not descent. The dynamics of each scalar factor for gradient flow can be written as
    \begin{align*}
        \dot{\sigma}_{\ell}(t) = - \left(\prod_{\ell=1}^L \sigma_{ \ell} (t) - \sigma_{\star} \right)\cdot \prod_{i\neq \ell}^L \sigma_{i}(t)
    \end{align*}
Then, the time derivative of balancing is given as
\begin{align*}
  & \frac{\partial}{\partial t} (\sigma^2_{ \ell} (t) - \sigma^2_{m} (t)) = \sigma_{ \ell} (t)\dot{\sigma}_{\ell}(t)  - \sigma_{m} (t)\dot{\sigma}_{m}(t)  \\
  & = - \sigma_{ \ell} (t)\left(\prod_{\ell=1}^L \sigma_{ \ell} (t) - \sigma_{\star} \right)\cdot \prod_{i\neq \ell}^L \sigma_{i}(t) + \sigma_{m} (t)\left(\prod_{m=1}^L \sigma_{ \ell} (t) - \sigma_{\star} \right)\cdot \prod_{j\neq m}^L \sigma_{j}(t). \\
  & = 0.
\end{align*}
Hence, the quantity $\sigma^2_{ \ell} (t) - \sigma^2_{m} (t) $ remains constant for all time $t$, hence preserving unbalancedness. 
\end{proof}

\begin{manuallemmainner}
\label{1d-sharp}
    Consider the scalar loss     \begin{align*} 
        \mathcal{L}(\{\sigma_i\}_{i=1}^d)
 = \frac{1}{2} \left( \prod_{i=1}^L \sigma_{i} - \sigma_{\star} \right)^2,
    \end{align*}
    The sharpness at the global minima is given as $\| \nabla^2 \mathcal{L} \|_{2} = \sum_{i=1}^{L} \frac{\sigma^2_{\star}}{\sigma^2_{i}}$.
\end{manuallemmainner}

\begin{proof}
The gradient is given by
\begin{align*}
    \nabla_{\sigma_{i}}  \mathcal{L} = \left(\prod_{\ell=1}^L \sigma_{ \ell} (t) - \sigma_{\star} \right) \prod_{j\neq i}^L \sigma_{j}(t).
\end{align*}
Then, 
\begin{align*}
     \nabla_{\sigma_{j}}  \nabla_{\sigma_{i}}  \mathcal{L} =  \prod_{\ell\neq i}^L \sigma_{\ell}(t)  \prod_{\ell\neq j}^L \sigma_{\ell}(t) + \left(\prod_{\ell=1}^L \sigma_{ \ell} (t) - \sigma_{\star} \right)  \prod_{\ell\neq j, \ell \neq i}^L \sigma_{\ell}(t)
\end{align*}
 Let $\pi(t)=  \prod_{i=1}^L \sigma_{i}(t)$. Then, at the global minima, we have
\begin{align*}
     \nabla_{\sigma_{j}}  \nabla_{\sigma_{i}}  \mathcal{L} =  \frac{\pi^2}{\sigma_{i} \sigma_{j}} = \frac{\sigma_{\star}^2}{\sigma_{i} \sigma_{j}}
\end{align*}
Thus, the sharpness of the largest eigenvalue is given as $ \| \nabla^2 \mathcal{L} \|_{2} = \sum_{i=1}^{L} \frac{\sigma^2_{\star}}{\sigma^2_{i}}$. 
\end{proof}

\begin{manualtheoreminner}
[Stable Subspace Oscillations]
       Consider running GD on the deep matrix factorization loss in Equation~(\ref{eqn:deep_mf}) and denote the SVD of the target matrix as  $\mbf{M}_\star = \mbf{U}_\star\mbf{\Sigma}_\star\mbf{V}^\top_\star $, with distinct singular values $\sigma_{\star, 1} > \ldots > \sigma_{\star, r}$. Let $\Delta_i$  denote the $i$-th eigenvector of the Hessian with unit norm, $\lambda_{i}$ the corresponding eigenvalue after strict balancing occurs and denote $f_{\Delta_i}$ as the 1-D function at the cross section of the loss landscape and the line
following the direction of $\Delta_i$ passing the minima.
Then, if the minima of $f_{\Delta_i}$ satisfy $f_{\Delta_i}^{(3)}>0$ and $3[f_{\Delta_i}^{(3)}]^2 - f_{\Delta_i}^{(2)}f_{\Delta_i}^{(4)} > 0$, then 2-period orbit oscillation occurs in direction of $\Delta_i$ if $\eta>\frac{2}{\lambda_{i}}$. \label{thm:stable_sub}
\end{manualtheoreminner}
\begin{proof}
    First, we derive the eigenvectors of the Hessian of the training loss at convergence (i.e., $\mbf{M}_\star = \mbf{W}_{L:1}$).
    To obtain the eigenvectors of the Hessian of parameters $(\mbf{W}_L, \ldots, \mbf{W}_2, \mbf{W}_1)$, consider a small perturbation of the parameters:
    \begin{align*}
        \mbf{\Theta} \coloneqq \left(\Delta \mbf{W}_\ell +  \mbf{W}_\ell \right)_{\ell=1}^L =  (\mbf{W}_L + \Delta \mbf{W}_L, \ldots, \mbf{W}_2+ \Delta \mbf{W}_2, \mbf{W}_1+ \Delta \mbf{W}_1).
    \end{align*}

    Given that $\mbf{W}_{L:1} = \mbf{M}_\star$, consider and evaluate the loss function at this minima: 
    \begin{align}
        \mathcal{L}(\mbf{\Theta}) = \frac{1}{2} \biggl\| &\sum_{\ell} \mbf{W}_{L:\ell+1} \Delta \mbf{W}_\ell \mbf{W}_{\ell-1:1} \\
        &+ \sum_{\ell<m} \mbf{W}_{L:\ell+1} \Delta \mbf{W}_\ell \mbf{W}_{\ell-1:m+1} \Delta \mbf{W}_{m} \mbf{W}_{m-1:1}   +   \ldots   +  \Delta \mbf{W}_{L:1}\biggr\|^2_{\mathsf{F}}.
    \end{align}
    By expanding each of the terms and splitting by the orders of $\Delta \mbf{W}_\ell$ (perturbation), we get that the second-order term is equivalent to
    \begin{align*}
        \Theta&\left(\sum_{\ell=1}^L\|\Delta \mbf{W}_\ell\|^2\right): \,\, \frac{1}{2} \biggl\| \sum_{\ell} \mbf{W}_{L:\ell+1} \Delta \mbf{W}_\ell \mbf{W}_{\ell-1:1} \biggr\|^2_{\mathsf{F}} \\
        \Theta&\left(\sum_{\ell=1}^L\|\Delta \mbf{W}_\ell\|^3\right): \,\, \mathrm{tr}\left[\left(\sum_{\ell} \mbf{W}_{L:\ell+1} \Delta \mbf{W}_\ell \mbf{W}_{\ell-1:1} \right)^\top \left( \sum_{\ell<m} \mbf{W}_{L:\ell+1} \Delta \mbf{W}_\ell \mbf{W}_{\ell-1:m+1} \Delta \mbf{W}_{m} \mbf{W}_{m-1:1} \right)\right] \\
        \Theta&\left(\sum_{\ell=1}^L\|\Delta \mbf{W}_\ell\|^4\right): \,\, \frac{1}{2} \| \sum_{\ell<m} \mbf{W}_{L:\ell+1} \Delta \mbf{W}_\ell \mbf{W}_{\ell-1:m+1} \Delta \mbf{W}_{m} \mbf{W}_{m-1:1}\|^2_{\mathsf{F}}\\
        &+ \mathrm{tr}\left[\sum_{l} \left(\mbf{W}_{L:\ell+1}\Delta \mbf{W}_\ell \mbf{W}_{\ell-1:1} \right)^\top \left(\sum_{l<m<p} \mbf{W}_{L:\ell+1} \Delta \mbf{W}_\ell \mbf{W}_{\ell-1:m+1} \Delta \mbf{W}_{m} \mbf{W}_{m-1:p+1} \Delta \mbf{W}_{p} \mbf{W}_{p-1:1} \right)\right]
    \end{align*}

The direction of the steepest change in the loss at the minima correspond to the largest eigenvector direction of the Hessian. Since higher order terms such as $ \Theta\left(\sum_{\ell=1}^L\|\Delta \mbf{W}_\ell\|^3\right)$ are insignifcant compared to the second order terms $  \Theta\left(\sum_{\ell=1}^L\|\Delta \mbf{W}_\ell\|^2\right)$, finding the direction that maximizes the second order term leads to finding the eigenvector of the Hessian.
    Then, the eigenvector corresponding to the maximum eigenvalue of  $\nabla^2 \mathcal{L}$ is the solution of 
    \begin{align}
        \Delta_{1} \coloneqq \mathrm{vec}(\Delta \mbf{W}_L, \ldots \Delta \mbf{W}_1) = \underset{\|\Delta \mbf{W}_L\|^2_{\mathsf{F}} + \ldots + \|\Delta \mbf{W}_1\|^2_{\mathsf{F}} = 1}{\mathrm{arg max}} \, f\left(\Delta \mbf{W}_L, \ldots, \Delta \mbf{W}_1 \right),\label{max-eig}
    \end{align}
    where 
    \begin{align}
        f(\Delta \mbf{W}_L, \ldots, \Delta \mbf{W}_1) \coloneqq \frac{1}{2} \|\Delta \mbf{W}_L \mbf{W}_{L-1:1} + \ldots + \mbf{W}_{L:3}\Delta \mbf{W}_2 \mbf{W}_{1} + \mbf{W}_{L:2} \Delta \mbf{W}_1\|^2_{\mathsf{F}}.
    \end{align}

While the solution of Equation~(\ref{max-eig}) gives the maximum eigenvector direction of the Hessian, $\Delta_{1}$, the other eigenvectors can be found by solving
\begin{align}
    \Delta_{r} \coloneqq  \underset{
    \substack{
    \|\Delta \mbf{W}_L\|^2_{\mathsf{F}} + \ldots + \|\Delta \mbf{W}_1\|^2_{\mathsf{F}} = 1, \\
    \Delta_{r}\perp \Delta_{r-1},.., \Delta_{r}\perp \Delta_{1}
    }
    }{\mathrm{argmax}} \, f\left(\Delta \mbf{W}_L, \ldots, \Delta \mbf{W}_1 \right).\label{other-eig}
\end{align}

    By expanding $f(\cdot)$, %subject to the constraint ${\|\Delta \mbf{W}_L\|^2_{\mathsf{F}}} + \ldots + \|\Delta \mbf{W}_1\|^2_{\mathsf{F}} = 1$ ,
    we have that % we don't expand subject to a constraint
    \begin{align}
        f(\Delta \mbf{W}_L, &\ldots, \Delta \mbf{W}_1) = \|\Delta\mbf{W}_L \mbf{W}_{L-1:1}\|^2_{\mathsf{F}} +\ldots+ \|\mbf{W}_{L:3}\Delta \mbf{W}_2 \mbf{W}_{1}\|^2_{\mathsf{F}}  + \|\mbf{W}_{L:2} \Delta \mbf{W}_1\|^2_{\mathsf{F}} \notag \\
        &+ \mathrm{tr}\left[\left(\Delta\mbf{W}_L \mbf{W}_{L-1:1} \right)^\top \left(\mbf{W}_{L:3}\Delta \mbf{W}_2 \mbf{W}_{1} + \ldots +\mbf{W}_{L:2} \Delta \mbf{W}_1 \right)\right] + \ldots + \notag \\
        &\mathrm{tr}\left[\left(\mbf{W}_{L:2} \Delta \mbf{W}_1\right)^\top \left(\mbf{W}_{L:3}\Delta \mbf{W}_2 \mbf{W}_{1} + \ldots +\mbf{W}_{L:3}\Delta \mbf{W}_2 \mbf{W}_{1} \right)\right].     \label{expansion}
    \end{align}

We can solve Equation~(\ref{max-eig}) by maximizing each of the terms, which can be done in two steps:
\begin{enumerate}[label=(\roman*)]
\item 
Each Frobenius term in the expansion is maximized when the left singular vector of $\Delta \mbf{W}_{\ell}$ aligns with $\mbf{W}_{L:\ell+1}$ and the right singular vector aligns with $\mbf{W}_{\ell-1:1}$. This is a result of Von Neumann's trace inequality~\citep{mirsky1975trace}. Similarly, each term in the trace is maximized when the singular vector of the perturbations align with the products. 
\item Due to the alignment, Equation~(\ref{max-eig}) can be written in just the singular values. Let $\Delta s_{\ell, i}$ denote the $i$-th singular value of the perturbation matrix $\Delta\mbf{W}_\ell$. Recall that all of the singular values of $\mbf{M}_\star$ are distinct (i.e., $\sigma_{\star, 1} > \ldots>\sigma_{\star, r}$). Hence, it is easy to see that
Equation~(\ref{max-eig}) is maximized when $\Delta s_{\ell,i} = 0$ (i.e, all the weight goes to $\Delta s_{\ell,1}$). Thus, each perturbation matrix must be rank-$1$.
\end{enumerate}
Now since each perturbation is rank-$1$, we can write each perturbation as 
    \begin{align}
        \Delta\mbf{W}_{\ell} = \Delta s_{\ell} \Delta \mbf{u}_{\ell} \Delta\mbf{v}_\ell^\top, \quad \forall \ell \in [L],
    \end{align}
    % Then, notice that since the top-$r$ singular values of $\mbf{M}_\star$ are unique (i.e., $\sigma_{\star, 1} > \ldots > \sigma_{\star, r}$), the singular values of each $\mbf{W}_{\ell}$ are also unique, and hence the solution for each $\Delta\mbf{W}_{\ell}$ will be rank-$1$. We can express each solution as \
    for $\Delta s_{\ell} > 0$ and orthonormal vectors $\Delta \mbf{u}_{\ell} \in \mbb{R}^d$ and  $\Delta \mbf{v}_{\ell} \in \mbb{R}^d$ with $\sum_{\ell=1}^L \Delta s^2_{\ell} = 1$.
    Plugging this in each term, we obtain:
   \begin{align*}
        \|\mbf{W}_{L:\ell+1} \Delta_1 \mbf{W}_{\ell} \mbf{W}_{\ell-1:1}\|_2^2 = \Delta_1 s_\ell^2\cdot \biggl\|\underbrace{\mbf{V}_\star \mbf{\sigma}^{\frac{L-\ell}{L}}_\star \mbf{V}^\top_\star \Delta \mbf{u}_\ell}_{\eqqcolon \mbf{a}}\underbrace{ \Delta \mbf{v}_\ell^\top \mbf{V}_\star \mbf{\sigma}^{\frac{\ell-1}{L}}_\star \mbf{V}^\top_\star}_{\eqqcolon \mbf{b}^\top}\biggr\|_2^2.
    \end{align*}

    Since, allignment maximizes this expression as discussed in first point, we have:
        % We first derive the leading eigenvector of the Hessian, denoted by $\Delta_1$. This makes repeated use of Von-Neumann trace inequality~, in that $\Delta \mbf{W}_\ell$ will have their singular vectors align.

    % To maximize $f(\cdot)$, we can find $\Delta \mbf{W}_\ell$ that maximizes each term in its expansion. Consider the Frobenius norm terms (e.g., $\|\mbf{W}_{L:\ell+1} \Delta \mbf{W}_{\ell} \mbf{W}_{\ell-1:1}\|^2_{\mathsf{F}}$). Since each $\Delta\mbf{W}_\ell$ solution is rank-$1$, it follows that each one of the matrices within the norm must also be at most rank-$1$. Then, we have
    % \begin{align*}
    %     \|\mbf{W}_{L:\ell+1} \Delta_1 \mbf{W}_{\ell} \mbf{W}_{\ell-1:1}\|^2_{\mathsf{F}} = \|\mbf{W}_{L:\ell+1} \Delta_1 \mbf{W}_{\ell} \mbf{W}_{\ell-1:1}\|^2_{2} &\leq \|\mbf{W}_{L:\ell+1}\|_2^2 \cdot \|\Delta_1 \mbf{W}_{\ell}\|_2^2 \cdot \|\mbf{W}_{\ell-1:1}\|_2^2 \\
    %     &= \Delta_1 s_{\ell}^{2} \cdot \sigma_{\star, 1}^{2 - \frac{2}{L}}.
    % \end{align*}
    % To obtain this upper bound, consider the following:
    % \begin{align*}
    %     \|\mbf{W}_{L:\ell+1} \Delta_1 \mbf{W}_{\ell} \mbf{W}_{\ell-1:1}\|_2^2 = \Delta_1 s_\ell^2\cdot \biggl\|\underbrace{\mbf{V}_\star \mbf{\sigma}^{\frac{L-\ell}{L}}_\star \mbf{V}^\top_\star\mbf{u}_\ell}_{\eqqcolon \mbf{a}}\underbrace{\mbf{v}_\ell^\top \mbf{V}_\star \mbf{\sigma}^{\frac{\ell-1}{L}}_\star \mbf{V}^\top_\star}_{\eqqcolon \mbf{b}^\top}\biggr\|_2^2.
    % \end{align*}
     $\mbf{u}_\ell =\mbf{v}_\ell = \mbf{v}_{\star, 1}$ for all $\ell \in [2, L-1]$, then
    \begin{align*}
        \mbf{a} = \sigma_{\star, 1}^{\frac{L-\ell}{L}}\mbf{v}_{\star, 1} \quad \text{and} \quad \mbf{b}^\top = \sigma_{\star, 1}^{\frac{\ell - 1}{L}}\mbf{v}_{\star, 1}^\top \implies \mbf{ab}^\top = \sigma_{\star, 1}^{1 - \frac{1}{L}} \cdot \mbf{v}_{\star, 1}\mbf{v}_{\star, 1}^\top.
    \end{align*}
    The very same argument can be made for the trace terms.
    Hence, in order to maximize $f(\cdot)$, we must have
    \begin{align*}
        \mbf{v}_L &= \mbf{v}_{\star, 1}, \quad \text{and} \quad \mbf{u}_1 = \mbf{v}_{\star, 1}, \\
        \mbf{u}_\ell &= \mbf{v}_\ell = \mbf{v}_{\star, 1}, \quad \forall \ell \in [2, L-1].
    \end{align*}
    To determine $\mbf{u}_L$ and $\mbf{v}_1$, we can look at one of the trace terms:
    \begin{align*}
    \mathrm{tr}\left[\left(\Delta_1\mbf{W}_L \mbf{W}_{L-1:1} \right)^\top \left(\mbf{W}_{L:3}\Delta_1 \mbf{W}_2 \mbf{W}_{1} + \ldots +\mbf{W}_{L:2} \Delta_1 \mbf{W}_1 \right)\right] \leq \left(\frac{L-1}{L} \right)\cdot\sigma_{\star, 1}^{2 - \frac{2}{L}}.
    \end{align*}
    To reach the upper bound, we require $\mbf{u}_L = \mbf{u}_{\star, 1}$ and $\mbf{v}_1 = \mbf{v}_{\star, 1}$. Finally, as the for each index, the singular values are balanced, we will have  $\Delta_1 s_{\ell} = \frac{1}{\sqrt{L}}$ for all $\ell \in [L]$ to satisfy the constraint. Finally, we get that the leading eigenvector is
    \begin{align*}
        \Delta_1 \coloneqq \mathrm{vec}\left(\frac{1}{\sqrt{L}}\mbf{u}_1 \mbf{v}_1^\top, \frac{1}{\sqrt{L}}\mbf{v}_1 \mbf{v}_1^\top, \ldots, \frac{1}{\sqrt{L}}\mbf{v}_1 \mbf{v}_1^\top \right).
    \end{align*}
    Notice that we can also verify that $f(\Delta_1) = L\sigma_{\star, 1}^{2- \frac{2}{L}}$, which is the leading eigenvalue (or sharpness) derived in Lemma~\ref{lemma:hessian_eigvals}.  

    To derive the remaining eigenvectors, we need to find all of the vectors in which $\Delta_i^\top \Delta_j = 0$ for $i\neq j$, where
    \begin{align*}
        \Delta_i = \mathrm{vec}(\Delta_i \mbf{W}_L, \ldots \Delta_i \mbf{W}_1),
    \end{align*}
    and $f(\Delta_i) = \lambda_i$, where $\lambda_i$ is the $i$-th largest eigenvalue. By repeating the same process as above, we find that the eigenvector-eigenvalue pair as follows:
    \begin{align*}
        \Delta_1 &= \mathrm{vec}\left(\frac{1}{\sqrt{L}}\mbf{u}_1 \mbf{v}_1^\top, \frac{1}{\sqrt{L}}\mbf{v}_1 \mbf{v}_1^\top, \ldots, \frac{1}{\sqrt{L}}\mbf{v}_1 \mbf{v}_1^\top \right) , \quad\lambda_{1} =  L\sigma_{\star, 1}^{2- \frac{2}{L}} \\
        \Delta_2 &= \mathrm{vec}\left(\frac{1}{\sqrt{L}}\mbf{u}_1 \mbf{v}_2^\top, \frac{1}{\sqrt{L}}\mbf{v}_1 \mbf{v}_2^\top, \ldots, \frac{1}{\sqrt{L}}\mbf{v}_1 \mbf{v}_2^\top \right), \quad\lambda_{2} =  \left(\sum_{i=0}^{L-1} \sigma_{\star, 1}^{1-\frac{1}{L}-\frac{1}{L}i} \cdot \sigma_{\star, 2}^{\frac{1}{L}i} \right) \\
        \Delta_3 &= \mathrm{vec}\left(\frac{1}{\sqrt{L}}\mbf{u}_2 \mbf{v}_1^\top, \frac{1}{\sqrt{L}}\mbf{v}_2 \mbf{v}_1^\top, \ldots, \frac{1}{\sqrt{L}}\mbf{v}_2 \mbf{v}_1^\top \right), \quad\lambda_{3} =  \left(\sum_{i=0}^{L-1} \sigma_{\star, 1}^{1-\frac{1}{L}-\frac{1}{L}i} \cdot \sigma_{\star, 2}^{\frac{1}{L}i} \right) \\
        \quad\quad\quad&\vdots \\
         \Delta_d &= \mathrm{vec}\left(\frac{1}{\sqrt{L}}\mbf{u}_2 \mbf{v}_2^\top, \frac{1}{\sqrt{L}}\mbf{v}_2 \mbf{v}_2^\top, \ldots, \frac{1}{\sqrt{L}}\mbf{v}_2 \mbf{v}_2^\top \right), \quad\lambda_{d} =  L\sigma_{\star, 2}^{2- \frac{2}{L}} \\     
        \quad\quad\quad&\vdots \\
        \Delta_{dr+r} &= \mathrm{vec}\left(\frac{1}{\sqrt{L}}\mbf{u}_d \mbf{v}_r^\top, \frac{1}{\sqrt{L}}\mbf{v}_d \mbf{v}_r^\top, \ldots, \frac{1}{\sqrt{L}}\mbf{v}_d \mbf{v}_r^\top \right),
    \end{align*}
    which gives a total of $dr + r$ eigenvectors.

    Second, equipped with the eigenvectors, let us consider the 1-D function $f_{\Delta_i}$ generated by the cross-section of the loss landscape and each eigenvector $\Delta_i$ passing the minima:
    \begin{align*}
        f_{\Delta_i}(\mu) &= \mathcal{L}(\mbf{W}_L + \mu\Delta \mbf{W}_L, \ldots, \mbf{W}_2+ \mu\Delta \mbf{W}_2, \mbf{W}_1+ \mu\Delta \mbf{W}_1), \\
        &= \mu^2\cdot \frac{1}{2} \|\Delta \mbf{W}_L \mbf{W}_{L-1:1} + \ldots + \mbf{W}_{L:3}\Delta \mbf{W}_2 \mbf{W}_{1} + \mbf{W}_{L:2} \Delta \mbf{W}_1\|^2_{\mathsf{F}}\\
        \quad&+\mu^3 \cdot \sum_{\ell=1, \ell< m}^L\mathrm{tr}\left[\left(\mbf{W}_{L:\ell+1}\Delta \mbf{W}_\ell \mbf{W}_{\ell-1:1} \right)^\top \left( \mbf{W}_{L:\ell+1} \Delta \mbf{W}_\ell \mbf{W}_{\ell-1:m+1} \Delta \mbf{W}_{m} \mbf{W}_{m-1:1} \right)\right] \\
        \quad&+\mu^4\cdot \frac{1}{2} \left\|  \left( \sum_{\ell<m} \mbf{W}_{L:\ell+1} \Delta \mbf{W}_\ell \mbf{W}_{\ell-1:m+1} \Delta \mbf{W}_{m} \mbf{W}_{m-1:1} \right) \right\|^2_{\mathsf{F}}\\
        &+ \mu^4 \cdot\sum_{\ell<m<p} ^L \mathrm{tr}\left[\left(\mbf{W}_{L:\ell+1}\Delta \mbf{W}_\ell \mbf{W}_{\ell-1:1} \right)^\top  \left(\mbf{W}_{L:\ell+1} \Delta \mbf{W}_\ell \mbf{W}_{\ell-1:m+1} \Delta \mbf{W}_{m} \mbf{W}_{m-1:p+1} \Delta \mbf{W}_{p} \mbf{W}_{p-1:1} \right)\right].
    \end{align*}
    Then, the several order derivatives of $f_{\Delta_i}(\mu)$ at $\mu = 0$ can be obtained from Taylor expansion as
    \begin{align*}
        f_{\Delta_i}^{(2)}(0) &= \|\Delta_i \mbf{W}_L \mbf{W}_{L-1:1} + \ldots + \mbf{W}_{L:3}\Delta_i \mbf{W}_2 \mbf{W}_{1} + \mbf{W}_{L:2} \Delta_i \mbf{W}_1\|^2_{\mathsf{F}} = \lambda^2_{i}\\
        f_{\Delta_i}^{(3)}(0) &= 6\sum_{\ell=1}^L\mathrm{tr}\left[\left(\mbf{W}_{L:\ell+1}\Delta_i \mbf{W}_\ell \mbf{W}_{\ell-1:1} \right)^\top \left(\mbf{W}_{L:\ell+2}\Delta_i \mbf{W}_{\ell+1} \mbf{W}_\ell\Delta_i\mbf{W}_{\ell-1} \mbf{W}_{\ell-2:1} \right)\right] \\
        & = 6 \biggl\| \sum_{\ell} \mbf{W}_{L:\ell+1}\Delta_i \mbf{W}_\ell \mbf{W}_{\ell-1:1} \biggr\|_{\mathsf{F}}\cdot \biggl\| \left( \sum_{\ell<m} \mbf{W}_{L:\ell+1} \Delta \mbf{W}_\ell \mbf{W}_{\ell-1:m+1} \Delta \mbf{W}_{m} \mbf{W}_{m-1:1} \right) \biggr\|_{\mathsf{F}}\\
        & \coloneqq 6  \lambda_{i}\cdot\beta_{i} \\
        f_{\Delta_i}^{(4)}(0) &= 12\|\Delta_i \mbf{W}_L \Delta_i\mbf{W}_{L-1}\mbf{W}_{L-2:1} + \ldots + \mbf{W}_{L:4}\Delta_i \mbf{W}_3 \mbf{W}_{2}\Delta_i\mbf{W}_1 + \mbf{W}_{L:3}\Delta_i\mbf{W}_2 \Delta_i \mbf{W}_1\|^2_{\mathsf{F}} \\
        &+ 24\sum_{\ell=1}^L \mathrm{tr}\left[\left(\mbf{W}_{L:\ell+1}\Delta_i \mbf{W}_\ell \mbf{W}_{\ell-1:1} \right)^\top \left(\sum_{l<m<p} \mbf{W}_{L:\ell+1} \Delta \mbf{W}_\ell \mbf{W}_{\ell-1:m+1} \Delta \mbf{W}_{m} \mbf{W}_{m-1:p+1} \Delta \mbf{W}_{p} \mbf{W}_{p-1:1} \right)\right] \\
        &\coloneqq 12\beta^2_{i} + 24\lambda_{i}\cdot\delta_{i},
    \end{align*}
  
    % \begin{align*}
    %     3[f_{\Delta_i}^{(3)}]^2 - f_{\Delta_i}^{(2)}f_{\Delta_i}^{(4)} &= 108\beta\|\Delta_i \mbf{W}_L \mbf{W}_{L-1:1} + \ldots + \mbf{W}_{L:3}\Delta_i \mbf{W}_2 \mbf{W}_{1} + \mbf{W}_{L:2} \Delta_i \mbf{W}_1\|^2_{\mathsf{F}} \\
    %     &- 12\beta\|\Delta_i \mbf{W}_L \mbf{W}_{L-1:1} + \ldots + \mbf{W}_{L:3}\Delta_i \mbf{W}_2 \mbf{W}_{1} + \mbf{W}_{L:2} \Delta_i \mbf{W}_1\|^2_{\mathsf{F}} \\
    %     &- 24\gamma\|\Delta_i \mbf{W}_L \mbf{W}_{L-1:1} + \ldots + \mbf{W}_{L:3}\Delta_i \mbf{W}_2 \mbf{W}_{1} + \mbf{W}_{L:2} \Delta_i \mbf{W}_1\|^2_{\mathsf{F}} \\
    %     &= 96\beta\|\Delta_i \mbf{W}_L \mbf{W}_{L-1:1} + \ldots + \mbf{W}_{L:3}\Delta_i \mbf{W}_2 \mbf{W}_{1} + \mbf{W}_{L:2} \Delta_i \mbf{W}_1\|^2_{\mathsf{F}} \\
    %     &- 24\gamma\|\Delta_i \mbf{W}_L \mbf{W}_{L-1:1} + \ldots + \mbf{W}_{L:3}\Delta_i \mbf{W}_2 \mbf{W}_{1} + \mbf{W}_{L:2} \Delta_i \mbf{W}_1\|^2_{\mathsf{F}}.
    % \end{align*}

    where we defined 
    \begin{align*}
        & \lambda_{i} = \biggl\| \sum_{\ell} \mbf{W}_{L:\ell+1} \Delta_{i} \mbf{W}_\ell \mbf{W}_{\ell-1:1}  \biggr\|_{\mathsf{F}} \quad \tag{Total $L\choose 1$ terms}\\
        & \beta_{i} =\biggl\| \left( \sum_{\ell<m} \mbf{W}_{L:\ell+1} \Delta \mbf{W}_\ell \mbf{W}_{\ell-1:m+1} \Delta \mbf{W}_{m} \mbf{W}_{m-1:1} \right)\biggr\|_{\mathsf{F}} \quad \tag{Total $L\choose 2$ terms}\\
        & \delta_{i} = \biggl\| \left(\sum_{l<m<p} \mbf{W}_{L:\ell+1} \Delta \mbf{W}_\ell \mbf{W}_{\ell-1:m+1} \Delta \mbf{W}_{m} \mbf{W}_{m-1:p+1} \Delta \mbf{W}_{p} \mbf{W}_{p-1:1} \right) \biggr\|_{\mathsf{F}}, \quad \tag{Total $L\choose 3$ terms}
    \end{align*}
and used the fact that $\mathrm{tr}(\mbf{A}^\top \mbf{B}) = \| \mbf{A} \|_{\mathsf{F}}\cdot \| \mbf{B}\|_{\mathsf{F}}$ under singular vector alignment.

Then, since $\beta_{i} $ has $L\choose 2$ terms inside the sum, when the Frobenium term is expanded, it will have $\frac{{L\choose 2}\left({L\choose 2}+1\right)}{2}$ number of terms. 
Under alignment and balancedness, $\beta^{2}_{i} = \Delta s^2_{\ell} \sigma^{2-\frac{4}{L}}_{i}  \times \frac{{L\choose 2}\left({L\choose 2}+1\right)}{2}$ and $\lambda_{i} \delta_{i} =  \Delta s^2_{\ell} \sigma^{2-\frac{4}{L}}_{i}  \times {L\choose 3} L$. Thus, we have the expression
\begin{align*}
   2\beta^{2}_{i} - \lambda_{i} \delta_{i} &= \Delta s^2_{\ell} \sigma^{2-\frac{4}{L}}_{i} \left( 2 \frac{\binom{L}{2}\left(\binom{L}{2} + 1\right)}{2} -  \binom{L}{3} L \right) \\
   &= \Delta s^2_{\ell} \sigma^{2-\frac{4}{L}}_{i}  \binom{L}{3} L \times \left( \frac{3\left(\frac{L(L-1)}{2}+1\right)}{L(L-2)} -1 \right) \\
   & =  \Delta s^2_{\ell} \sigma^{2-\frac{4}{L}}_{i} \frac{2 \binom{L}{3} L }{L(L-2)} \times \left( (L-1)^2  + 5\right) > 0,\\
\end{align*}
for any depth $L>2$. Finally, the condition of stable oscillation of 1-D function is
\begin{align*}
       &  3[f_{\Delta_i}^{(3)}]^2 - f_{\Delta_i}^{(2)}f_{\Delta_i}^{(4)} =   108 \lambda^2_{i}\beta^{2}_{i} -  ( \lambda^{2}_{i})( 12\beta^{2}_{i} + 24(2\lambda_{i})(\delta_{i})) = 48 \lambda^{2}_{i} ( 2\beta^{2}_{i} - \lambda_{i} \delta_{i}  ) > 0,
\end{align*}
which we have proven to be positive for any depth $L>2$, for all the eigenvector directions corresponding to the non-zero eigenvalues. This completes the proof. 
    % Then, notice that from the first part of the proof,
    % \begin{align*}
    %     \|\Delta_i \mbf{W}_L \mbf{W}_{L-1:1} + \ldots + \mbf{W}_{L:3}\Delta_i \mbf{W}_2 \mbf{W}_{1} + \mbf{W}_{L:2} \Delta_i \mbf{W}_1\|^2_{\mathsf{F}} = 2\lambda_i > 0,
    % \end{align*}
    
\end{proof}

\begin{manualtheoreminner}
[Subspace Oscillation for Diagonal Linear Networks]
Consider an $L$-layer diagonal linear network on the loss 
\begin{align}
\label{eqn:diag_lin_loss}
        \mathcal{L}\left(\{\mbf{s}_\ell\}_{\ell=1}^L \right) \coloneqq \frac{1}{2} \|\mbf{s}_1 \odot \ldots \odot \mbf{s}_{L} - \mbf{s}_{\star}\|_2^2, 
 \end{align}
where $\mbf{s}_\star \in \mbb{R}^{d}$ be an $r$-sparse vector with ordered coordinates such that $s_{\star,1} >\ldots>s_{\star,d}$ and define $S_p \coloneqq L s_{\star,p}^{2-\frac{2}{L}}$ and $\alpha' \coloneqq \left( \log\left( \frac{2\sqrt{2}}{\eta S_1} \right) \cdot 2 s_{\star, 1}^{\frac{4}{L}} \right)^{\frac{1}{4}}$.
For any $p < r-1$ and $\alpha < \alpha'$, suppose we run GD on Equation~(\ref{eqn:diag_lin_loss}) with learning rate $\eta = \frac{2}{K}$, where $S_{p}\geq K> S_{p+1}$ with initialization 
$\mbf{s}_\ell = \alpha  \mbf{1}_d$ for all $\ell \in [L-1]$ and $\mbf{s}_{L}=\mbf{0}_d$. Then, under strict balancing, the top-$p$ coordinates of $\mbf{s}_\ell$ oscillate within a $2$-period fixed orbit around the minima in the form
 \begin{align*}
     s_{\ell, i}(t) = \rho_{i, j}(t), \quad \forall i < p,  \, \forall \ell \in [L],
 \end{align*}
where $\rho_{i, j}(t) \in\{\rho_{i, 1}, \rho_{i, 2}\}$, $\rho_{i, 1} \in \left(0, s_{\star, i}^{1/L} \right)$ and $\rho_{i, 2} \in \left(s_{\star, i}^{1/L}, (2s_{\star, i})^{1/L} \right)$ are two real roots of the polynomial $h(\rho)=0$:
\begin{align*}
    h(\rho) = \rho^L\cdot \frac{1+\left(1 + \eta L(s_{\star,i}  - \rho^L)\cdot \rho^{L-2} \right)^{2L-1}}{1+\left(1 + \eta L(s_{\star,i}  - \rho^L)\cdot \rho^{L-2} \right)^{L-1}}- s_{\star,i}.
\end{align*}
\label{diag-osc}
\end{manualtheoreminner}

\begin{proof}
This proof essentially mimics that of the DLN proof from Theorem~\ref{thm:align_thm}, in that we will
    \begin{enumerate}[label=(\roman*)]
        \item Compute the eigenvalues and eigenvectors of the flattened training loss Hessian of the diagonal linear network at convergence under the balancing assumption.
        \item Show that in 1D cross-section of the eigenvector, the stable condition oscillation $3[f_{\Delta_i}^{(3)}]^2 - f_{\Delta_i}^{(2)}f_{\Delta_i}^{(4)} > 0$ is satisfied, where $f_{\Delta_i}$ denotes the 1D cross-section function at the $i$-th eigenvector direction.
    \end{enumerate}
With a slight abuse in notation, let $\mbf{s} \coloneqq \{\mbf{s}_\ell\}_{\ell=1}^L$.
Let us first derive the Hessian at convergence by considering each block of the flattened Hessian matrix denoted by $\mbf{H}_{m, \ell}$:
   \begin{alignat}{2}
        &\mbf{H}_{\ell,\ell} = \begin{bmatrix}
        \prod_{k\neq \ell} s_{k, 1} & & \\
        & \ddots & \\
        & & \prod_{k\neq \ell} s_{k, d}
    \end{bmatrix} \quad\quad &\text{if } m = \ell  \\
    &\mbf{H}_{m,\ell} = \begin{bmatrix}
        \gamma_1 & & \\
        & \ddots & \\
        & & \gamma_d
    \end{bmatrix} \quad\quad &\text{if } m \neq \ell,
    \end{alignat}
    where 
    \begin{align*}
        \gamma_i \coloneqq \left(\prod_{k \neq l} s_{k, i} \right)\left(\prod_{k \neq m} s_{k, i}\right) + \left(\prod_k s_{k, i} - s_{\star, i} \right) \left(\prod_{k \neq l, k \neq m} s_{k, i} \right).
    \end{align*}
    Then, under Lemma~\ref{lemma:balancing}, at convergence (i.e. the gradient is zero), we have
    \begin{align*}
        \left(\prod_k s_{k, i} - s_{\star, i} \right) = 0 \implies s_{k, i} = s_{\star, i}^{\frac{1}{L}},
    \end{align*}
    which means that at convergence, the Hessian is given by 
    \begin{align*}
        \mbf{H} = 
        \begin{bmatrix}
            \mbf{A} & \hdots & \mbf{A} & \mbf{A} \\
            \vdots & \ddots & \vdots & \vdots \\
            \mbf{A} & \hdots & \mbf{A} & \mbf{A} \\
            \mbf{A} & \hdots & \mbf{A} & \mbf{B}
        \end{bmatrix} \in \mbb{R}^{dL \times dL},
    \end{align*}
    where 
    \begin{align*}
        \mbf{A} \coloneqq
        \begin{bmatrix}
            s_{\star, 1}^{2 - \frac{2}{L}} & & &\\
            & \ddots &  & \\
            & & s_{\star, r}^{2 - \frac{2}{L}} & \\
            & & & \mbf{0}_{d-r}
        \end{bmatrix} \in \mbb{R}^{d\times d}, \quad\quad
        \mbf{B} \coloneqq
        \begin{bmatrix}
            s_{\star, 1}^{2 - \frac{2}{L}} & & &\\
            & \ddots &  & \\
            & & s_{\star, r}^{2 - \frac{2}{L}} & \\
            & & & \alpha^{2(L-1)}\cdot\mbf{I}_{d-r}
        \end{bmatrix} \in \mbb{R}^{d\times d}.
    \end{align*}
    To compute the eigenvalues of $\mbf{H}$, we can block diagonalize $\mbf{H}$ into the form $\mbf{C} = \mbf{PHP}^{\top}$, where $\mbf{P}$ is a permutation matrix and 
    \begin{align*}
        \mbf{C} = 
        \begin{bmatrix}
            \mbf{C}_{1} & & \\
            & \ddots & \\
            &&\mbf{C}_d
        \end{bmatrix} \in \mbb{R}^{dL \times dL},
    \end{align*}
    where each $(i,j)$-th entry of $\mbf{C}_k \in \mbb{R}^{L \times L}$ is the $k$-th diagonal element of $\mbf{H}_{i, j}$. Then, since $\mbf{C}$ is a block diagonal matrix, its eigenvalues are the union of each of the eigenvalues of its blocks. Then, notice that
    \begin{align*}
        \mbf{C}_j = s_{\star, k}^{2- \frac{2}{L}} \cdot \mbf{1}_L\mbf{1}_L^{\top}, \,\,\forall j \in [r] \quad\quad
        \mbf{C}_k = 
        \begin{bmatrix}
            0 & \hdots & 0 & \alpha^{2(L-1)} \\
            \vdots & \ddots & \vdots & \vdots \\
            0 & \hdots & 0 & \alpha^{2(L-1)} \\
            \alpha^{2(L-1)} & \hdots & \alpha^{2(L-1)} & \alpha^{2(L-1)}
        \end{bmatrix}, \,\,
        \forall k \in [r+1, d].
    \end{align*}
    Hence, the eigenvalues of $\mbf{C}$ (and the eigenvalues of $\mbf{H}$) are given by 
    \begin{align*}
        \lambda_{\mbf{H}} = \biggl\{Ls_{\star, i}^{2 - \frac{2}{L}}, \underbrace{0}_{\text{multiplicity } L-1}\biggr\}_{i=1}^r \, \bigcup \,\, \biggl\{\underbrace{\frac{-\alpha^{2(L-1)} \pm \sqrt{(4L-3)\cdot \alpha^{4(L-1)^2}}}{-2}}_{\text{multiplicity } d-r}, \underbrace{0}_{\text{multiplicity } (d-r)(L-2)}\biggr\},
    \end{align*}
    which can be computed using co-factor expansion. For the eigenvectors, notice that we can write
    \begin{align*}
        \mbf{Cv} = \mbf{PHP}^\top\mbf{v} = \lambda\mbf{v} \implies \mbf{HP}^\top \mbf{v} = \lambda \mbf{P}^\top \mbf{v}.
    \end{align*}
    Hence, we can find the eigenvectors of the block diagonal matrix $\mbf{C}$, and left multiply them by $\mbf{P}^\top$ to obtain the eigenvectors of the Hessian $\mbf{H}$. This yields the eigenvector and eigenvalue pairs
\begin{alignat}{2}
    \Delta_1 &= \mbf{P}^\top\mathrm{vec}\left( \frac{1}{\sqrt{L}} \mathbf{1}_{L}, \mathbf{0}, \dots, \mathbf{0} \right), \quad &&\lambda_{1} = L s_{\star,1}^{2 - \frac{2}{L}} \\
    \Delta_2 &= \mbf{P}^\top\mathrm{vec}\left( \mathbf{0}, \frac{1}{\sqrt{L}} \mathbf{1}_{L}, \dots, \mathbf{0} \right), \quad &&\lambda_{2} = L s_{\star,2}^{2 - \frac{2}{L}} \\
    \quad\quad\quad&\vdots \quad &&\vdots\\
    \Delta_r &= \mbf{P}^\top\mathrm{vec}\left( \mathbf{0}, \dots, \frac{1}{\sqrt{L}} \mathbf{1}_{L}, \dots, \mathbf{0} \right), \quad &&\lambda_{r} = L s_{\star,r}^{2 - \frac{2}{L}} \\
    \quad\quad\quad&\vdots \quad &&\vdots\\
    \Delta_{r+j} &= \mbf{P}^\top\mathrm{vec}\left( \mathbf{0}, \dots, \mathbf{e}_{r+j}, \dots, \mathbf{0} \right) , \quad &&\lambda_{r+j} = \frac{-\alpha^{2(L-1)} \pm \sqrt{(4L-3)\cdot \alpha^{4(L-1)^2}}}{-2},
\end{alignat}
where $\mbf{e}_i$ is an $i$-th elementary basis vector.

Then, in each 1-D eigenvector direction, we can analyze the loss and verify if it satisfies the stability condition. Notice that we can consider the scalar loss 
\begin{align*}
    \mathcal{L}_i(\mbf{s}) = \frac{1}{2}(s_{1, i} \odot \ldots \odot s_{L, i} - s_{\star, i})^2 = \frac{1}{2} (s_i^L -s_{\star, i})^2. \tag{By Lemma~\ref{lemma:balancing}}
\end{align*}
Using Corollary 5 by \cite{chen2023edge} or restated Lemma~\ref{lemma:chen-bruna} on the 1D scalar function, this 1D loss is amenable to stable oscillation when learning rate $\eta >\frac{2}{\lambda_{i}} $. Finally, to prove the uniqueness and existence of two period orbit fixed point for $ \eta >\frac{2}{\lambda_{i}}$, we show that the polynomial obtained by solving two step fixed point has a real root. This is the same loss we analyzed in Theorem \ref{thm:stable_oscillations}, where we showed that the oscillations are real roots of the polynomial
\begin{align*}
    \sigma_{\star, 1} = \rho^L\frac{1+z^{2L-1}}{1+z^{L-1}}, \quad \text{where  } \, z \coloneqq \left(1 + \eta L(\sigma_{\star, 1} - \rho^L)\cdot \rho^{L-2} \right).
\end{align*}
and 
$\rho_1 \in \left(0, \sigma_{\star, 1}^{1/L}\right)$ and $\rho_2 \in \left(\sigma_{\star, 1}^{1/L}, (2\sigma_{\star, 1})^{1/L}\right)$ are the two real roots of the polynomial which exists and are unique.
Hence, whenever the learning rate $\eta$ lies between $[2/\lambda_p,2/\lambda_{p+1}]$, we will have oscillations in all of the $p$ eigenvector directions. This completes the proof. 

\end{proof}

\begin{manuallemmainner}
[\cite{chen2023edge}]
\label{lemma:chen-bruna}
Consider any 1-D differentiable function $f(x)$ around a local minima $\bar{x}$, satisfying (i) $f^{(3)}(\bar{x}) \neq 0$, and (ii) $3[f^{(3)}]^2 - f'' f^{(4)} > 0$ at $\bar{x}$. Then, there exists $\epsilon$ with sufficiently small $|\epsilon|$ and $\epsilon \cdot f^{(3)} > 0$ such that: for any point $x_0$ between $\bar{x}$ and $\bar{x} - \epsilon$, there exists a learning rate $\eta$ such that $F_{\eta}^2(x_0) = x_0$, and
\end{manuallemmainner}

\[
\frac{2}{f''(\bar{x})} < \eta < \frac{2}{f''(\bar{x}) - \epsilon \cdot f^{(3)}(\bar{x})}.
\]

\clearpage

\begin{manualpropositioninner}
    
\label{prop:one_zero_svs_set}
    Let $\mbf{M}_\star = \mbf{U}_\star\mbf{\Sigma}_\star \mbf{V}_\star^\top$ denote the SVD of the target matrix. The initialization in Equation~(\ref{eqn:init}) is a member of the singular vector stationary set in Proposition~\ref{prop:svs_set}, where $\mbf{Q}_L = \ldots = \mbf{Q}_2 = \mbf{V}_\star$.
\end{manualpropositioninner}
\begin{proof}
Recall that the initialization is given by
    \begin{align*}
        \mbf{W}_L(0) = 0 \quad \text{and} \quad \mbf{W}_\ell(0) = \alpha\mbf{I}_d \quad \forall \ell \in [L-1].
    \end{align*}
    We will show that under this initialization, each weight matrix admits the following decomposition for all $t \geq 1$:
    \begin{align}
        \mbf{W}_L(t) = \mbf{U}_\star \begin{bmatrix}
            \widetilde{\mbf{\Sigma}}_L(t) & \mbf{0} \\
            \mbf{0} & \mbf{0}
        \end{bmatrix} \mbf{V}_\star^\top,
        \quad\quad
        \mbf{W}_{\ell}(t) = \mbf{V}_\star \begin{bmatrix}
            \widetilde{\mbf{\Sigma}}(t) & \mbf{0} \\
            \mbf{0} & \alpha\mbf{I}_{d-r}
        \end{bmatrix} \mbf{V}_\star^\top,
        \quad \forall \ell \in [L-1],
    \end{align}
where
\begin{align*}
    \widetilde{\mbf{\Sigma}}_L(t) &= \widetilde{\mbf{\Sigma}}_L(t-1) - \eta \cdot\left(\widetilde{\mbf{\Sigma}}_L(t-1) \cdot \widetilde{\mbf{\Sigma}}^{L-1}(t-1) - \mbf{\Sigma}_{\star,r}\right)\cdot \widetilde{\mbf{\Sigma}}^{L-1}(t-1) \\
    \widetilde{\mbf{\Sigma}}(t) &= \widetilde{\mbf{\Sigma}}(t-1)\cdot  \left(\mbf{I}_r- \eta\cdot\widetilde{\mbf{\Sigma}}_L(t-1)\cdot\left(\widetilde{\mbf{\Sigma}}_L(t-1) \cdot \widetilde{\mbf{\Sigma}}^{L-1}(t-1) - \mbf{\Sigma}_{\star,r}\right)\cdot \widetilde{\mbf{\Sigma}}^{L-3}(t-1)\right),
\end{align*}
where $\widetilde{\mbf{\Sigma}}_L(t), \widetilde{\mbf{\Sigma}}(t) \in \mbb{R}^{r\times r}$ is a diagonal matrix with $\widetilde{\mbf{\Sigma}}_L(1) = \eta \alpha^{L-1}\cdot \mbf{\Sigma}_{r,\star}$ and $\widetilde{\mbf{\Sigma}}(1) = \alpha \mbf{I}_r$. 

This will prove that the singular vectors are stationary with $\mbf{\Sigma}_L = \ldots =\mbf{\Sigma}_2 = \mbf{V}_\star$. We proceed with mathematical induction. 

\paragraph{Base Case.} For the base case, we will show that the decomposition holds for each weight matrix at $t=1$. The gradient of $f(\mbf{\Theta})$ with respect to $\mbf{W}_{\ell}$ is
\begin{align*}
    \nabla_{\mbf{W}_{\ell}} f(\mbf{\Theta}) = \mbf{W}^{\top}_{L:\ell+1} \cdot \left(\mbf{W}_{L:1} - \mbf{M}_\star \right) \cdot \mbf{W}^{\top}_{\ell-1:1}. 
\end{align*}
For $\mbf{W}_L(1)$, we have
\begin{align*}
    \mbf{W}_L(1) &= \mbf{W}_L(0) - \eta \cdot \nabla_{\mbf{W}_{L}} f(\mbf{\Theta}(0)) \\
    &= \mbf{W}_L(0) - \eta \cdot \left(\mbf{W}_{L:1}(0) - \mbf{M}_\star \right) \cdot \mbf{W}^{\top}_{L-1:1}(0)\\
    &= \eta \alpha^{L-1}\mbf{\Sigma}_\star \\
    &= \mbf{U}_\star \cdot \left( \eta \alpha^{L-1} \cdot \mbf{\Sigma}_\star \right) \cdot \mbf{V}_\star^\top \\
    &= \mbf{U}_\star
    \begin{bmatrix}
        \widetilde{\mbf{\Sigma}}_L(1) & \mbf{0} \\
        \mbf{0} & \mbf{0}
    \end{bmatrix}
    \mbf{V}_\star^\top.
\end{align*}
Then, for each $\mbf{W}_{\ell}(1)$ in $\ell \in [L-1]$, we have
\begin{align*}
\mbf{W}_{\ell}(1)&= \mbf{W}_{\ell}(0) - \eta \cdot \nabla_{\mbf{W}_{\ell}}f(\mbf{\Theta}(0)) \\
&= \alpha\mbf{I}_d,
\end{align*}
where the last equality follows from the fact that $\mbf{W}_L(0) = \mbf{0}$. Finally, we have
\begin{align*}
    \mbf{W}_{\ell}(1) = \alpha \mbf{V}_\star \mbf{V}_\star^\top = \mbf{V}_\star \begin{bmatrix}
        \widetilde{\mbf{\Sigma}}(1) & \mbf{0} \\
        \mbf{0} & \alpha\mbf{I}_{d-r}
     \end{bmatrix}\mbf{V}_\star^\top, \quad \forall \ell \in [L-1].
\end{align*}

\paragraph{Inductive Step.} By the inductive hypothesis, suppose that the decomposition holds. Then, notice that we can simplify the end-to-end weight matrix to
\begin{align*}
    \mbf{W}_{L:1}(t) = \mbf{U}_\star
    \begin{bmatrix}
        \widetilde{\mbf{\Sigma}}_L(t) \cdot \widetilde{\mbf{\Sigma}}^{L-1}(t) & \mbf{0} \\
        \mbf{0} & \mbf{0}
    \end{bmatrix}
    \mbf{V}_\star^\top,
\end{align*}
for which we can simplify the gradients to
\begin{align*}
    \nabla_{\mbf{W}_{L}} f(\mbf{\Theta}(t)) &= \left(\mbf{U}_\star \begin{bmatrix}
        \widetilde{\mbf{\Sigma}}_L(t) \cdot \widetilde{\mbf{\Sigma}}^{L-1}(t) - \mbf{\Sigma}_{\star,r} & \mbf{0} \\
        \mbf{0} & \mbf{0}
    \end{bmatrix} \mbf{V}_\star^\top\right) \cdot  \mbf{V}_\star \begin{bmatrix}
        \widetilde{\mbf{\Sigma}}^{L-1}(t) & \mbf{0} \\
        \mbf{0} & \mbf{0}
    \end{bmatrix}\mbf{V}_\star^\top \\
    &= \mbf{U}_\star \begin{bmatrix}
        \left(\widetilde{\mbf{\Sigma}}_L(t) \cdot \widetilde{\mbf{\Sigma}}^{L-1}(t) - \mbf{\Sigma}_{\star,r}\right)\cdot \widetilde{\mbf{\Sigma}}^{L-1}(t) & \mbf{0} \\
        \mbf{0} & \mbf{0}
    \end{bmatrix} \mbf{V}_\star^\top,
\end{align*}
for the last layer matrix, and similarly,
\begin{align*}
     \nabla_{\mbf{W}_{\ell}} f(\mbf{\Theta}(t)) &= \mbf{V}_\star \begin{bmatrix}
        \widetilde{\mbf{\Sigma}}_L(t)\cdot\left(\widetilde{\mbf{\Sigma}}_L(t) \cdot \widetilde{\mbf{\Sigma}}^{L-1}(t) - \mbf{\Sigma}_{\star,r}\right)\cdot \widetilde{\mbf{\Sigma}}^{L-2}(t)  & \mbf{0} \\
        \mbf{0} & \mbf{0}
    \end{bmatrix} \mbf{V}_\star^\top, \quad \ell \in [L-1],
\end{align*}
for all other layer matrices. Thus, for the next GD iteration, we have
\begin{align*}
    \mbf{W}_L(t+1) &= \mbf{W}_{L}(t) - \eta \cdot \nabla_{\mbf{W}_L}(\mbf{\Theta}(t)) \\
    &= \mbf{U}_\star \begin{bmatrix}
        \widetilde{\mbf{\Sigma}}_L(t) - \eta \cdot\left(\widetilde{\mbf{\Sigma}}_L(t) \cdot \widetilde{\mbf{\Sigma}}^{L-1}(t) - \mbf{\Sigma}_{\star,r}\right)\cdot \widetilde{\mbf{\Sigma}}^{L-1}(t) & \mbf{0} \\
        \mbf{0} & \mbf{0}
    \end{bmatrix} \mbf{V}_\star^\top \\
    &= \mbf{U}_\star \begin{bmatrix}
        \widetilde{\mbf{\Sigma}}_L(t+1) & \mbf{0} \\
        \mbf{0} & \mbf{0}
    \end{bmatrix} \mbf{V}_\star^\top.
\end{align*}
Similarly, we have
\begin{align*}
    \mbf{W}_\ell(t+1) &= \mbf{W}_{\ell}(t) - \eta \cdot \nabla_{\mbf{W}_\ell}(\mbf{\Theta}(t)) \\
    &= \mbf{V}_\star \begin{bmatrix}
        \widetilde{\mbf{\Sigma}}(t) - \eta\cdot\widetilde{\mbf{\Sigma}}_L(t)\cdot\left(\widetilde{\mbf{\Sigma}}_L(t) \cdot \widetilde{\mbf{\Sigma}}^{L-1}(t) - \mbf{\Sigma}_{\star,r}\right)\cdot \widetilde{\mbf{\Sigma}}^{L-2}(t)  & \mbf{0} \\
        \mbf{0} & \alpha \mbf{I}_{d-r}
    \end{bmatrix} \mbf{V}_\star^\top \\
     &= \mbf{V}_\star \begin{bmatrix}
        \widetilde{\mbf{\Sigma}}(t)\cdot  \left(\mbf{I}_r- \eta\cdot\widetilde{\mbf{\Sigma}}_L(t)\cdot\left(\widetilde{\mbf{\Sigma}}_L(t) \cdot \widetilde{\mbf{\Sigma}}^{L-1}(t) - \mbf{\Sigma}_{\star,r}\right)\cdot \widetilde{\mbf{\Sigma}}^{L-3}(t)\right)  & \mbf{0} \\
        \mbf{0} & \alpha \mbf{I}_{d-r}
    \end{bmatrix} \mbf{V}_\star^\top \\
    &= \mbf{V}_\star \begin{bmatrix}
        \widetilde{\mbf{\Sigma}}(t+1) & \mbf{0} \\
        \mbf{0} & \alpha \mbf{I}_{d-r}
    \end{bmatrix} \mbf{V}_\star^\top,
\end{align*}
for all $\ell \in [L-1]$. This completes the proof.
\end{proof}

\begin{manualpropositioninner}
\label{prop:balanced_svs_set}

 Let $\mbf{M}_\star = \mbf{V}_\star\mbf{\Sigma}_\star \mbf{V}_\star^\top \in \mbb{R}^{d\times d}$ denote the SVD of the target matrix. The balanced initialization in Equation~(\ref{eqn:balanced_init}) is a member of the singular vector stationary set in Proposition~\ref{prop:svs_set}, where  $\mbf{U}_L = \mbf{Q}_L = \ldots = \mbf{Q}_2 = \mbf{V}_1 = \mbf{V}_\star$.
 
\end{manualpropositioninner}

\begin{proof}
    
Using mathematical induction, we will show that with the balanced initialization in Equation~(\ref{eqn:balanced_init}), each weight matrix admits a decomposition of the form
\begin{align}
    \mbf{W}_\ell(t) = \mbf{V}_\star \mbf{\Sigma}_\ell(t) \mbf{V}_\star^\top,
\end{align}
which implies that the singular vectors are stationary for all $t$ such that $\mbf{U}_L = \mbf{Q}_L = \ldots = \mbf{Q}_2 = \mbf{V}_1 = \mbf{V}_\star$.

\paragraph{Base Case.} Consider the weights at iteration $t=0$. By the initialization scheme, we can write each weight matrix as
\begin{align*}
    \mbf{W}_\ell(0) = \alpha \mbf{I}_d \implies  \mbf{W}_\ell(0) = \alpha \mbf{V}_\star \mbf{V}_\star^\top,
\end{align*}
which implies that $\mbf{W}_\ell(0) = \mbf{V}_\star \mbf{\Sigma}_\ell(0)\mbf{V}_\star^\top$ with $\mbf{\Sigma}_\ell(0) = \alpha \mbf{I}_d$.

\paragraph{Inductive Step.} By the inductive hypothesis, assume that the decomposition holds for all $t \geq 0$. We will show that it holds for all iterations $t+1$. Recall that the gradient of $f(\mbf{\Theta})$ with respect to $\mbf{W}_{\ell}$ is
\begin{align*}
    \nabla_{\mbf{W}_{\ell}} f(\mbf{\Theta}) = \mbf{W}^{\top}_{L:\ell+1} \cdot \left(\mbf{W}_{L:1} - \mbf{M}_\star \right) \cdot \mbf{W}^{\top}_{\ell-1:1}. 
\end{align*}
Then, for $\mbf{W}_\ell(t+1)$, we have
\begin{align*}
    \mbf{W}_\ell(t+1) &= \mbf{W}_\ell(t) - \eta \cdot \nabla_{\mbf{W}_{L}} f(\mbf{\Theta}(t)) \\
    &=  \mbf{V}_\star \mbf{\Sigma}_\ell(t)\mbf{V}_\star^\top - \eta \mbf{W}^\top_{L:\ell+1}(t) \cdot \left(\mbf{W}_{L:1}(t) - \mbf{M}_\star \right) \cdot \mbf{W}^{\top}_{\ell-1:1}(t)\\
    &=  \mbf{V}_\star \mbf{\Sigma}_\ell(t)\mbf{V}_\star^\top - \eta \mbf{V}_\star\cdot \left(  \mbf{\Sigma}^{L-\ell}_\ell(t)\cdot \left(\mbf{\Sigma}_\ell^{L}(t) - \mbf{\Sigma}_\star \right)\cdot \mbf{\Sigma}_\ell^{\ell-1}(t) \right) \cdot\mbf{V}^{\top}_{\star}\\
    &=  \mbf{V}_\star\cdot \left(\mbf{\Sigma}_\ell(t) - \eta\cdot  \mbf{\Sigma}^{L-\ell}_\ell(t)\cdot \left(\mbf{\Sigma}_\ell^{L}(t) - \mbf{\Sigma}_\star \right)\cdot \mbf{\Sigma}_\ell^{\ell-1}(t) \right) \cdot\mbf{V}^{\top}_{\star}\\
    &= \mbf{V}_\star
   \mbf{\Sigma}(t)
    \mbf{V}_\star^\top,
\end{align*}
where $\mbf{\Sigma}(t) = \mbf{\Sigma}_\ell(t) - \eta\cdot  \mbf{\Sigma}^{L-\ell}_\ell(t)\cdot \left(\mbf{\Sigma}_\ell^{L}(t) - \mbf{\Sigma}_\star \right)\cdot \mbf{\Sigma}_\ell^{\ell-1}(t)$. This completes the proof.
\end{proof}

\begin{figure}[h!]
    \centering
    \includegraphics[width=\linewidth]{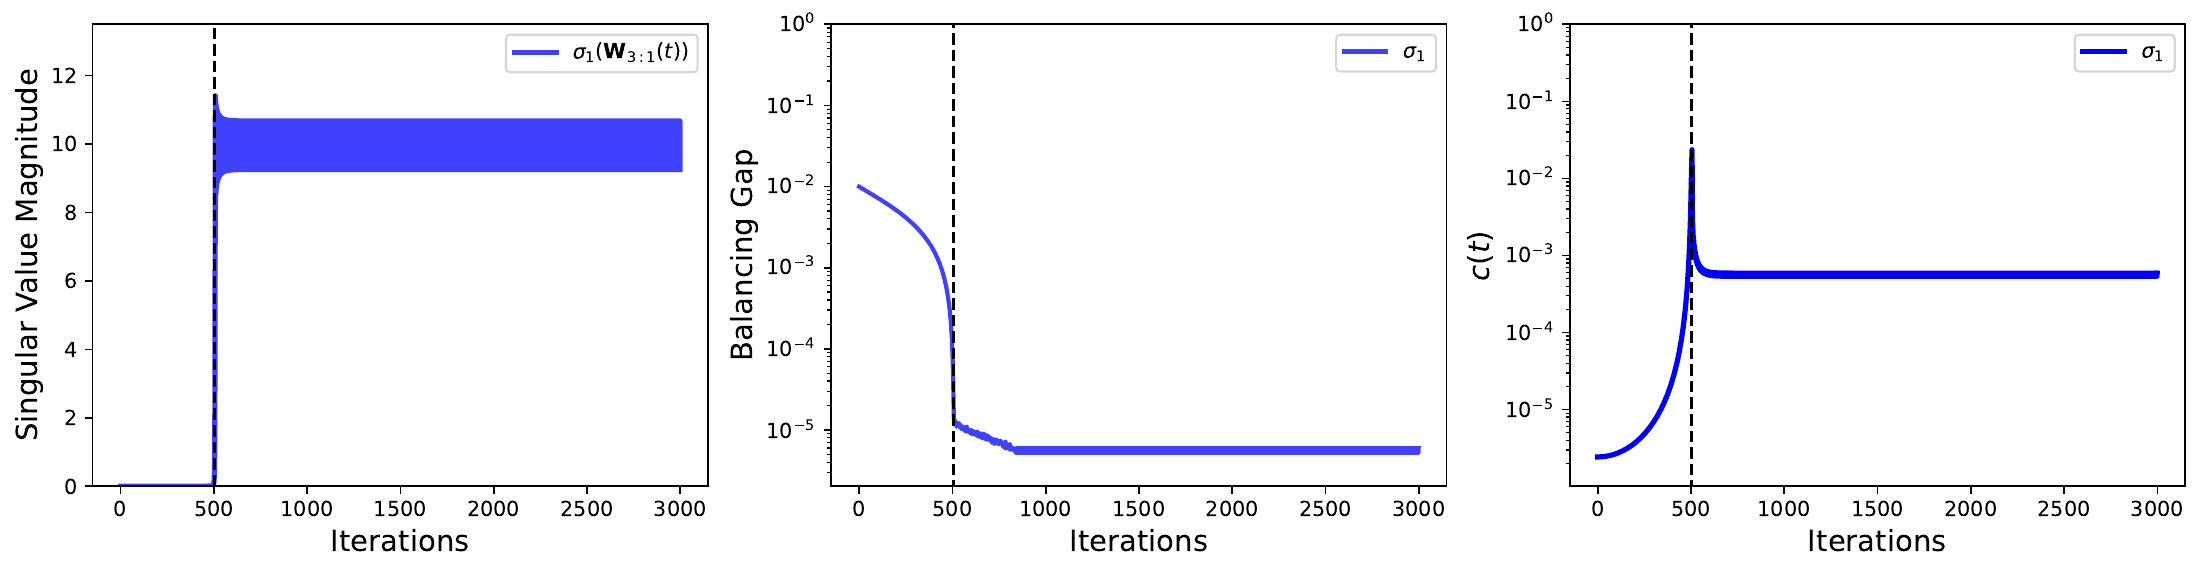}
    \caption*{The lefthand side of the dashed black line refers to 
    $\pi(t) < \sigma_{\star, 1}$ and the righthand side refers to a mixture of $\pi(t) < \sigma_{\star, 1}$ and $\pi(t) > \sigma_{\star, 1}$ due to oscillations. Left: Evolution of the first singular value of the end-to-end DLN for fitting a rank-1 target matrix. Due to small initialization, the singular value slowly increases from $\alpha$ until it oscillates around the minimum $\sigma_{\star, 1} = 10$. Middle: Evolution of the balancing gap. The balancing gap strictly decreases in the $\pi(t) < \sigma_{\star, 1}$ regime as predicted by our theory. When the oscillations occur, the balancing gap stabilizes close to 0. Right: Evolution of $c(t)$, which is the value that ensures that $0<c<1$ as long as $|1-c(t)|<c$. }
    \label{fig:enter-label}
\end{figure}
